# Supplementary material for: A Cradle-to-Gate Life Cycle Analysis of Bitcoin Mining Equipment Using Sphera LCA and ecoinvent Databases
Source: arXiv:2401.17512 ancillary file (2024-06-09)
Supplement: Supplementary file 1 [file SuppInfo-2-Foreground-modeling.pdf]

Supplementary information

# Detailed LCI model

Bitmain Antminer S9
APW3++

And a rapid analysis of the difference with Antminer S19 and APW12

# Contents

Purpose and structure, How to read this document: p. 3
Control Board: p. 7
Hashboard: p. 21
Power Supply (APW3): p. 32
Fan: p. 46
Casing: p. 48
Cables: p. 50
Assembly: p. 56
Transport: p. 58
Adaptation to the Antminer S19 Pro and the power supply APW 12: p. 60
Additional Information: p. 69
Sources: p. 79

# Purpose and structure of this document

- This document is a detailed presentation of the inventory of components realized on the Antminer S9 and the power supply APW3, supported by pictures. It provides a high level of transparency by allowing the reader to understand the reasoning used to determine the quantities and types of each electronic component in the life cycle inventory (LCI).
- This tool for understanding is a complement to the SI 1 inventory (Excel), which provides the names and quantities of each process used for implementation with the databases and allows the reproduction of our study.

Both documents are structured following the structure of the ASIC miner, with a section for each component:

- Control board: distributes the calculations between hashboards and communicates with the network.
- Hashboard (x3): used to do the parallel computations needed by the proof-of-work protocol.
- Power supply: not included in the Antminer S9, but it is required to ensure the board functionality
- Casing
- Fans
- Cables
- Transport
- Assembly

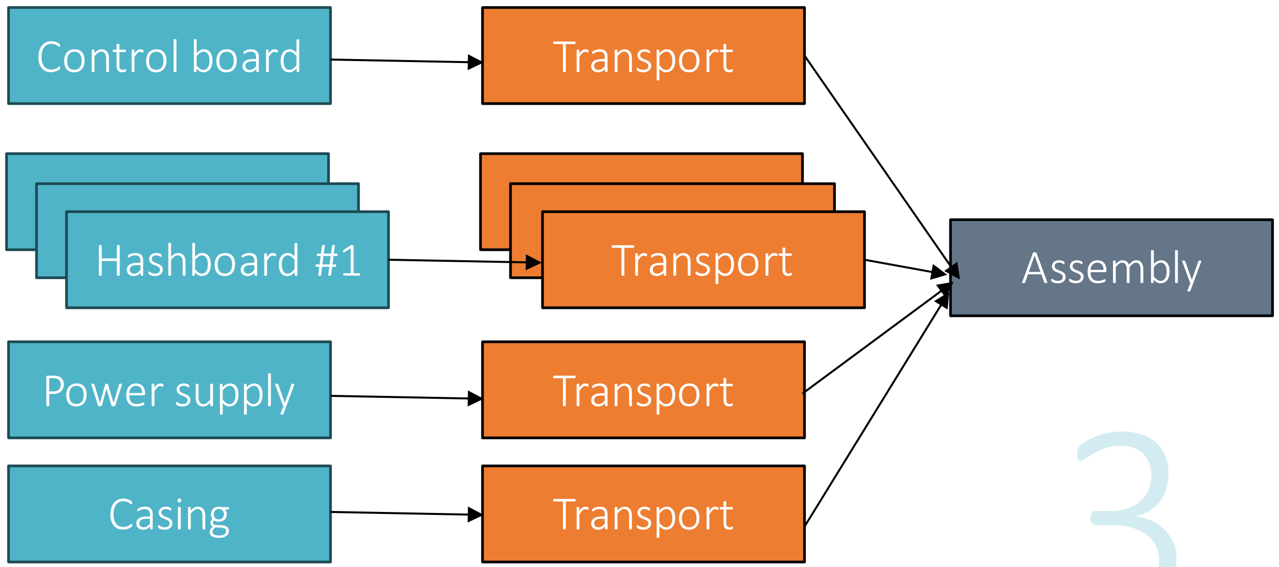

# How to read this document ? *Quantities*

1

Identifiers: they are attached with one component. It allows for several occurencies one type of component to be counted several times. In the EXCEL document, we use the same reference for easy matching between pictures presented and additional information

x2

Number of occurrences of one component

>x22

This indicates the maximum value we are able to read on the PCB labels for the type of component studied.

*Example: "D22" is the higher label with "D" we can read. Then, we conclude that there are at least 22 diodes.*

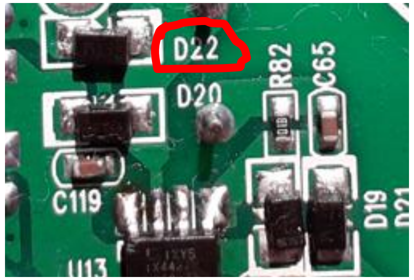


>~22

We count the maximum value we are able to read on the PCB labels for the type of component studied, but we also notice lot of empty footprints on the PCB, indicating that the maximum label may be a higher than the actual number of the one type of component.

Remark: If a same component is present in different modules (e.g. in the control board and in the hashboard), another ID is attributed to this component in each module. This is because the different modules are modeled independently with databases.

# How to read this document ? *Boxes (1)*

1. Blue boxes: they indicate a well identified component:

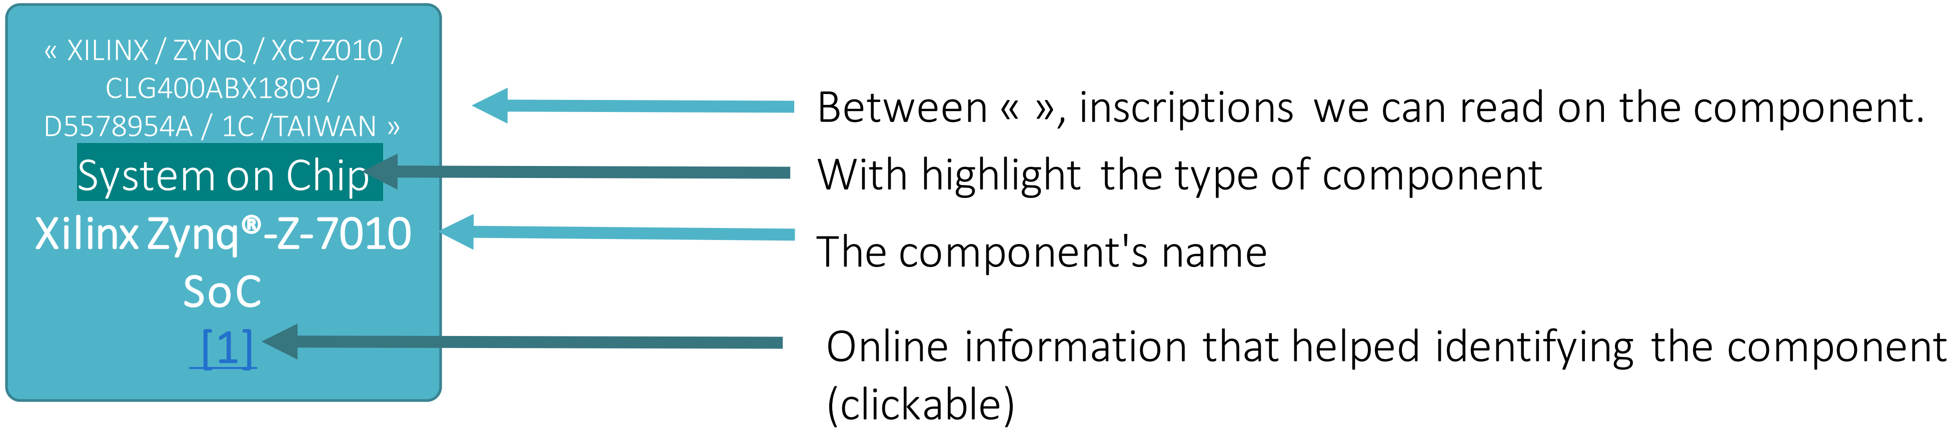

# How to read this document ? *Boxes (2)*

## 2. Green boxes: Identification with a component of the GaBi database

Inductors

Ring core coils 8, 30, 80g (without housing)

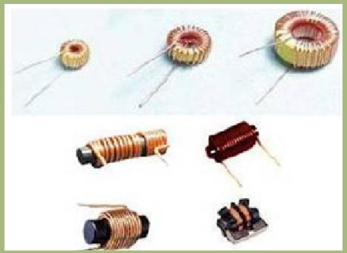

Nature of the component

Highlighted: name of the identified type of component in the database

Picture of the associated type of component in the GaBi documentation

Important: all the pictures in the green boxes are from the GaBi documentation. This pictures are available here [49] (for ICs, transistors and diodes) [50] (for resistors, capacitors, inductors, crystal oscillators, switches)

## 3. Pink boxes: Other components

24

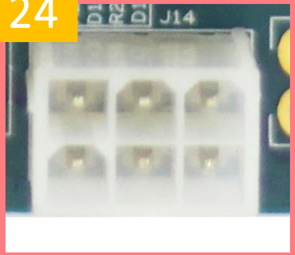


Controller PCI-e Power Connector

# Control board

The control board distributes the calculations between hashboards and communicates with the network.

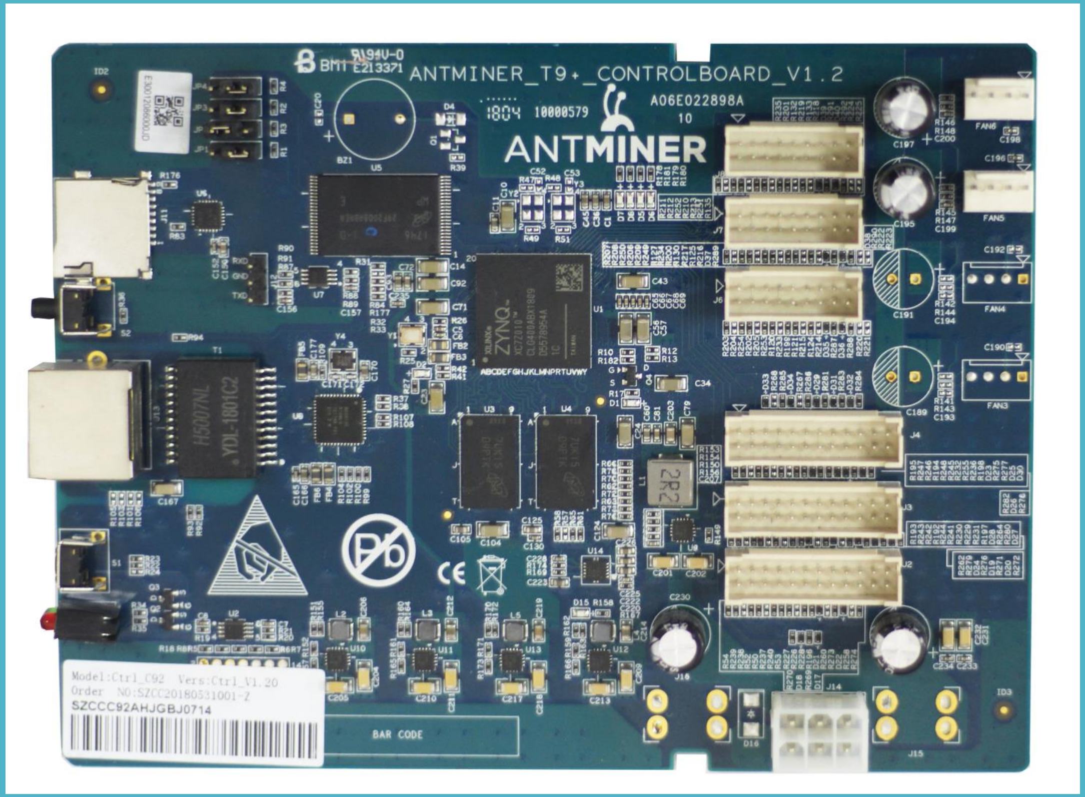

# General structure: the two sides

Remark: There are some differences between the different versions of this control board. Even if the study is mainly illustrated in this presentation with pictures of the control board v 1.2, in the majority of cases, the information collected on the version 1.0 (the version we have access to) were kept. However, the diffrences observed between the two versions are reported in the following.

Control Board V 1.0 (the one dismanteled for the study)

Upper side

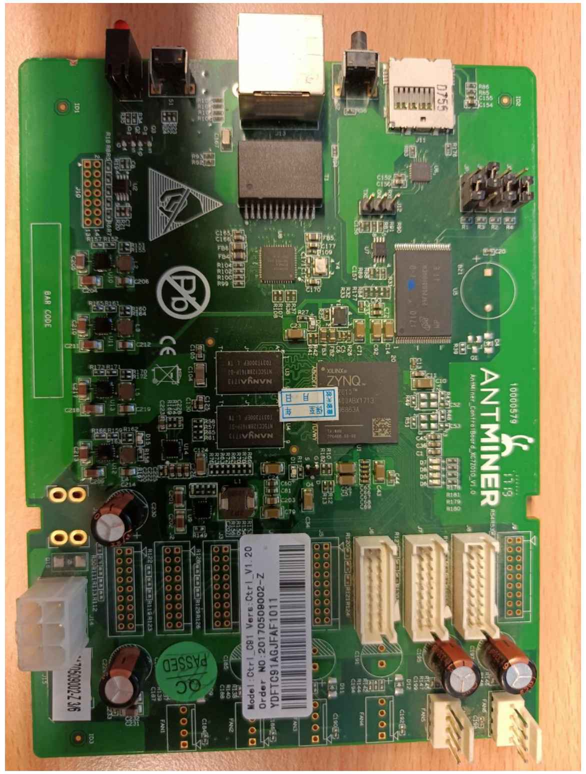


Picture from: Ludmila Courtillat--Piazza

Lower side

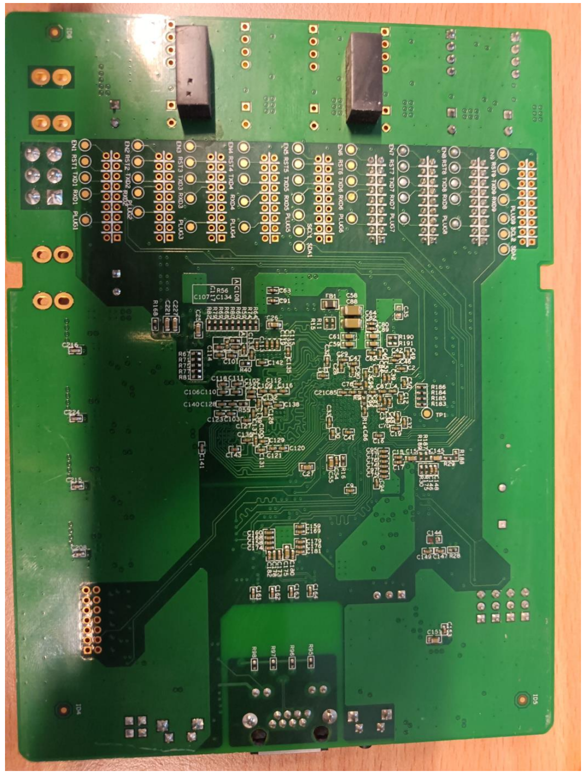

Picture from: Ludmila Courtillat--Piazza

Control Board V 1.2

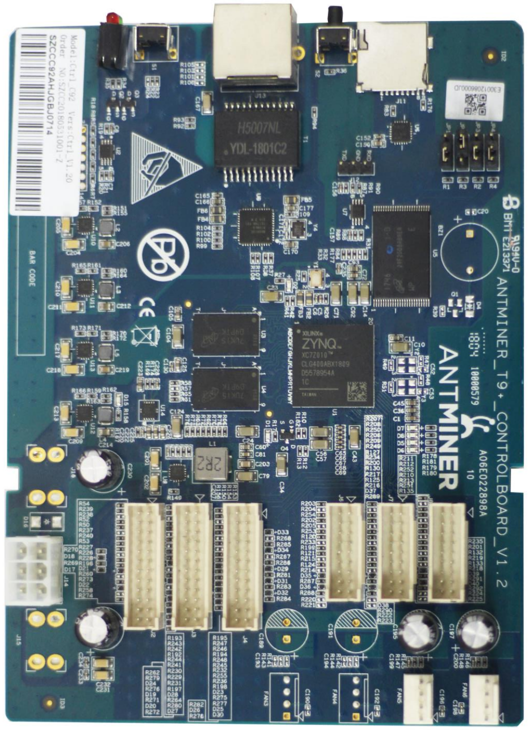


Picture from: [5]

Control Board (unidentified version)

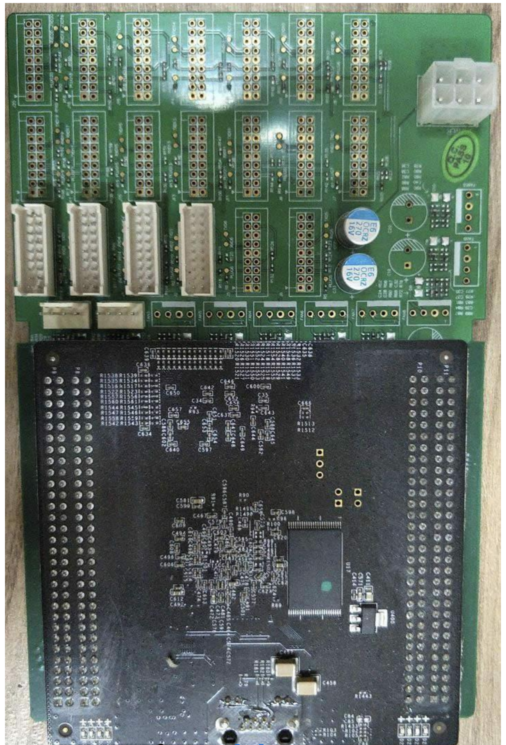

Picture from: [6]

# PCB

6 layers

The PCB were cut and observed under a microscope.

8

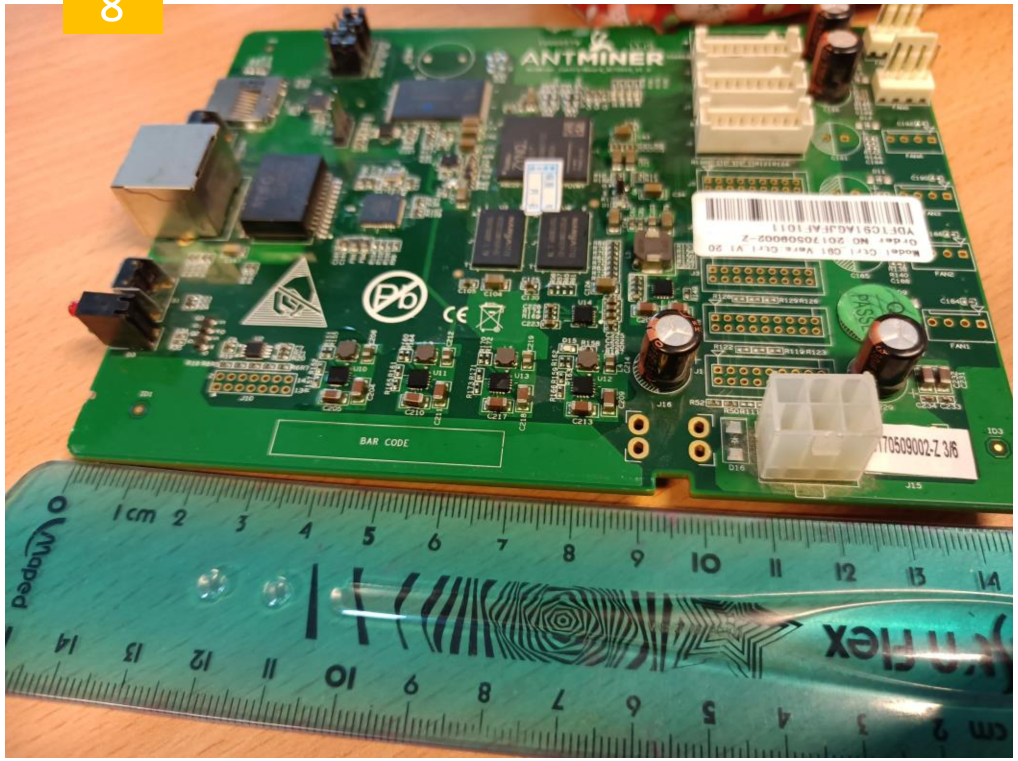


Picture from: Ludmila Courtillat--Piazza

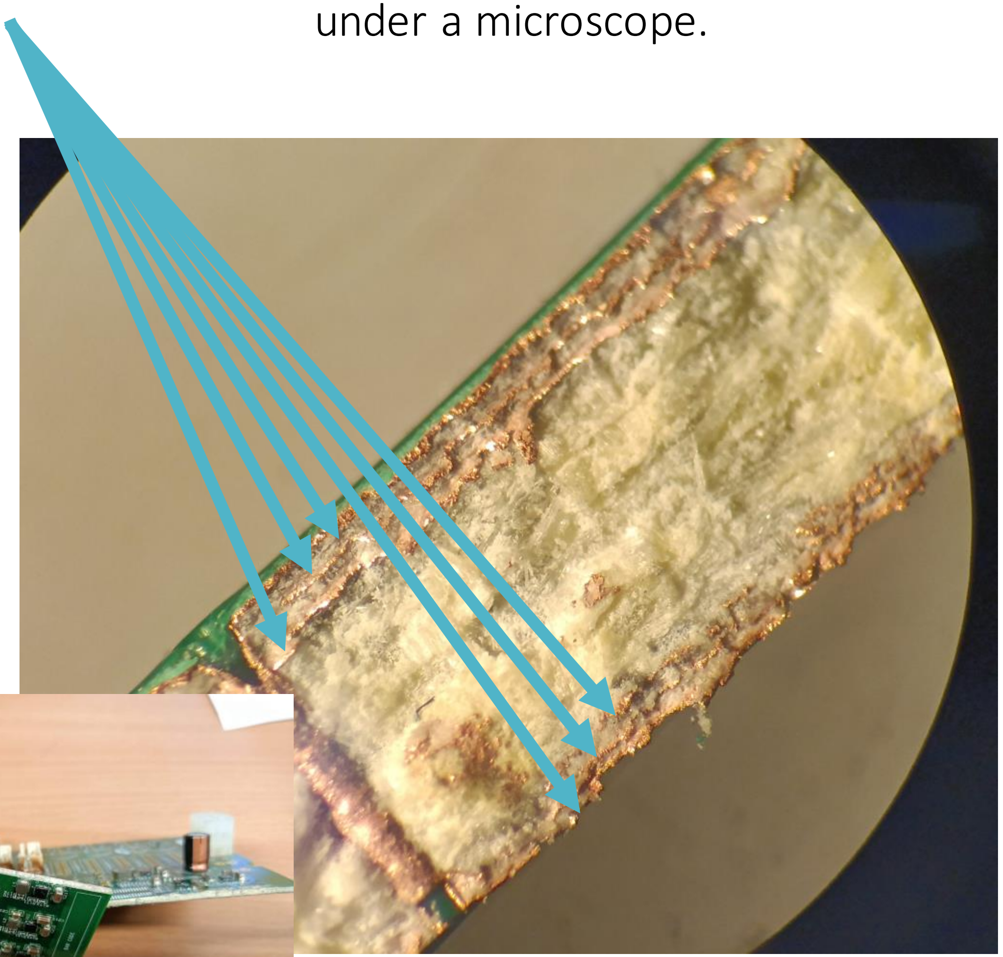

Picture from: Ludmila Courtillat--Piazza

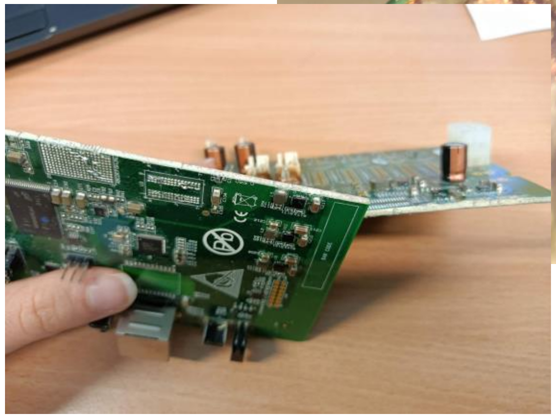

Picture from: Ludmila Courtillat--Piazza

# Control Board: ICs

Warning: this is not an IC !

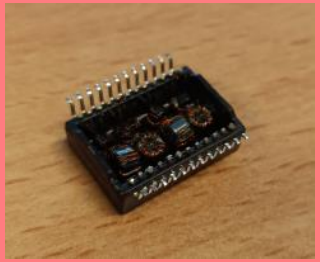

Picture from: Ludmila Courtillat--Piazza

« 7UK15
D9PTK + logo de Micron »
-> DRAM Micron
MT41K128M16JT-125:k
[3], [4]

3

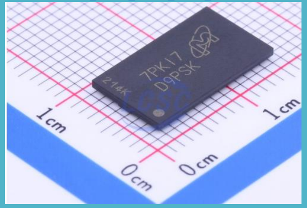

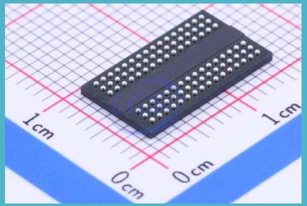

x2

« XILINX / ZYNQ / XC7Z010 / CLG400ABX1809 / D5578954A / 1C /TAIWAN »
System on Chip
Xilinx Zynq®-Z-7010 SoC

1 [1]

2

« H5007NL
YDL-1801C2 »
-> H500NL (Ethernet Transformer)
[2]

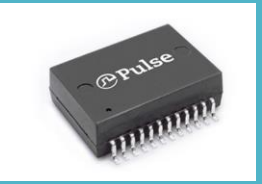


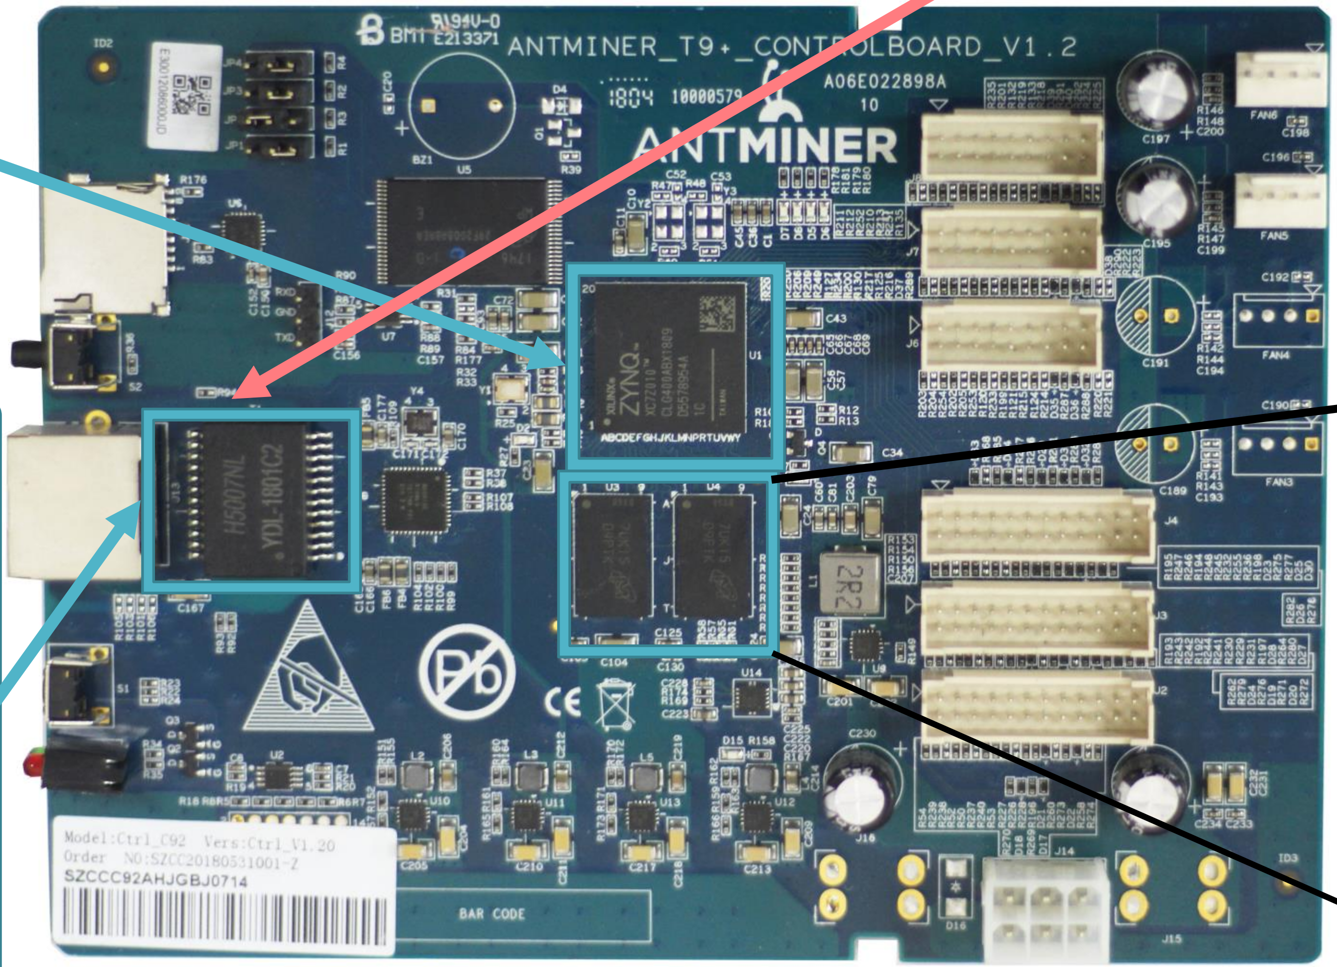


Picture from: [5]

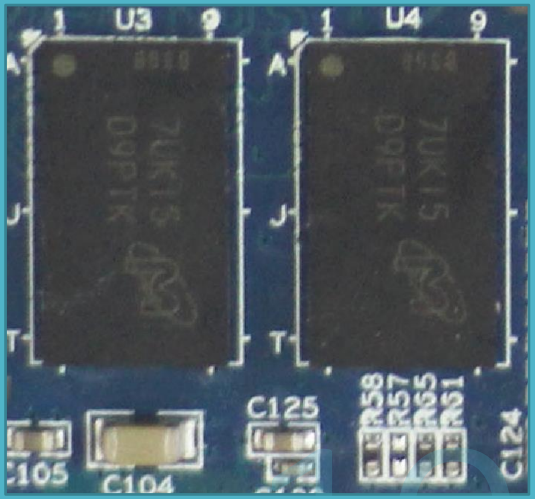


Picture from: [5]

# Control Board: ICs

« 1746 / I-D / logo micron / 29F2G08ABAEA / WP / E »

SLC NAND Flash

MT29F2G08ABAEA WP-IT:E TR

4

[7]

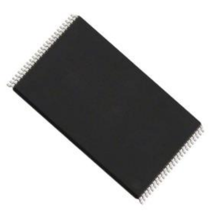

IC, SO 8-44

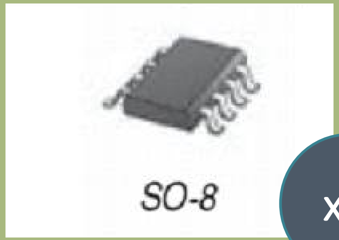


x2

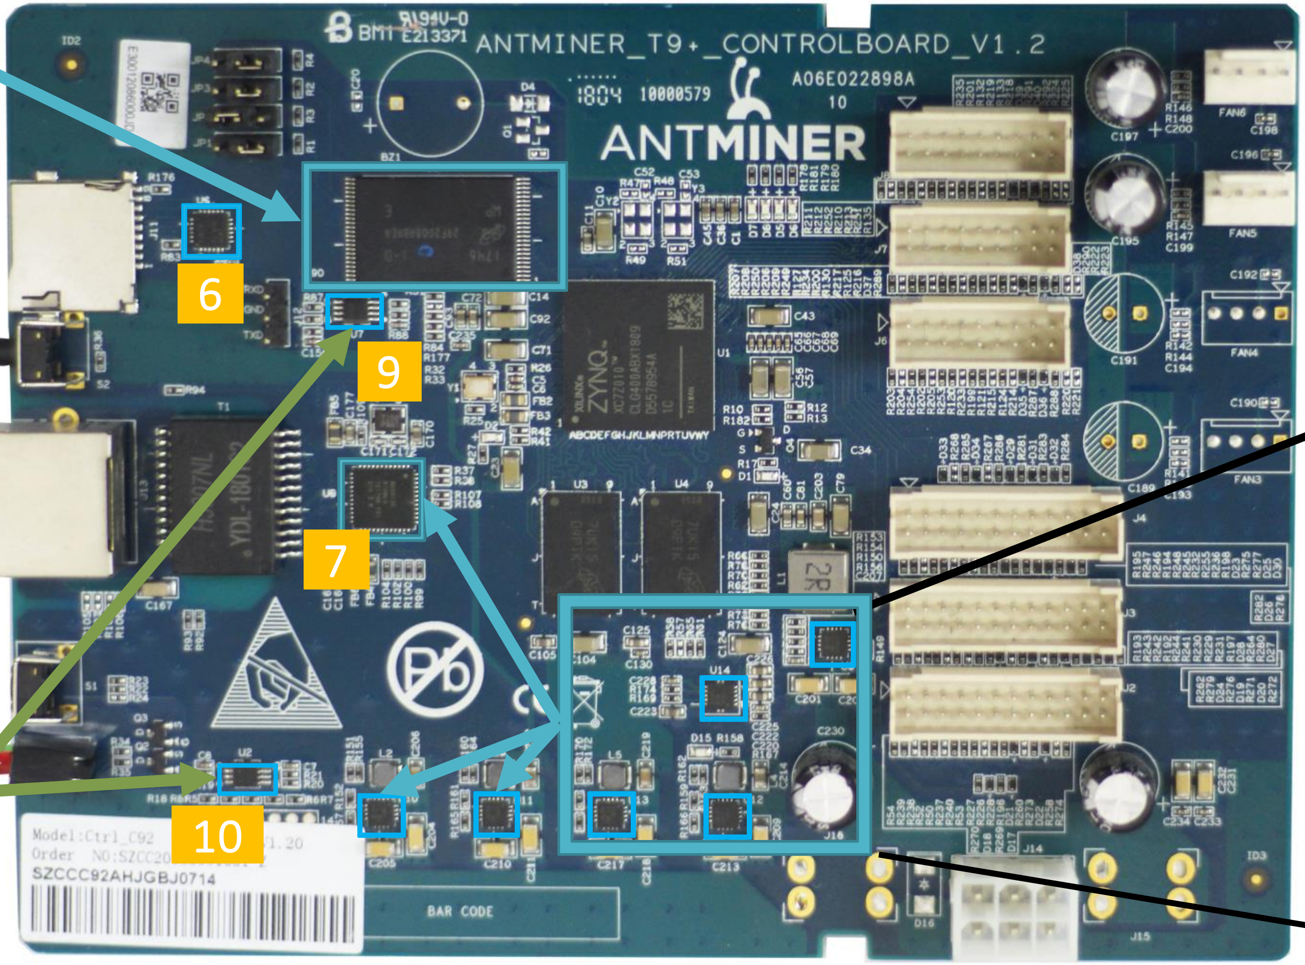


Picture from: [5]

IC, TQFP 32-100

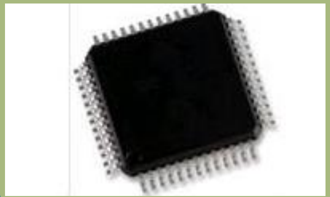

x6 +1+1

1 with ID 5 and
6 with ID 6
1 with ID 7

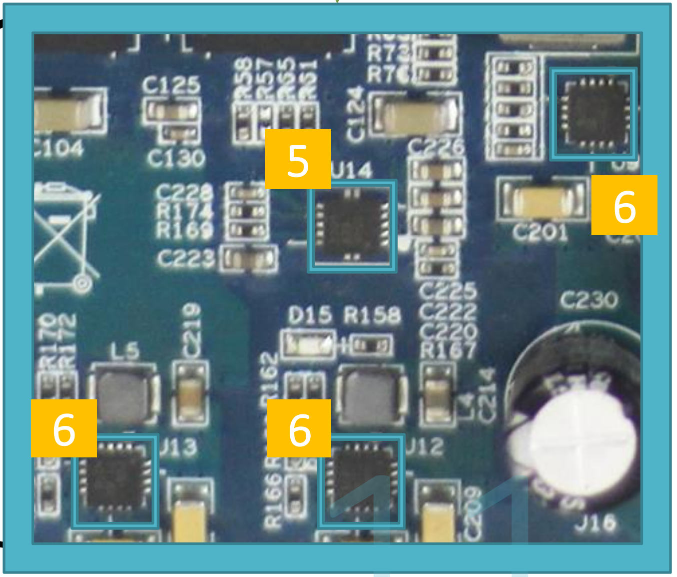


Picture from: [5]

# Control Board: capacitors

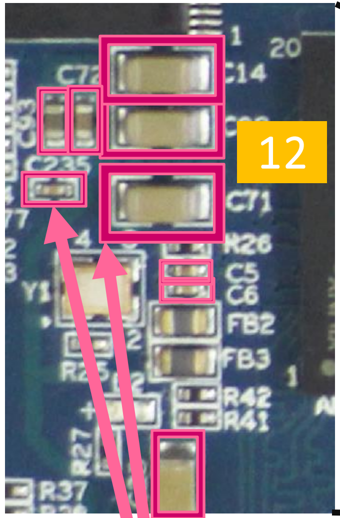


Picture from: [5]

~ x230
Big:
~ x24

Capacitor ceramic MLCC

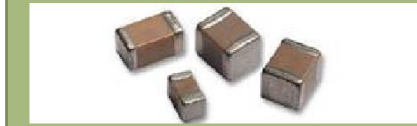

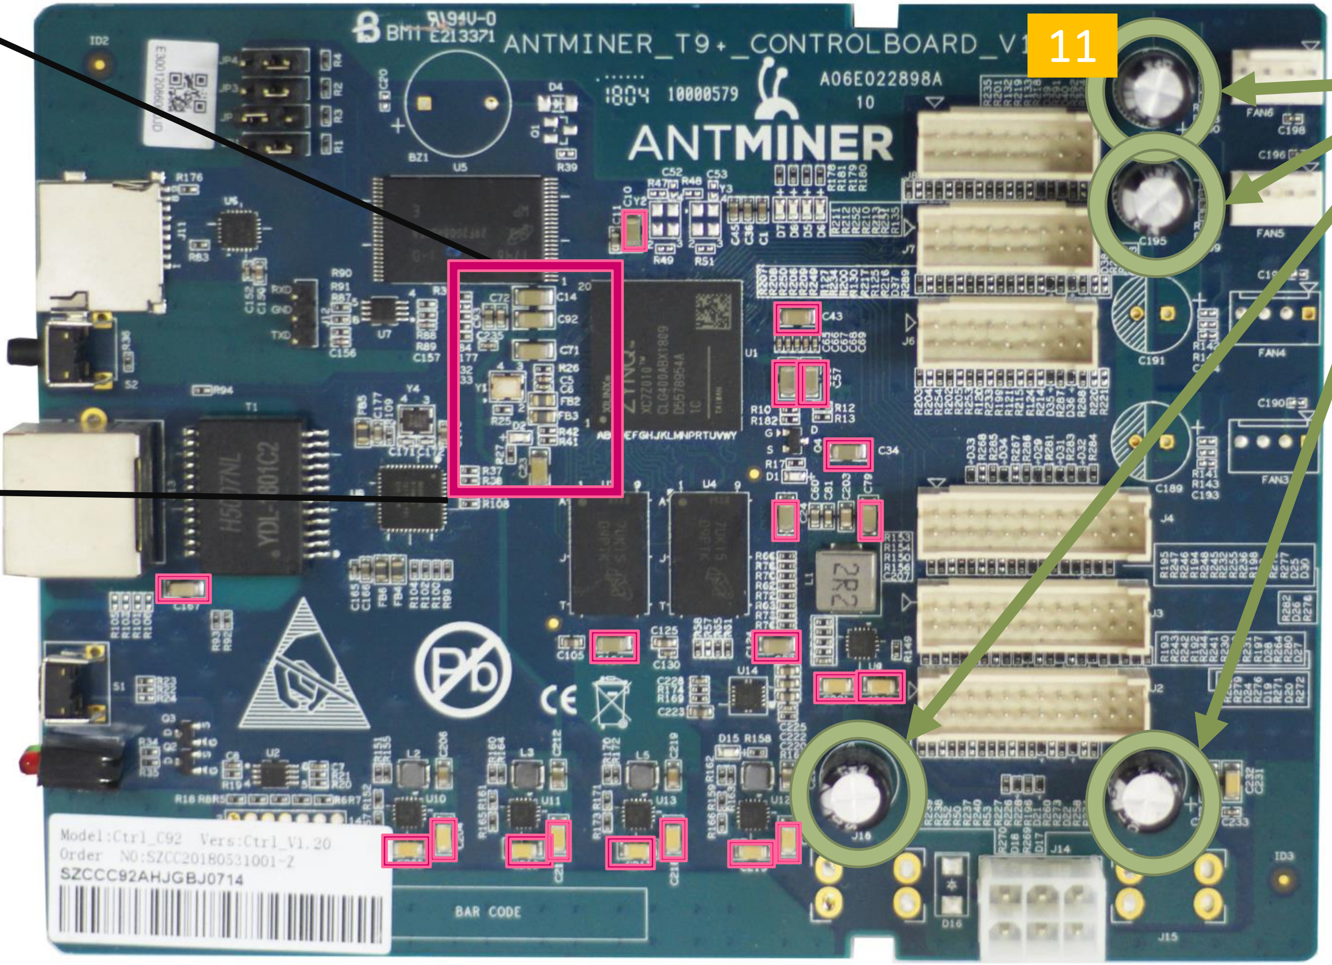


Picture from: [5]

x4

Capacitor Al – capacitor radial THT

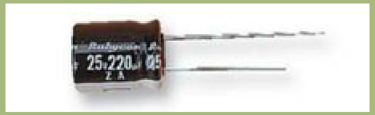

Electrolytic capacitor THT

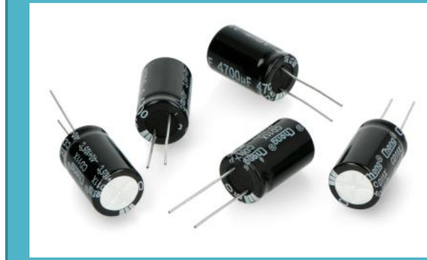

[8]

# Control Board: Inductors & Resistors

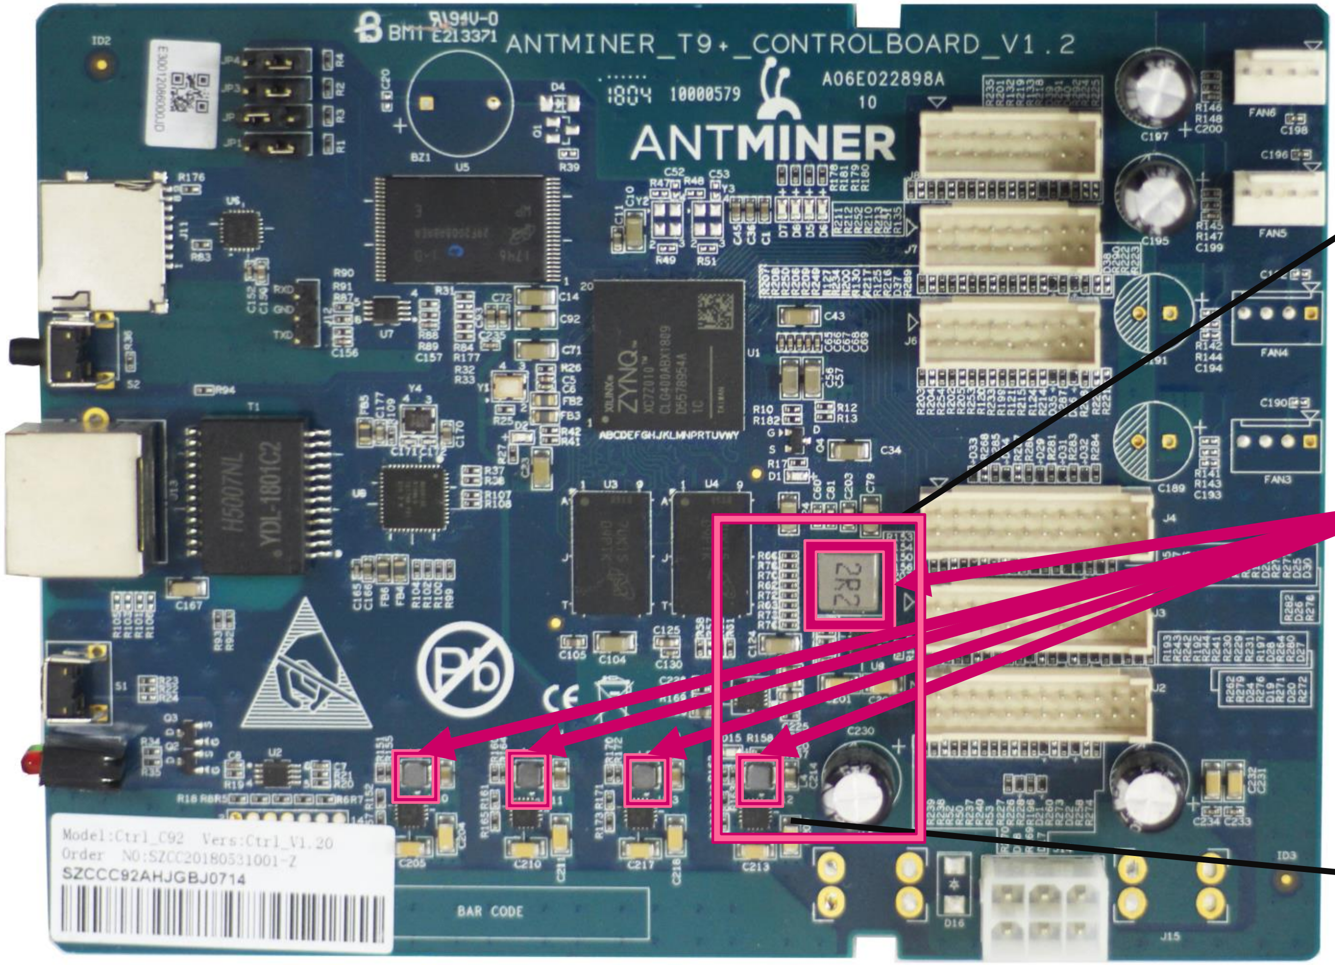


Picture from: [5]

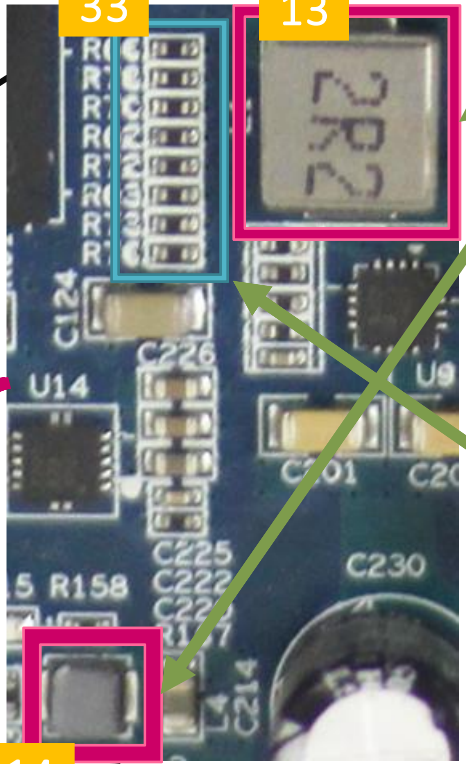


Picture from: [5]

**Inductors:**
Coil miniature wound SRP

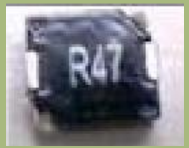

x4 +1

1 with ID 13
+ 4 with ID 14

**Resistors**
Flat chip

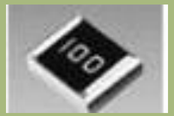

~x190

# Control Board: Diodes

Diode signal DO214/219

15, 16, 17, 18

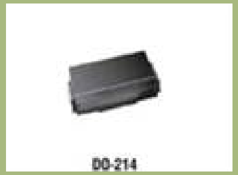


~ x40
(16 on the PCB v1.0)

empty footprint

15

16

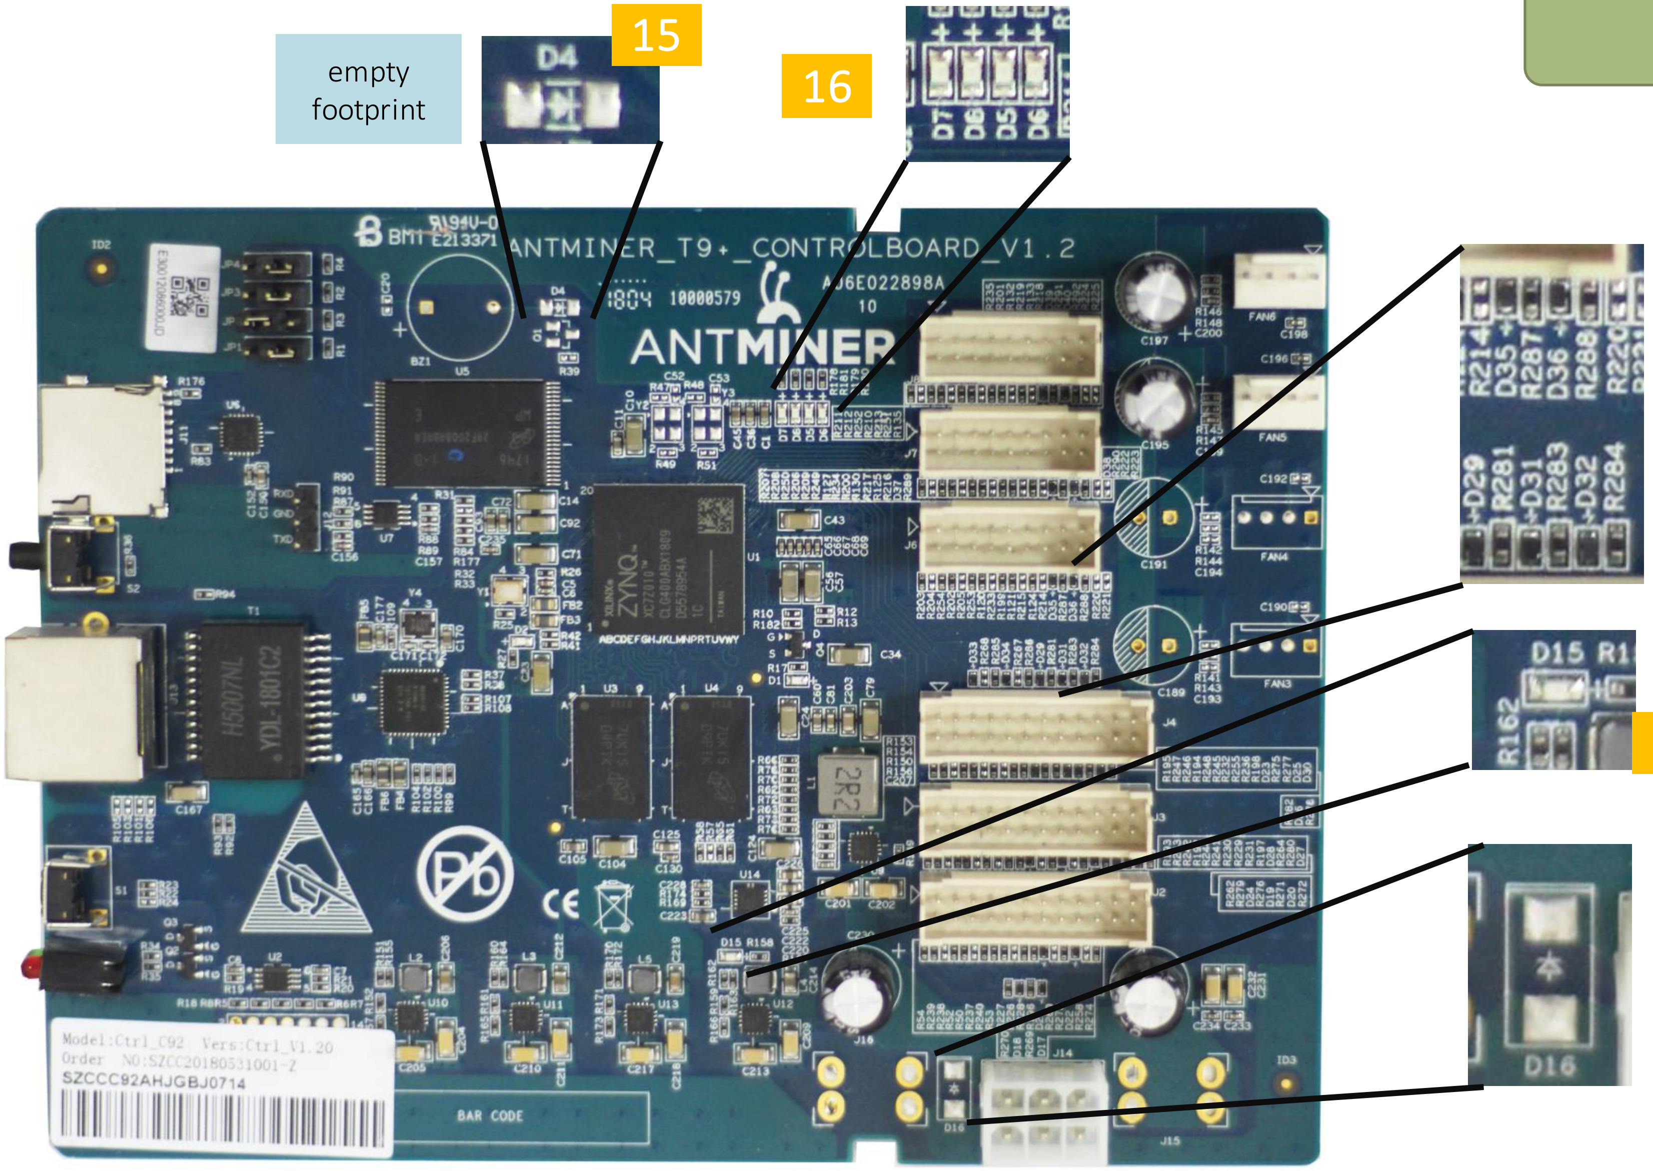


17

16

18

empty footprint

Picture from: [5]

# Control Board: Diodes (v1.0)

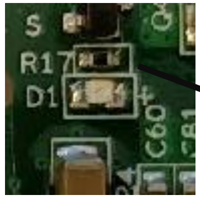


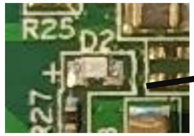


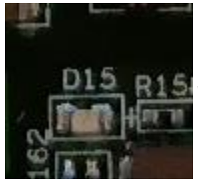


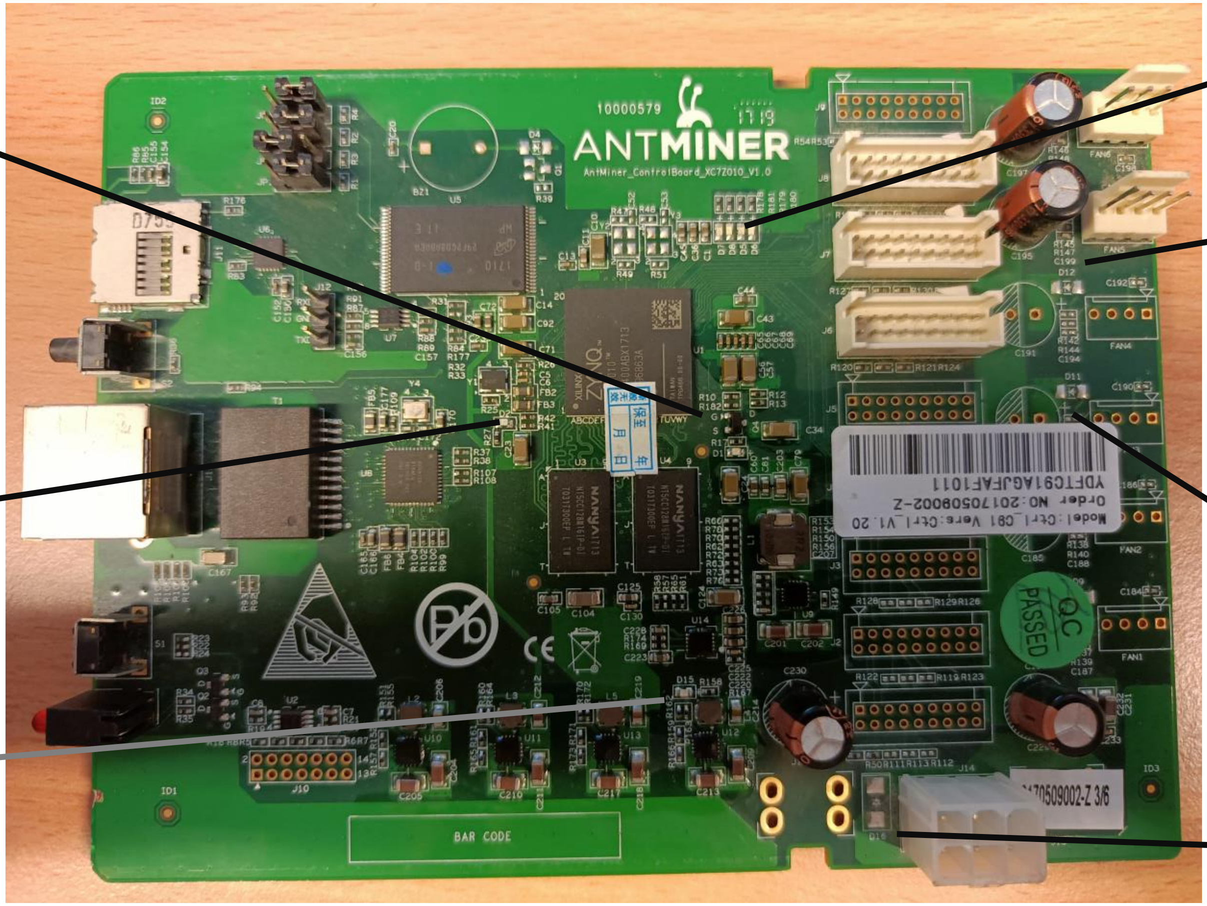


Picture from: Ludmila Courtillat--Piazza

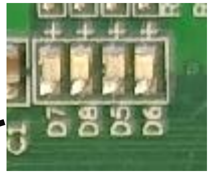


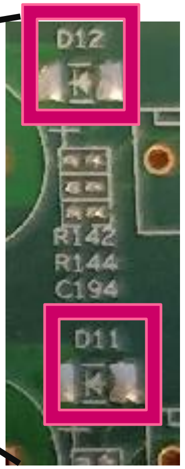


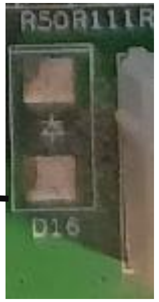


15, 16, 17, 18

Diode signal
DO214/219

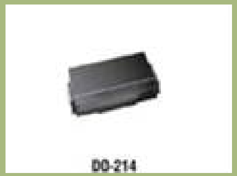


x16
(among whom, half are empty footprints)

# Control Board: Connectors

**Connectors:**
No information from GaBi documentation

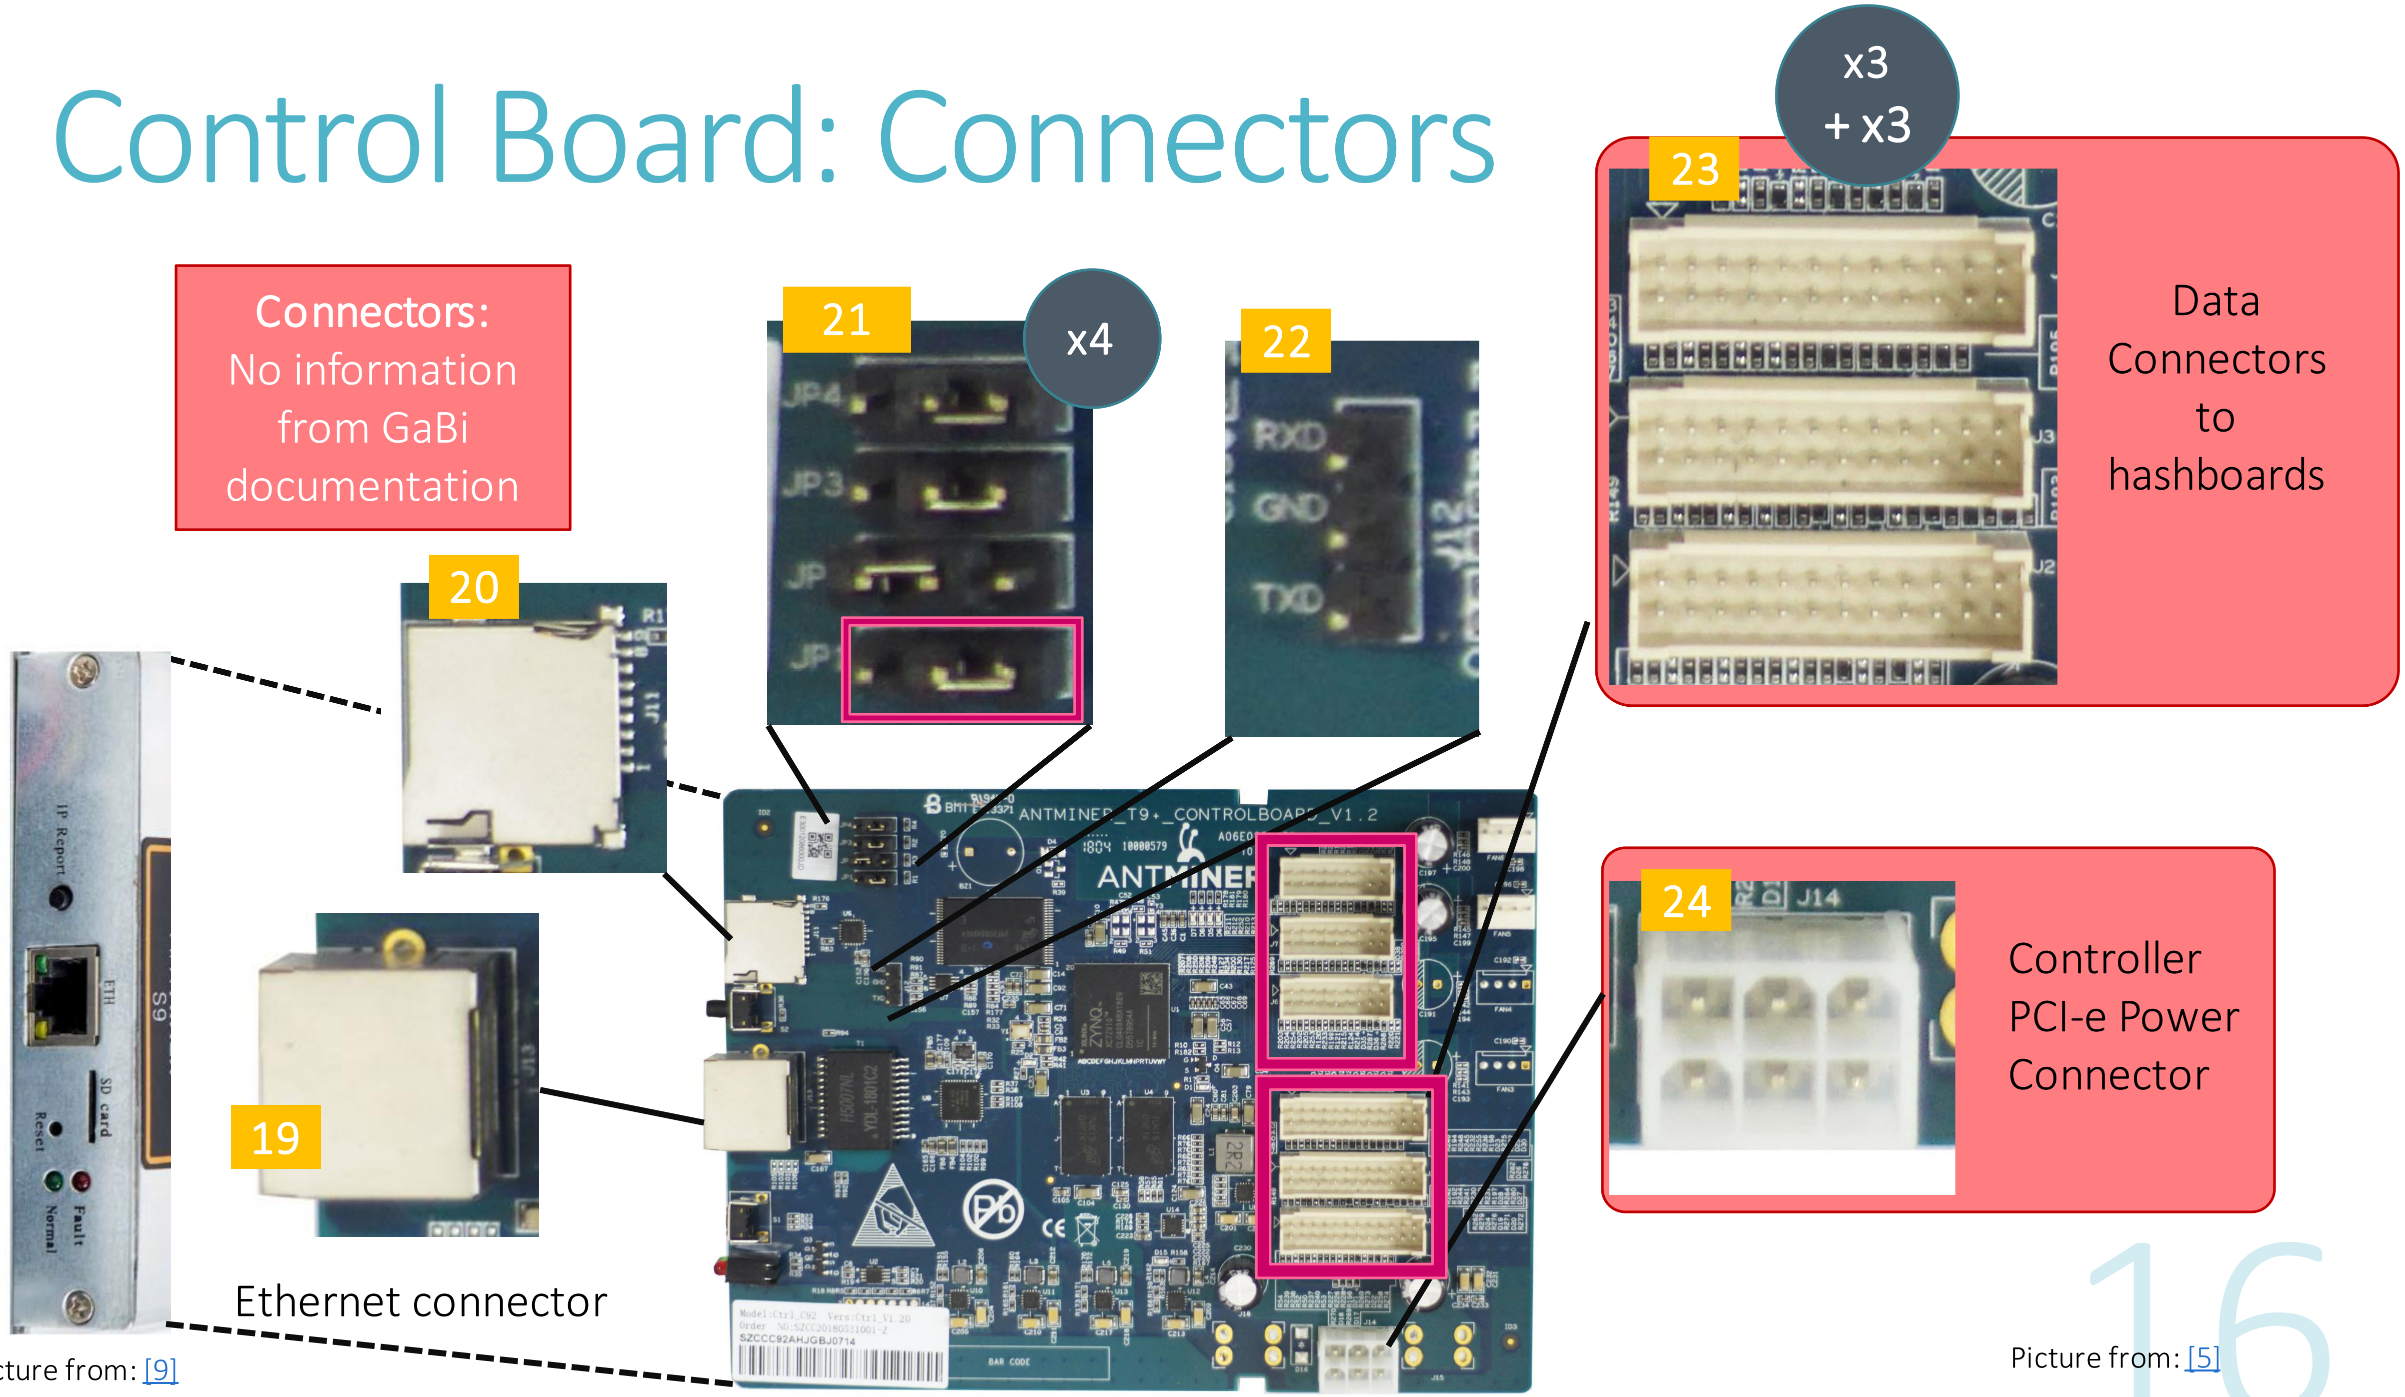


Picture from: [9]

Picture from: [5]

# Control Board: Transistors

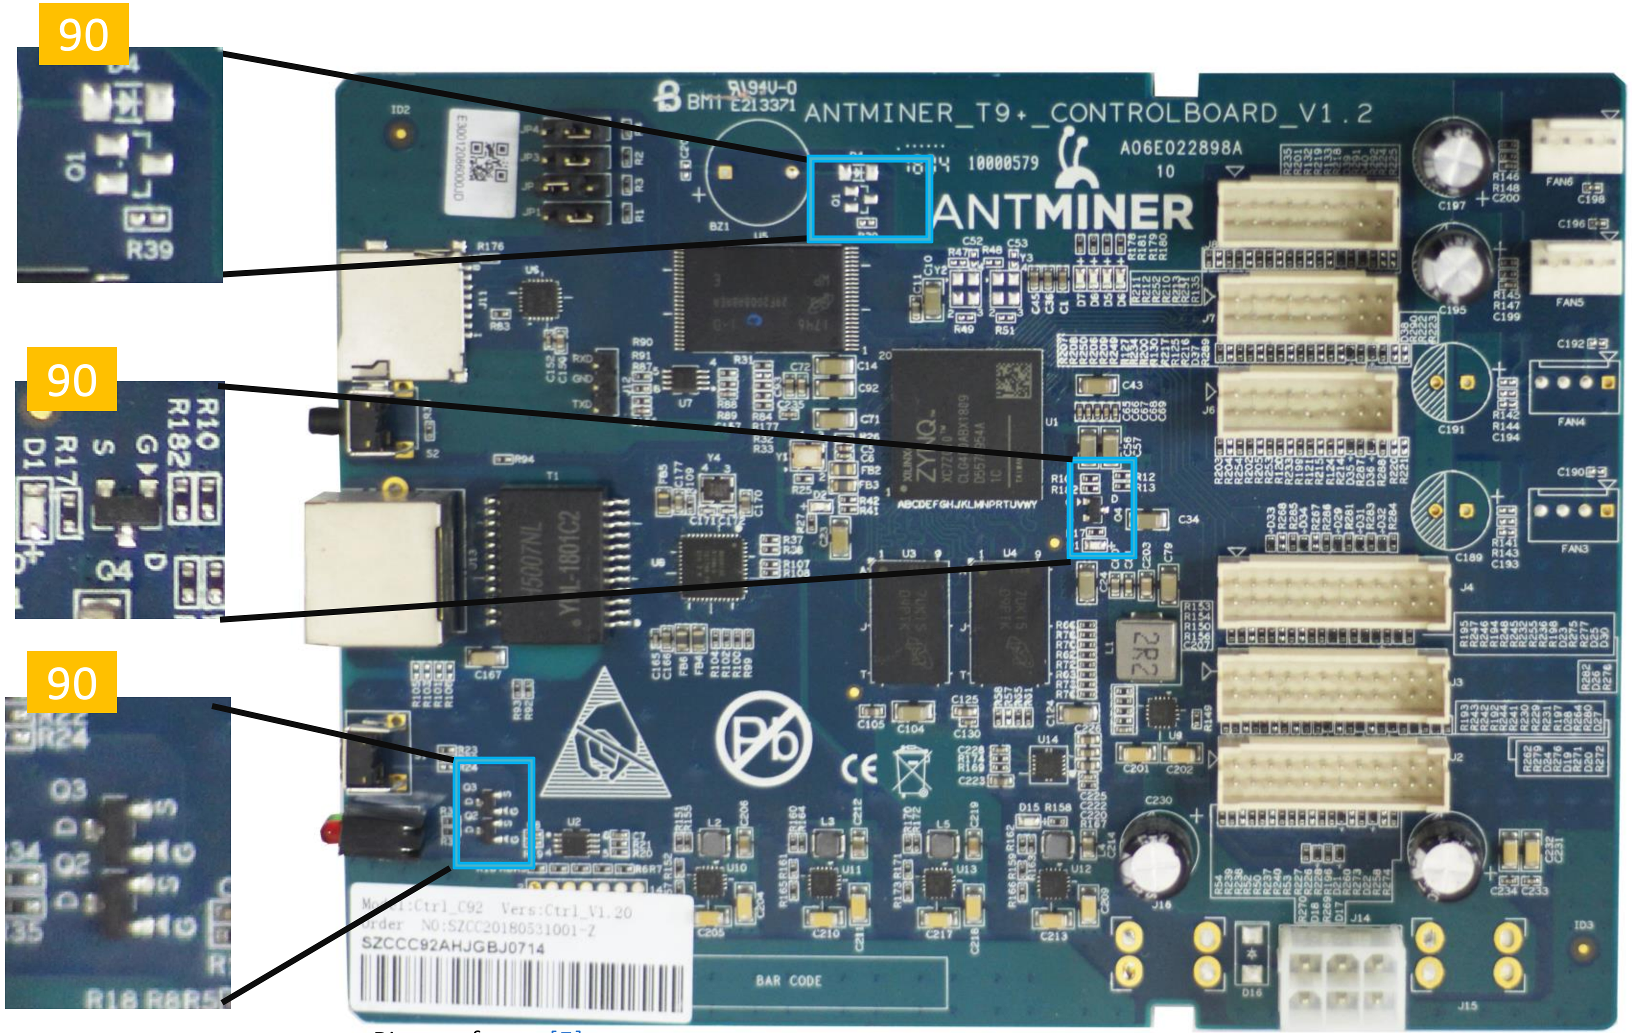


Picture from: [5]

Transistor DPAK TO 252

90

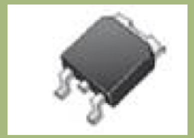

x4

# Control Board: Other components

Switches:

26

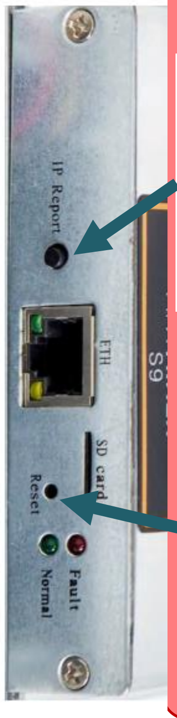

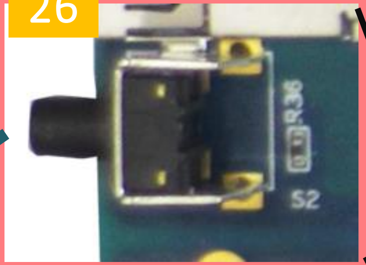


27

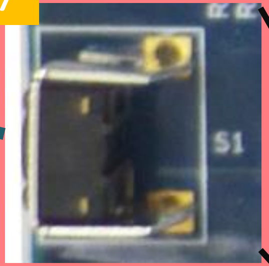


Picture from: [9]

FB -> resistors

x6

33

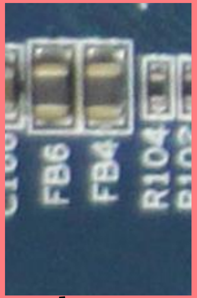


Oscillator crystals

x3

30

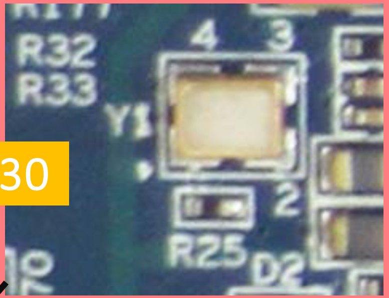


31

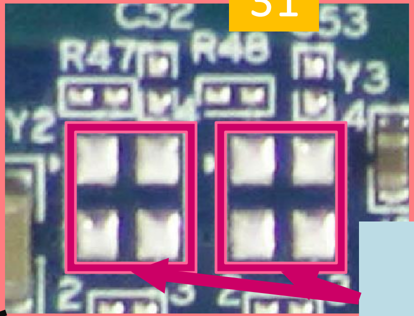


Remark: empty footprints here

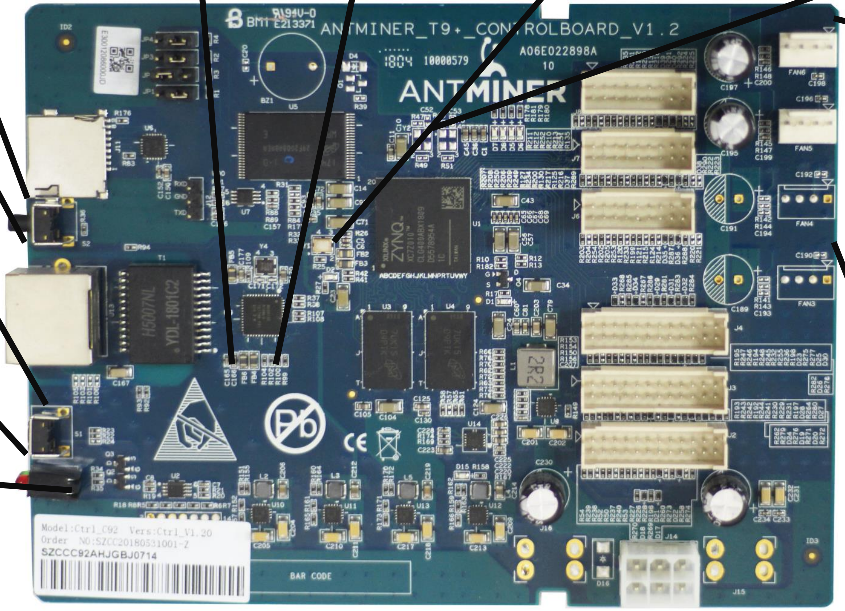


32

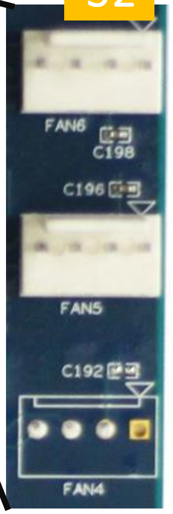


Fans connectors

x2 (4 footprints)

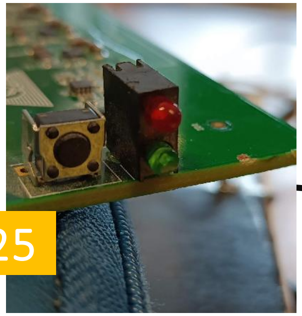

25

Picture from: Ludmila Courtillat--Piazza

Picture from: [5]

# Control Board: side B (v1.2)

(Remark: the PCB that we have (v1.0 is really different from this one) see next slide

12
Capacitors:
side A + B: > 666
Big: +2

> x666
Big:
~x23

4
Memory
+1 ->

x2

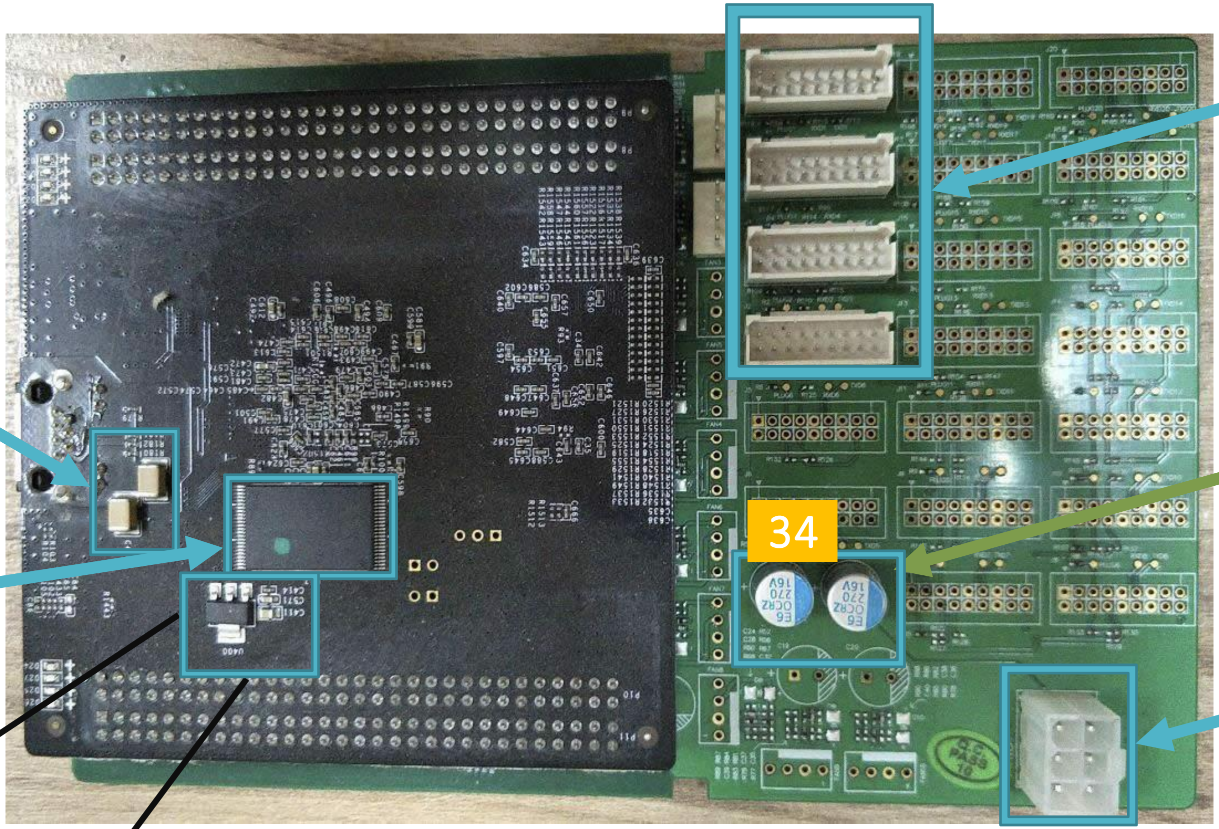


26
Connector
+4 ->

x10

11
Capacitor Al – capacitor radial THT

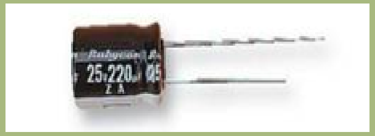


+2 ->

x6

24
Connector
+1 ->

x2

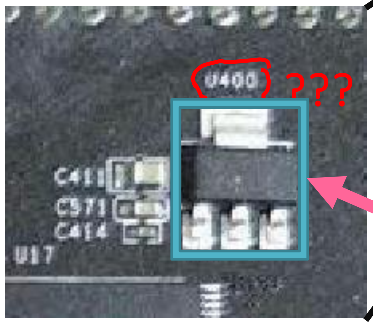


Picture from: [6]

91
Transistor

Transistor DPAK TO 252

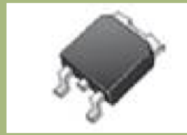

33
Resistors
side A + B:
> x1560

>
x1560

# Control Board: side B (v1.0)

The red crosses indicate elements presents in the v1.2, which does not appear on the v1.0.

12
Capacitors:
side A + B:
190 ~~> 666~~
~~Big: +2~~
> x190

4
Mem[illegible]lash
[illegible]1 ->
x2

91
Transist[illegible]
D[illegible]K[illegible]252

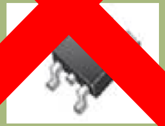

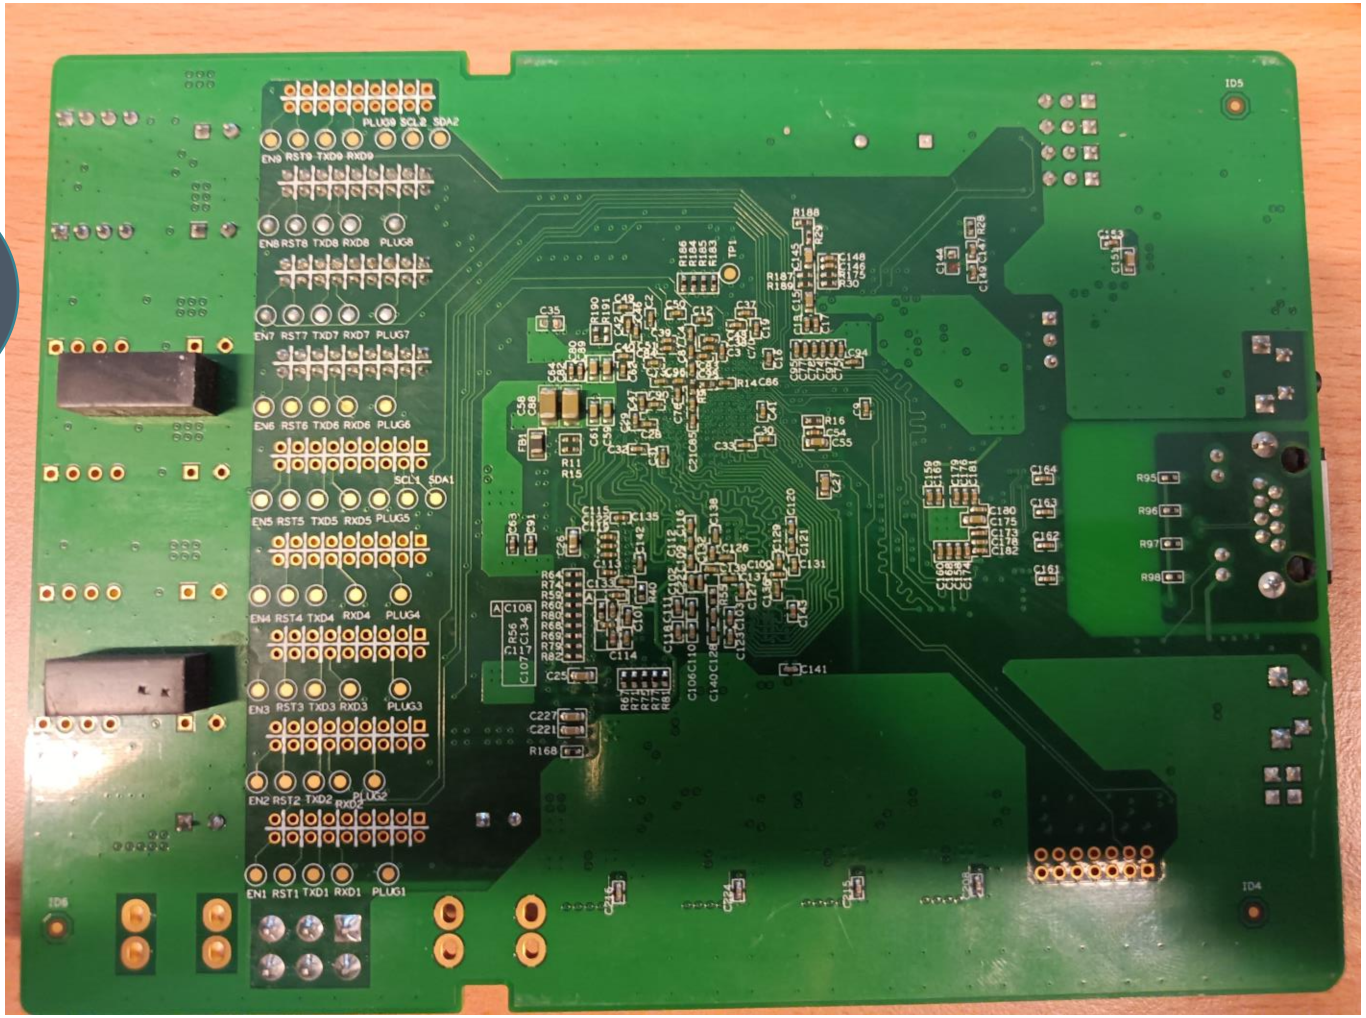

26
Co[illegible]ct[illegible]s to
hash[illegible]rds
[illegible]4 ->
x10

11
Capacitor Al –
capa[illegible]tor radi[illegible]THT

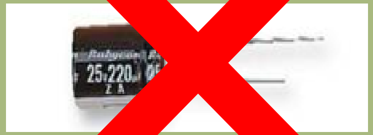

+2 ->
x6

4
C[illegible]n[illegible]tor
PC[illegible]ower
+1 -[illegible]
x2

33
Resistors
side A + B: 200
~~> x1560~~
> x200

# Hashboard

Hashboards are used to do the parallel computations needed by the proof-of-work protocol.

There are 3 hashboards in the Antminer S9.

# Hashboard: the two sides

Even if there are 3 hashboards in the Antminer S9, in the following all the quantities are provided for ONE hashboard !

Upper side

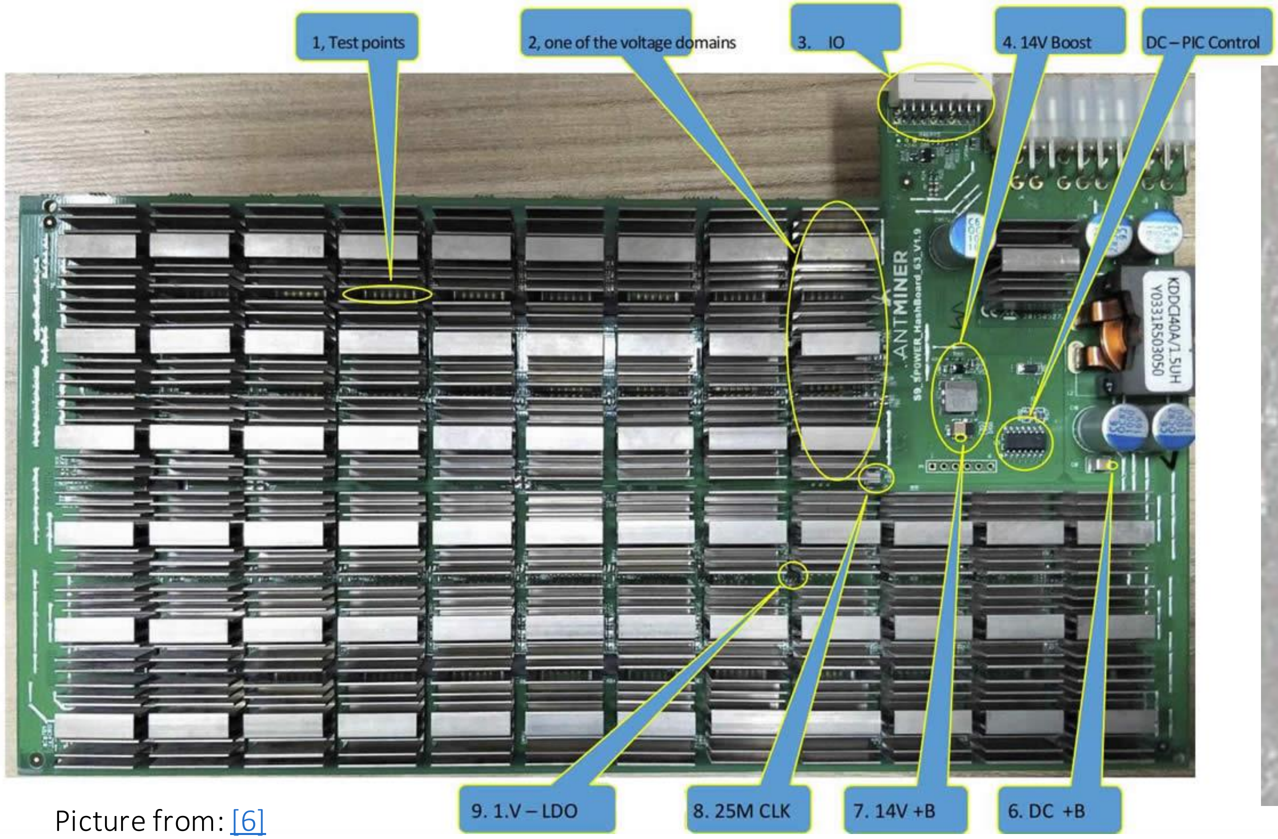


Picture from: [6]

Lower side

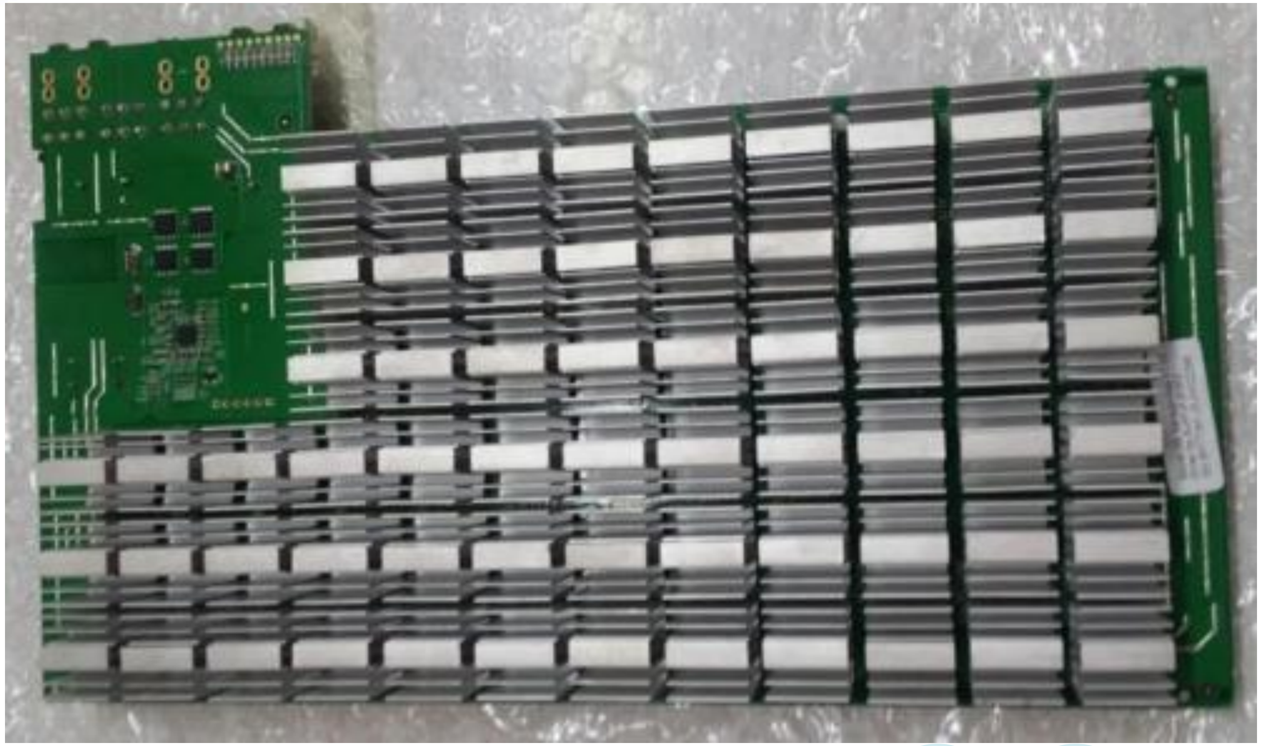

Picture from: [10]

# Hashboard: PCB

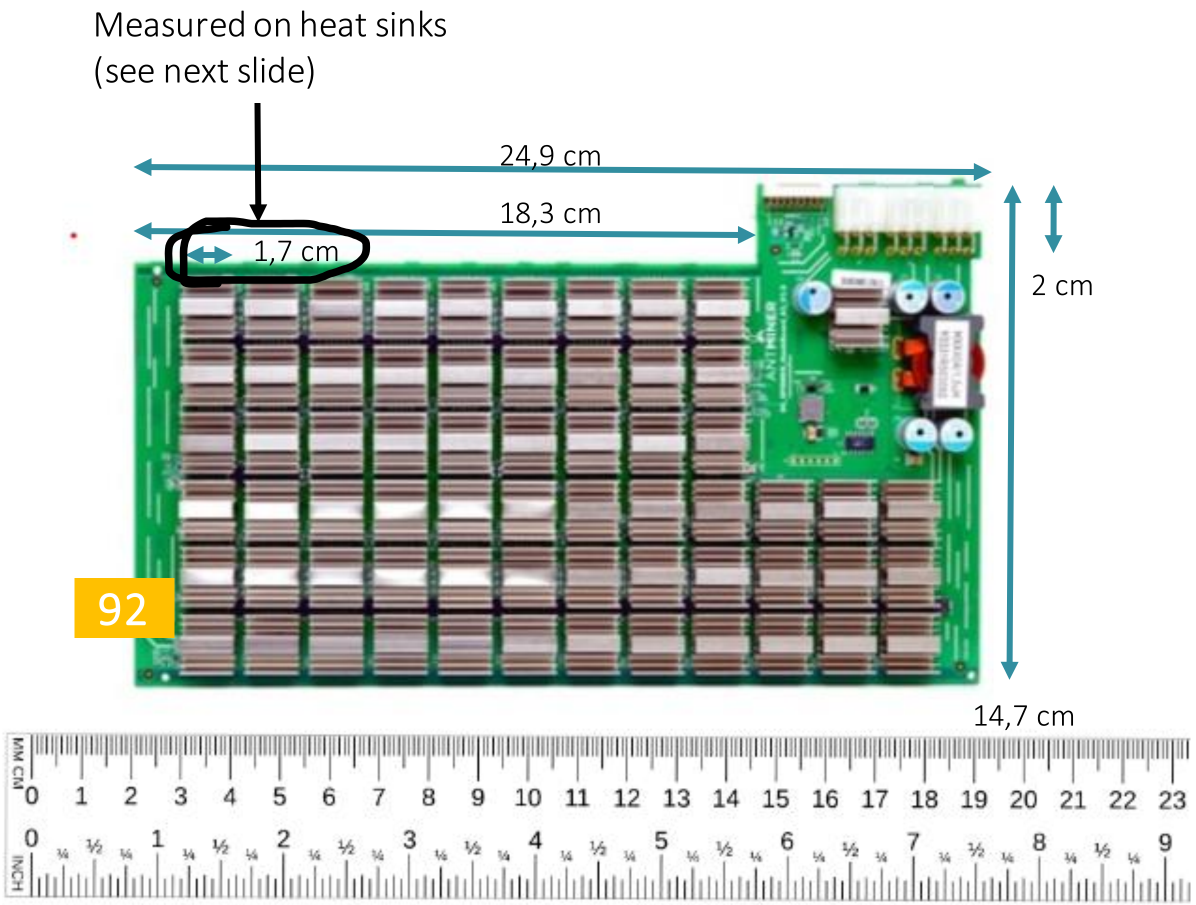


The dimensions and area of the hashboards were deduced from the observation of the real dimensions of the heat sinks and scaling on pictures.

Picture from: [49]
Capture from Ludmila Courtillat- -Piazza
Roler tool from: [50]

# Hashboard: heat sinks

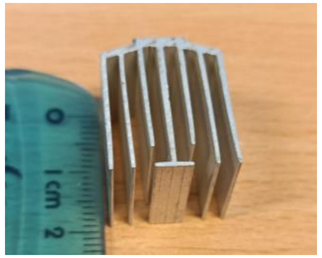


Picture from Ludmila Courtillat--Piazza

x127

35

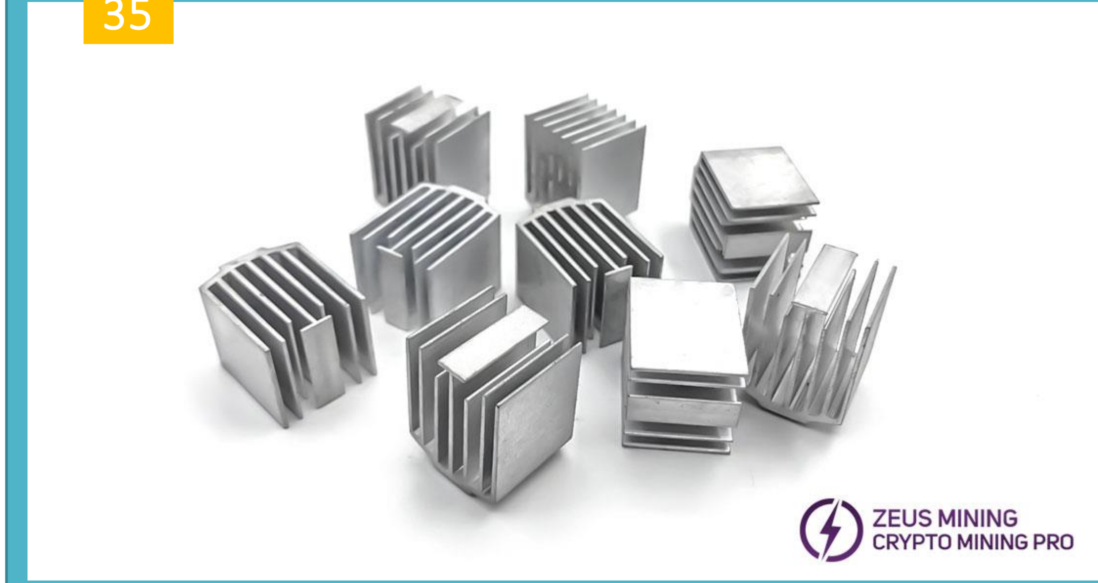


[11], [12]

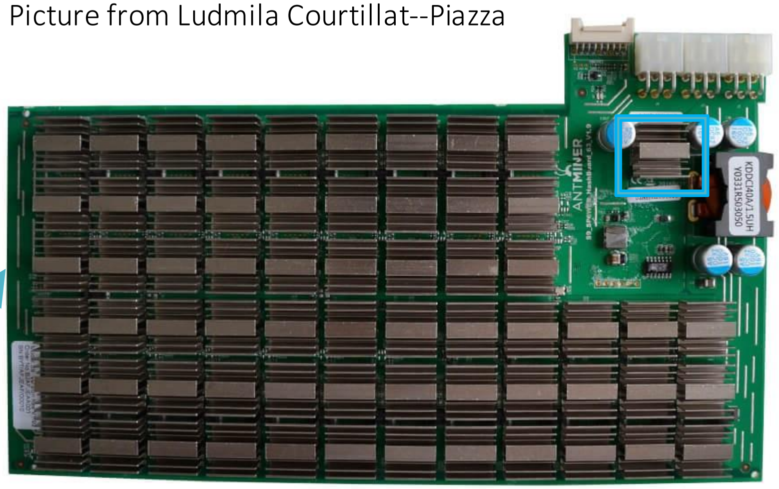


Picture from: [15]

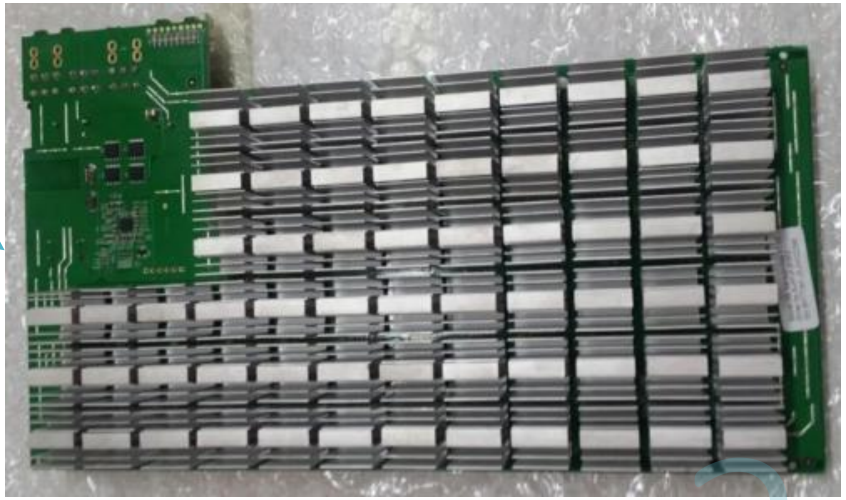

Picture from: [10]

# Hashboard: ASICs (BM1387)

x63

36

« ANTMINER / BMT387B / A10018AT1 »

BM1387B

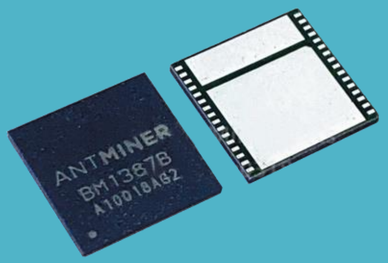


BGA, 16nm

[13], [14]

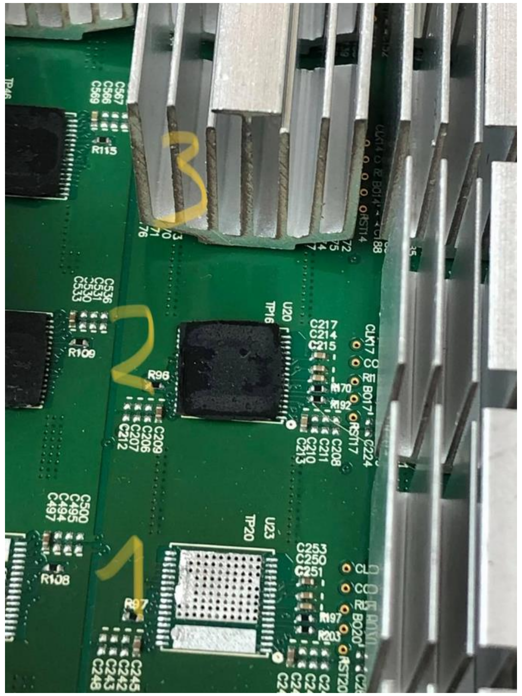


Picture from: [13]
(no longer available)

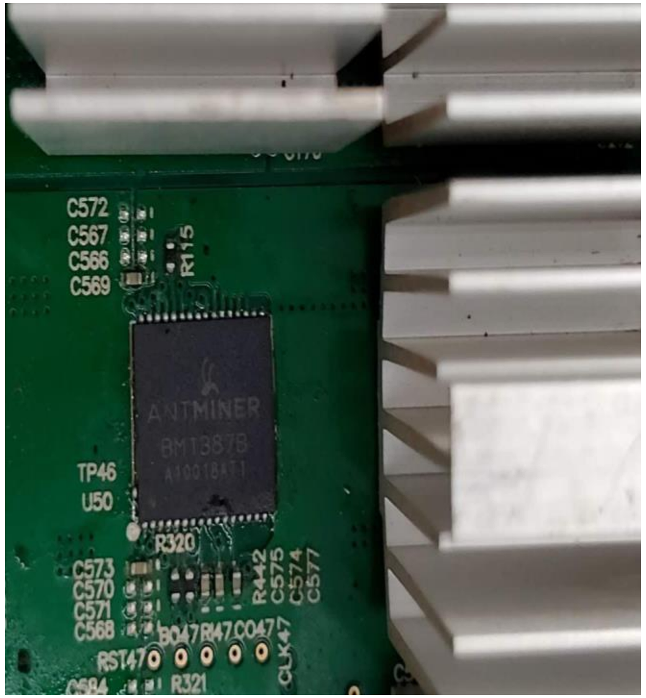


Picture from: [13]

# Hashboard: ICs (others)

37

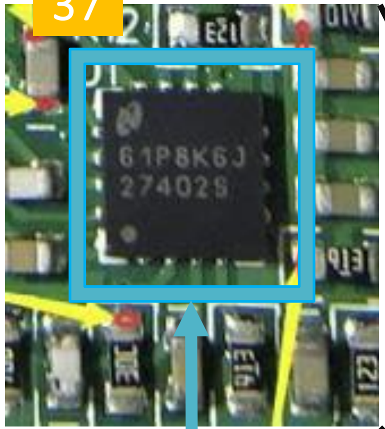


Picture from: [6]

« 61P8K6J / 27402S »

**Switching controller**

LM27402S

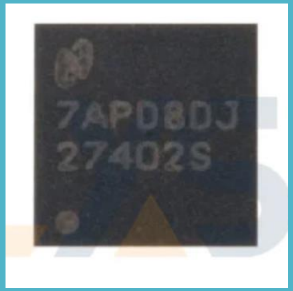


[16], [17]

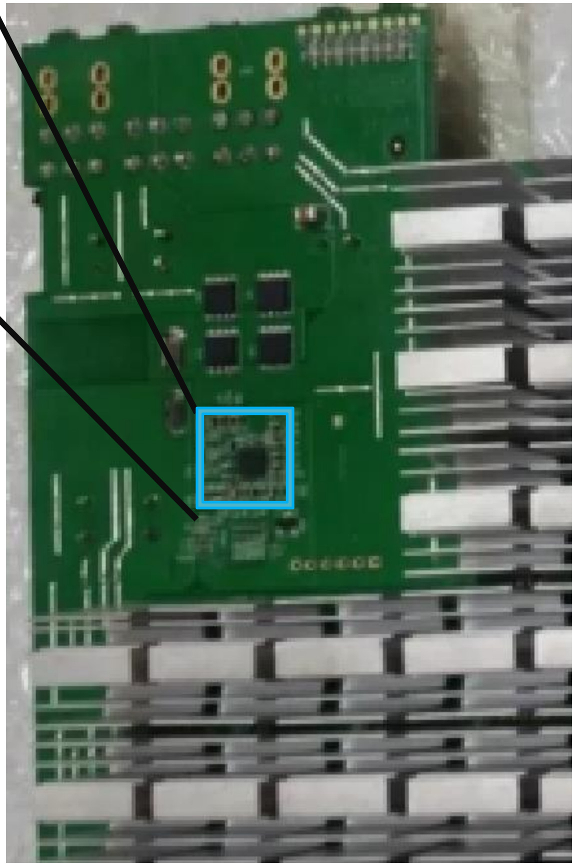

Picture from: [10]

«PIC16F1704 / -V SL 'symbol' / 'symbol' 1612B17 »

**Microcontroller**

PIC16F1704-I/SL

MCU 8-bit PIC RISC 7KB Flash 3.3V/5V Automotive 14-Pin SOIC N Tube

[18]

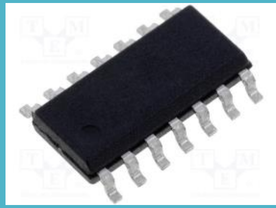

38

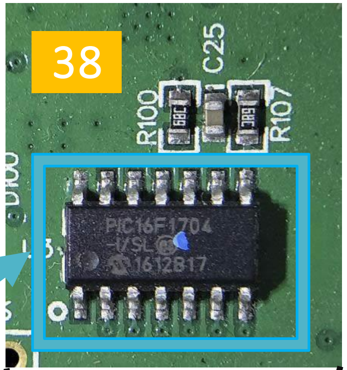


Picture from: [6]

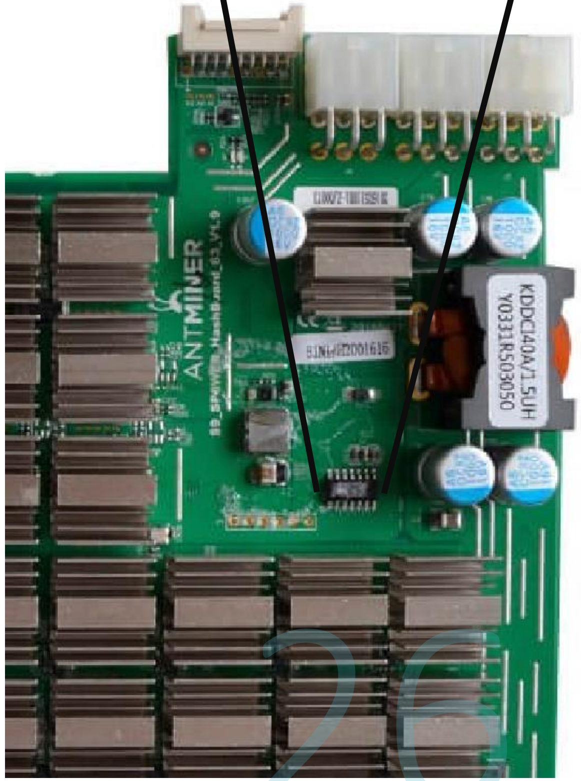


Picture from: [15]

# Hashboard: ICs (Others) and coil

In spite of indication of "LDO-1.8" by sources like [6], we are not able to observe it in pictures. There is uncertainty on the presence of them.

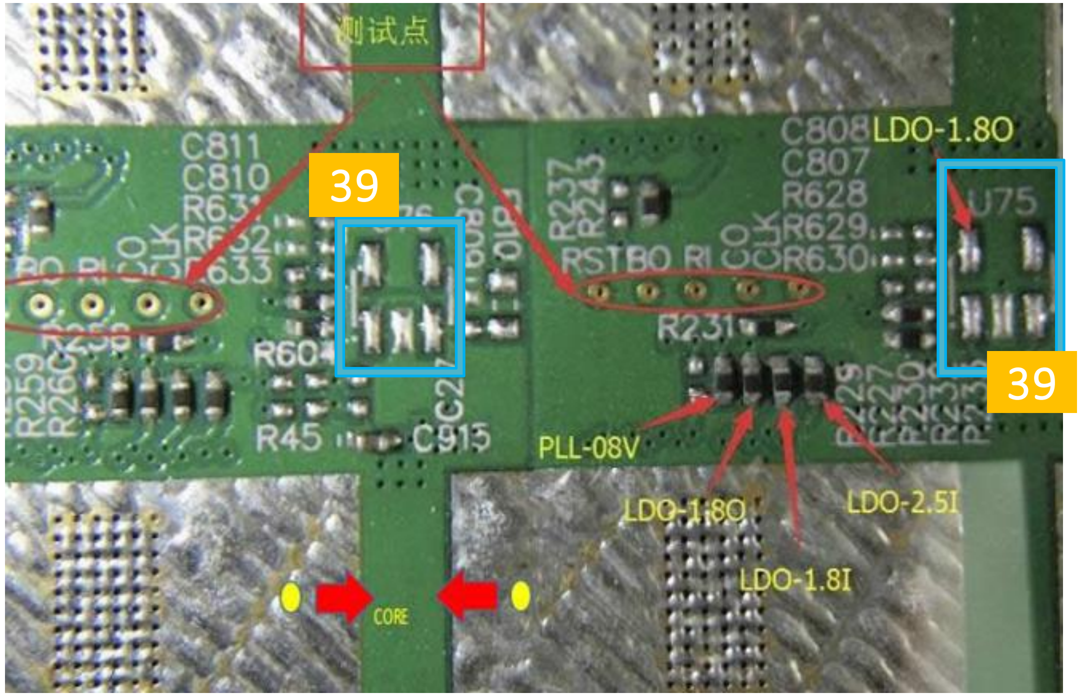


Picture from: [6]

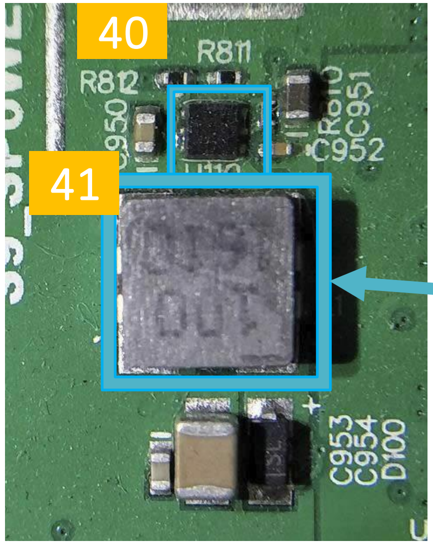


Picture from: [6]

Inductors:
Coil miniature wound SRP

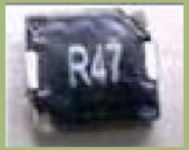

# Hashboard: Capacitors, Diodes & Resistors

93
Resistors
> x 813

94
Diodes
> x 100

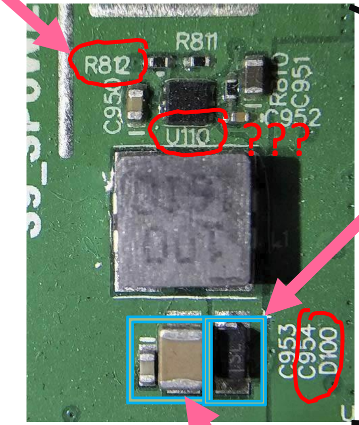


Picture from: [6]

x5
Capacitor Al – capacitor radial THT

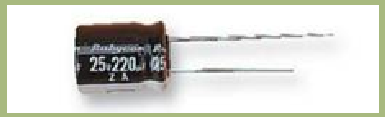

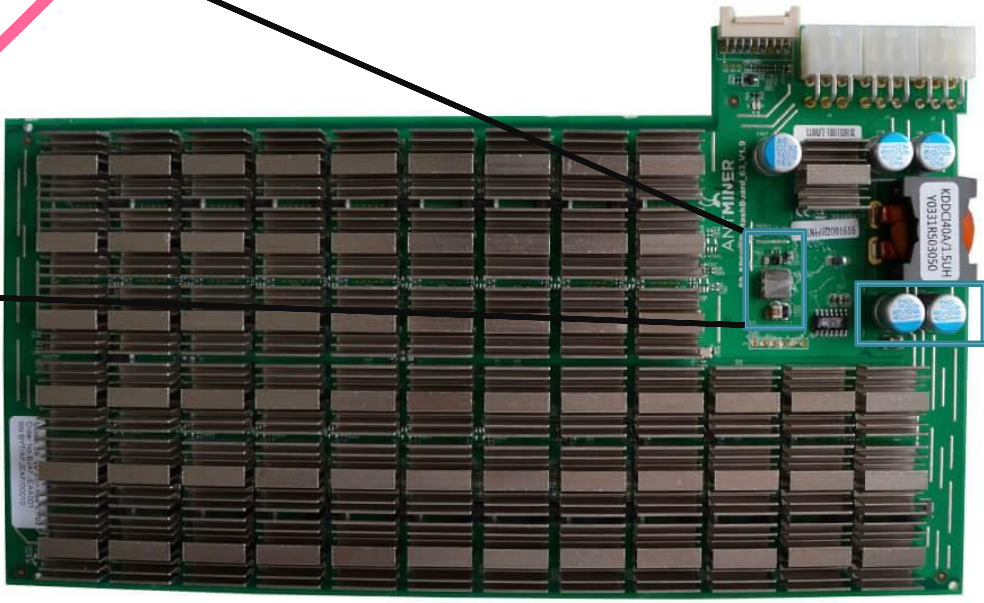

Picture from: [15]

> x 954
Big:
> x 2

95
Capacitor ceramic MLCC

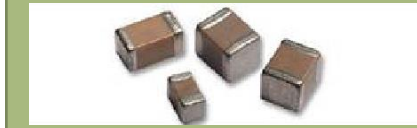

42

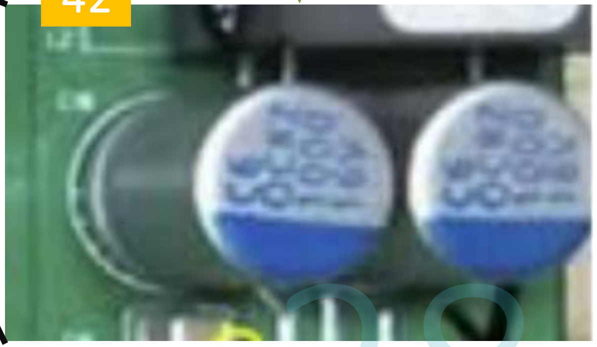

Picture from: [6]

# Hashboard: Transistors

43

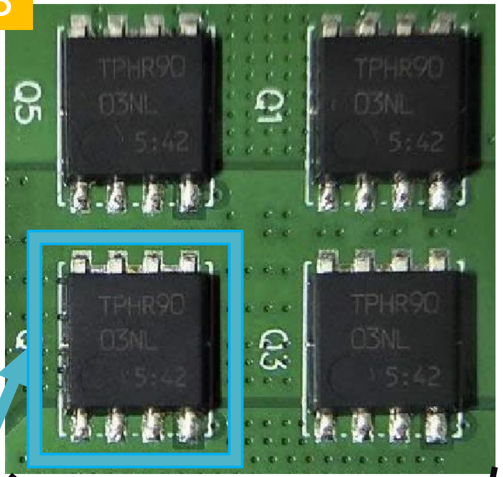


Picture from: [6]

44

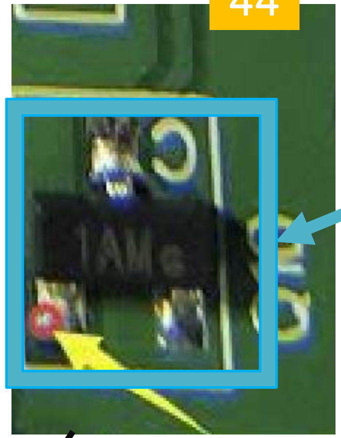


Picture from: [6]

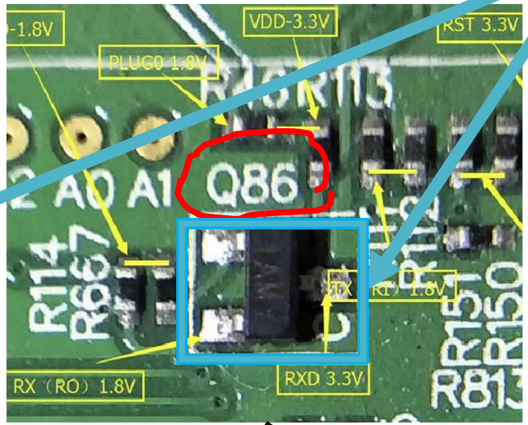


Picture from: [6]

> x2

« 1AM »

SOT-23 MMBT3904

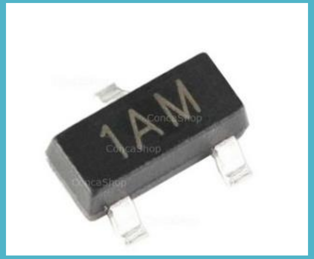


[19]

Transistor signal SOT23 3 leads

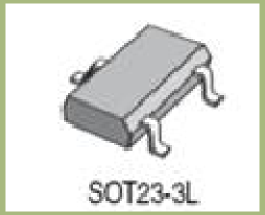


« TPHR90 / 03NL / 5:42 »

TPHR9003NL

x4

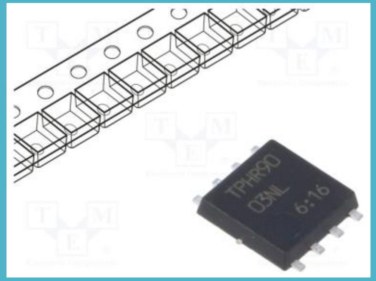


[46]

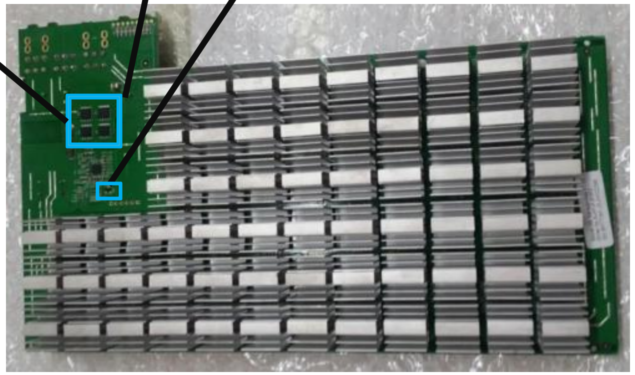

Picture from: [10]

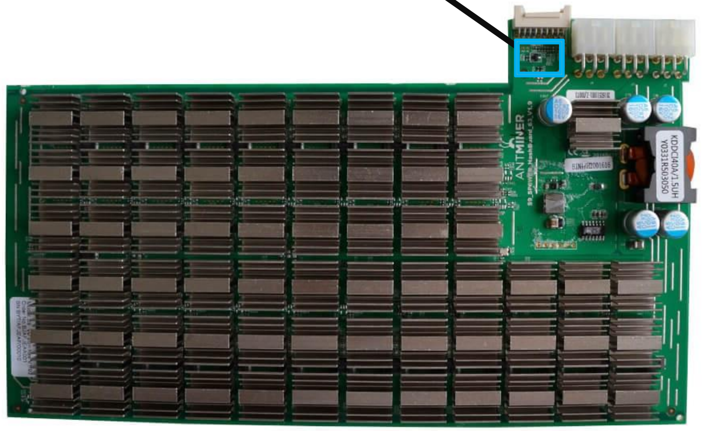


Picture from: [15]

+ Others transistors

Total : > x86

# Hashboard: Inductors

« KDDCI40A/1.5UH / Y0331R503050 »

Y0331R503050 1.5UH power inductor

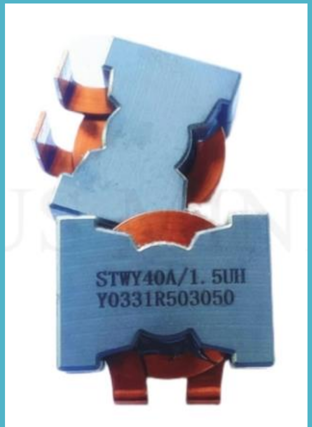


[20]

Ring core coils 8, 30, 80g (with housing)

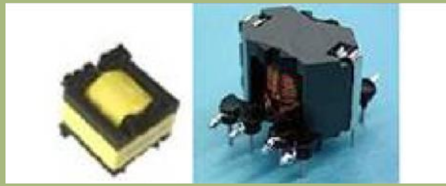

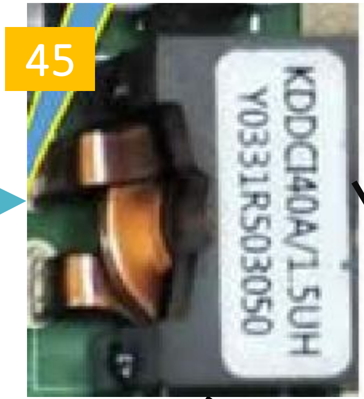


Picture from: [6]

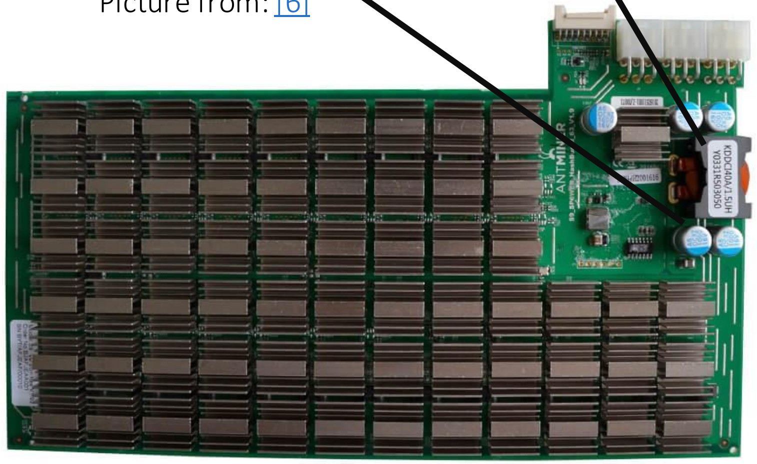

Picture from: [15]

# Hashboard: Connectors

Data Connector

PCI-e power connector

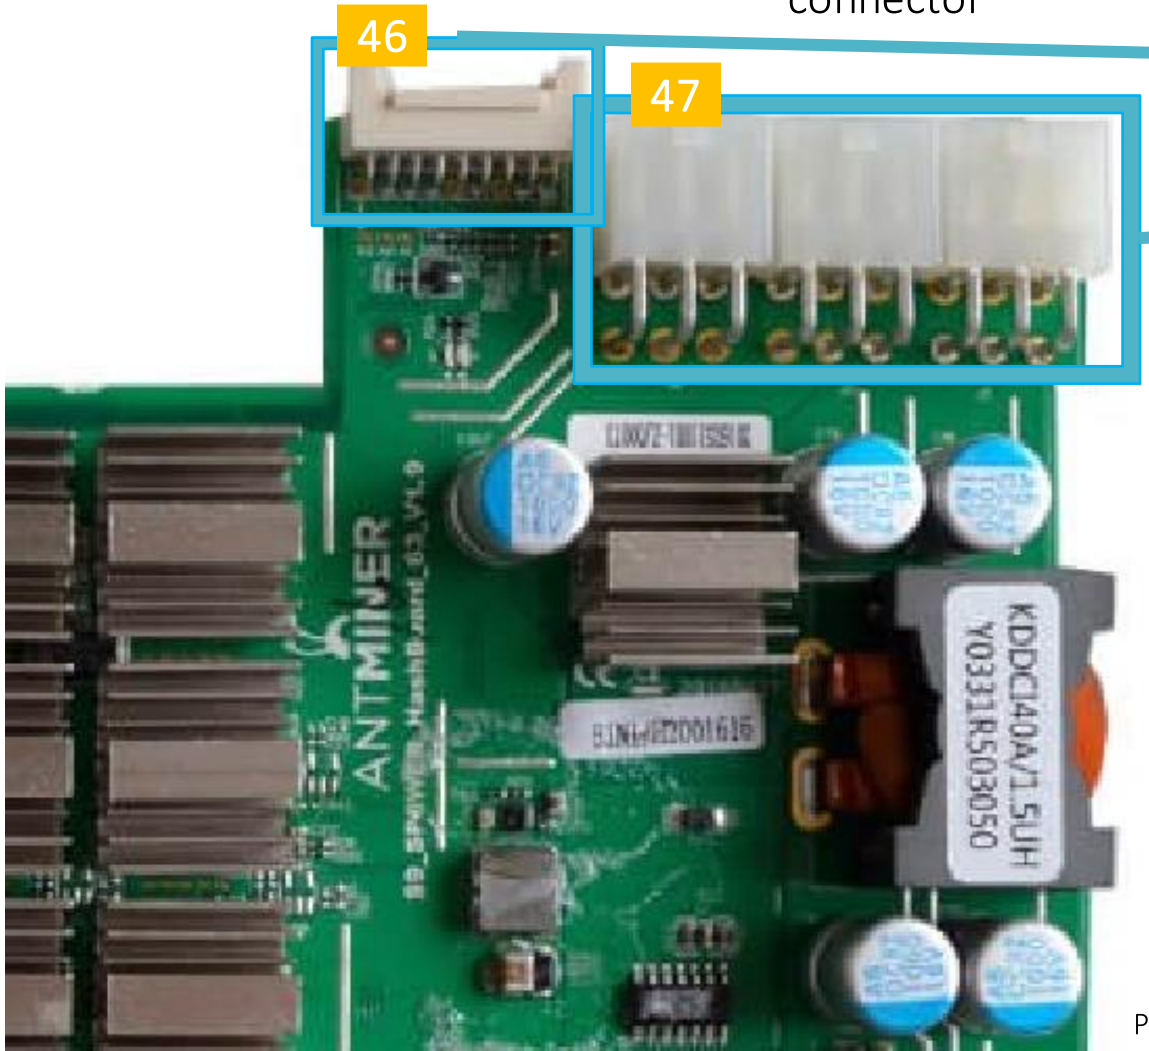


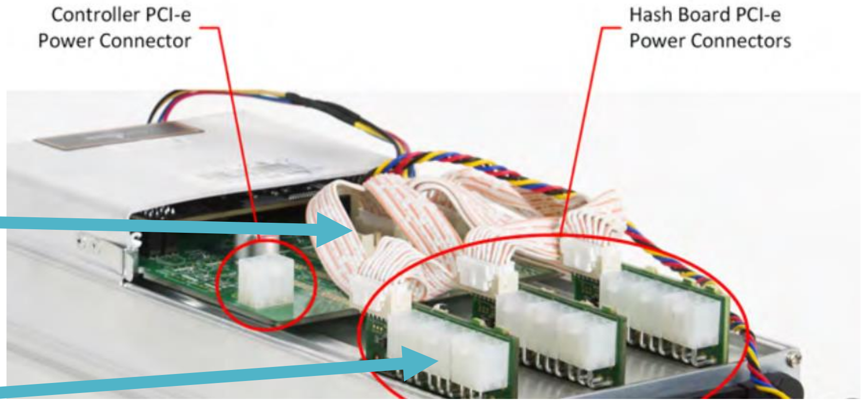


Picture from: [9]

Picture from: [15]

# Power supply

APW3++

It provides electricity to the Hashboards.

# Power supply: General structure and PCB

Size: 220 x 108 x 62 mm [21]

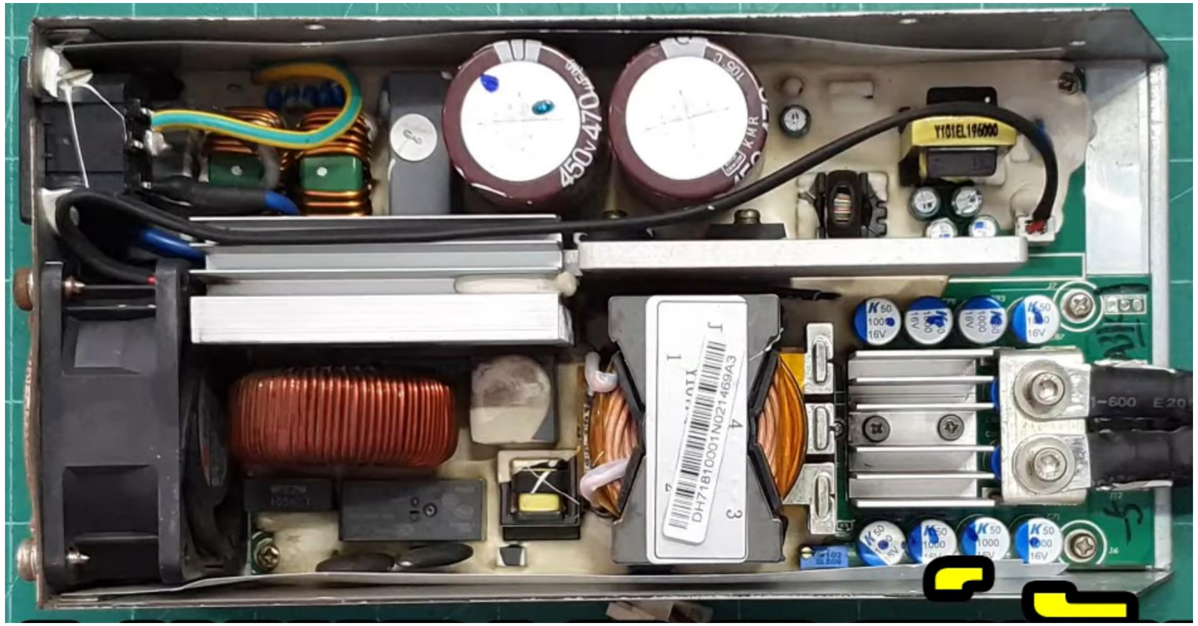

Picture from: [22]

side 1

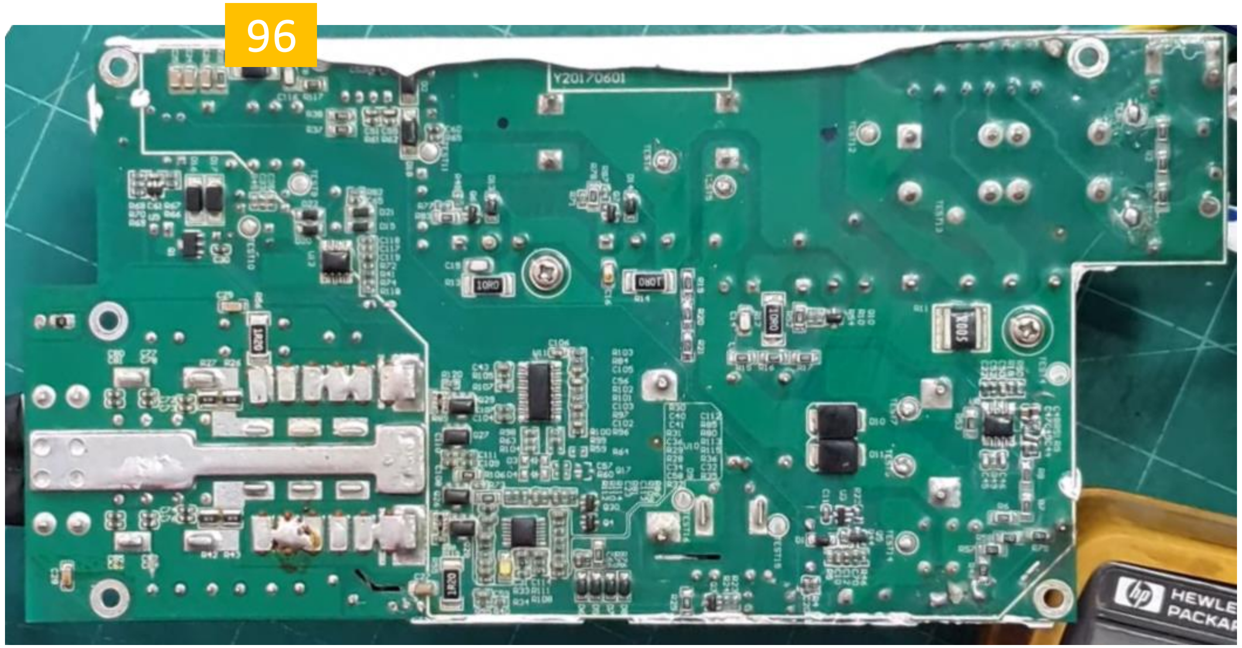


Picture from: [22]

side 2

# Power supply F1 : Capacitors

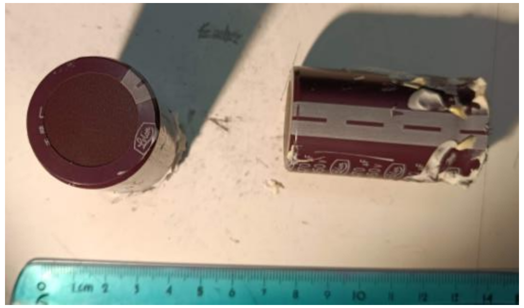

Picture from Ludmila Courtillat--Piazza

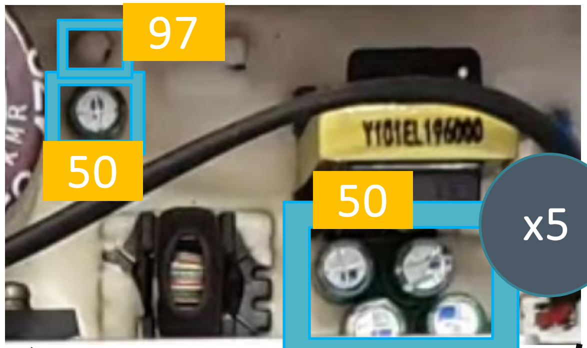


Capacitor Al – capacitor radial THT

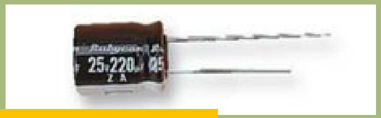

48, 49, 50, 97

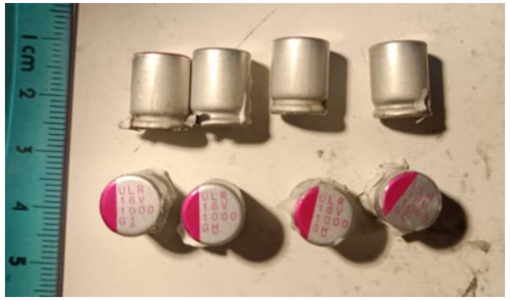

Picture from Ludmila Courtillat--Piazza

48

« 450v470 »

x2

Electrolitic capacitor

Nichicon 470µF Aluminium Electrolytic Capacitor 450V dc, Snap-In - LGU2W471MELC

[23], [24]

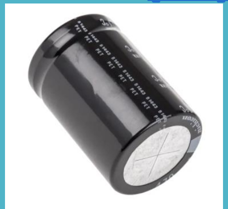

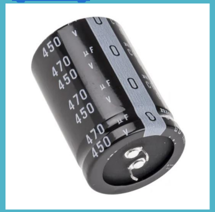

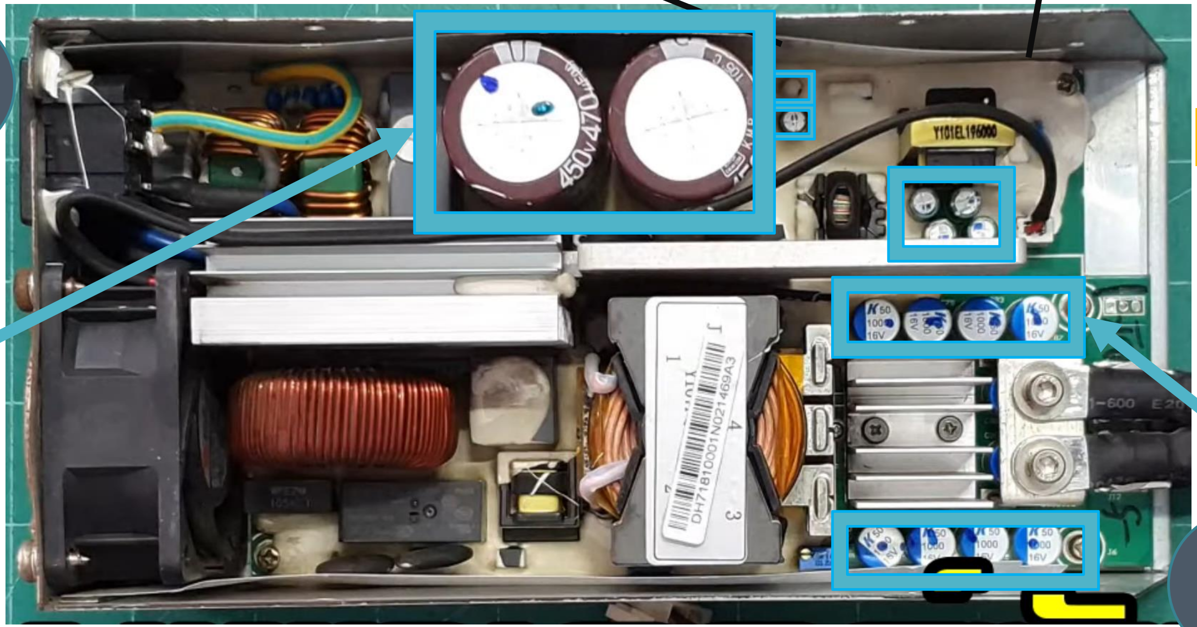

Picture from: [22]

49

« K 50 / 1000 / 16 V »

Electrolitic capacitor

KEMET – 1000uF, 16V, 10x12.5mm, DIP, très faible, ESR 16V, 1000uf, 10x12.5

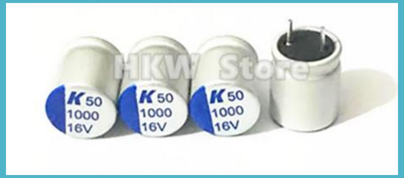


x8

[25]

# Power supply side 1: Inductors

Ring core coils 8, 30, 80g (without housing)

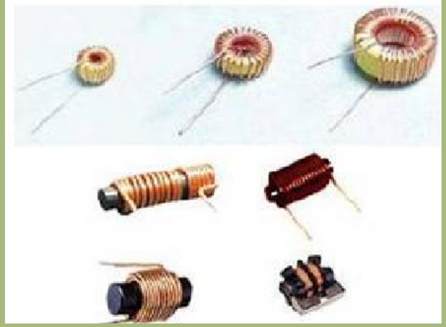

x2

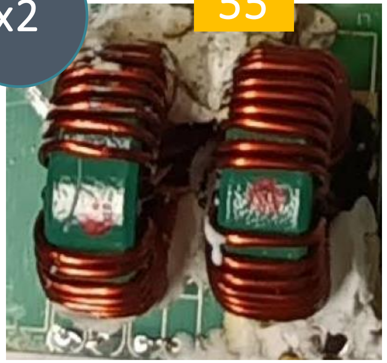


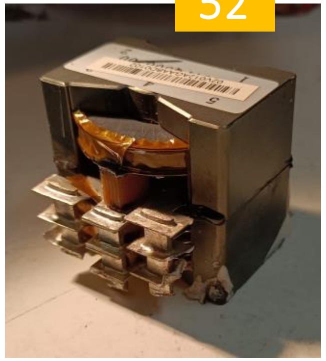


Pictures from Ludmila Courtillat--Piazza

Ring core coils 8, 30, 80g (with housing)

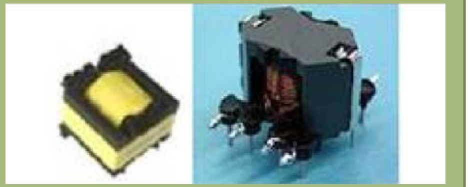

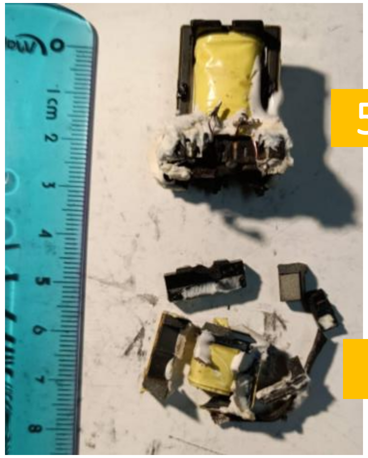


Picture from Ludmila Courtillat--Piazza

« Y101EL 196000 »
Unidentified
But looks similar to
« High frequency transformer »

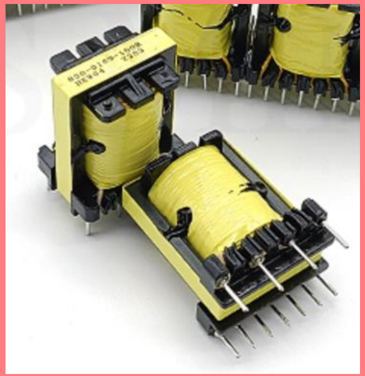

[26]

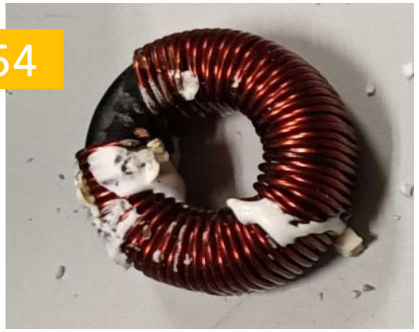


Picture from Ludmila Courtillat--Piazza

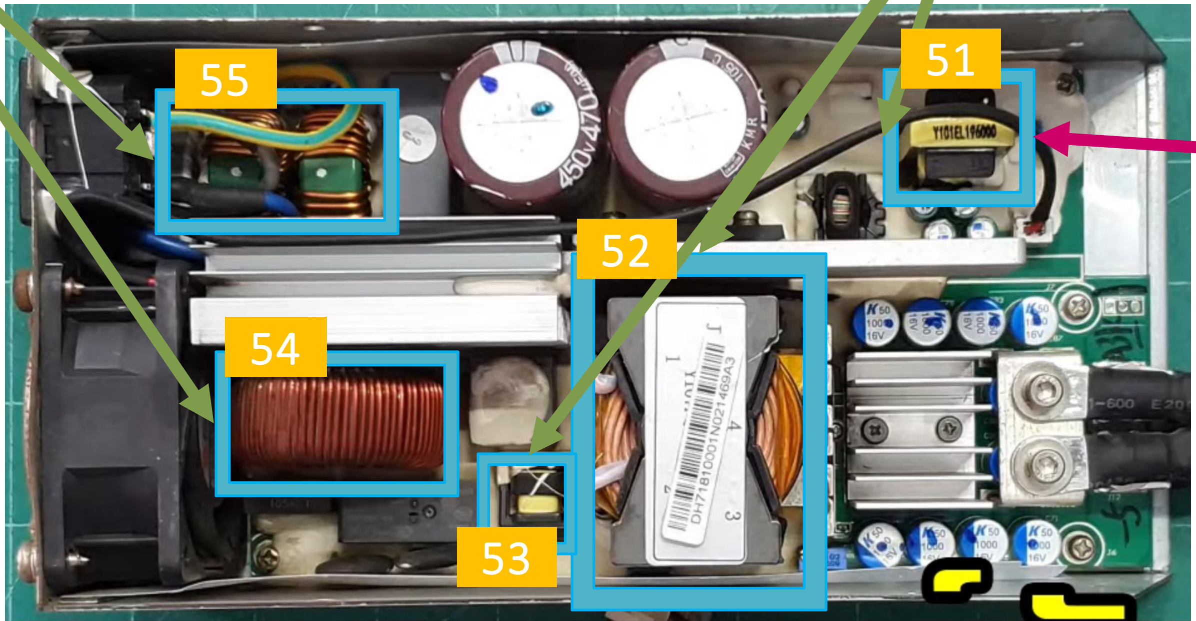


Picture from: [22]

# Power supply: Fan and Heat sinks

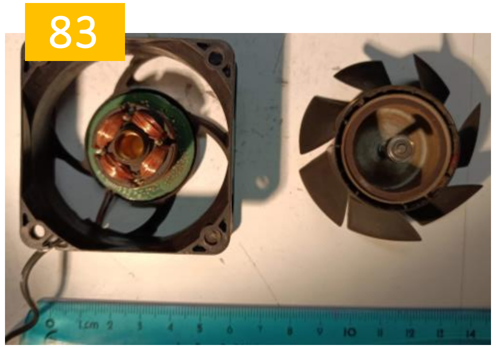


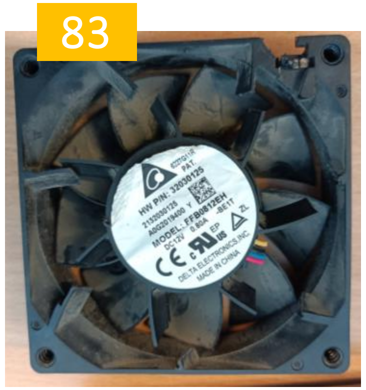


Pictures from Ludmila Courtillat--Piazza

6025 6cm DC12V 0.27A APW3++ PSU Fans Power Supply Cooling Fan PSAD16025BM

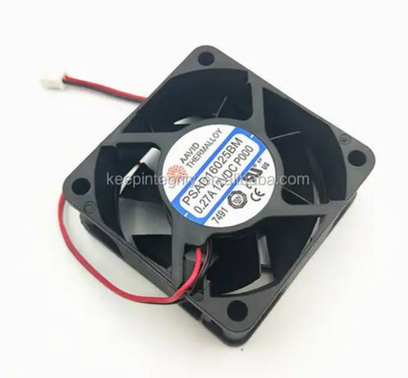

[27]

Heat sinks, metallic parts

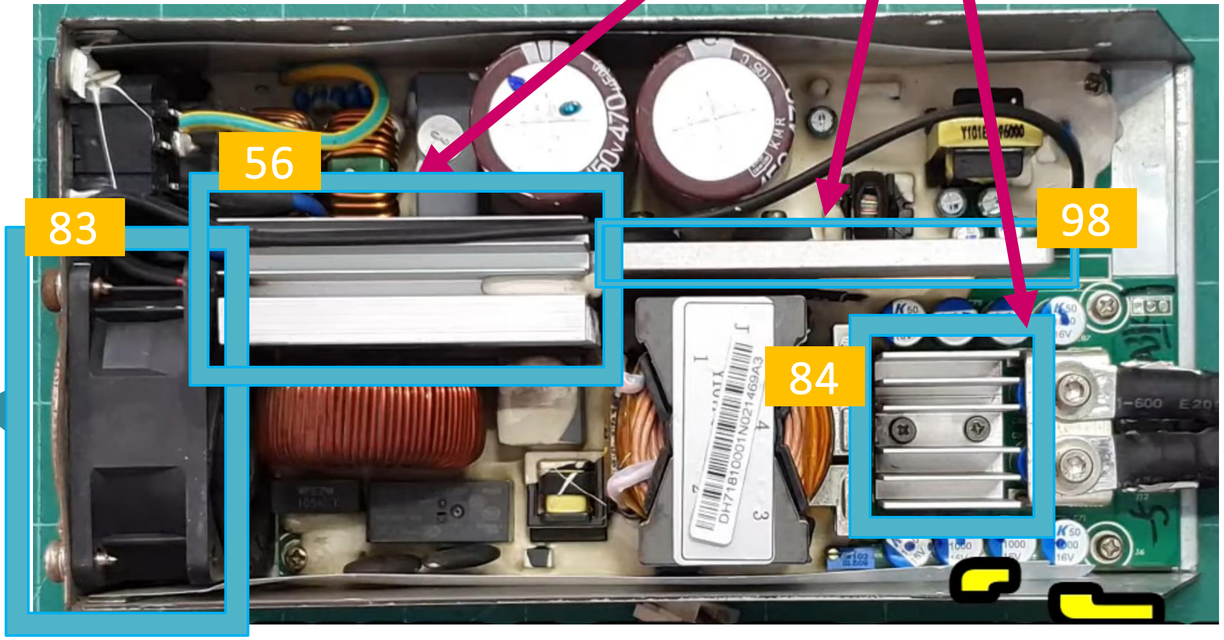


Picture from: [22]

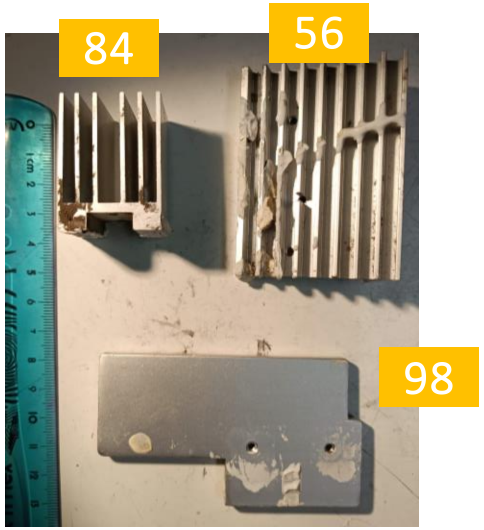


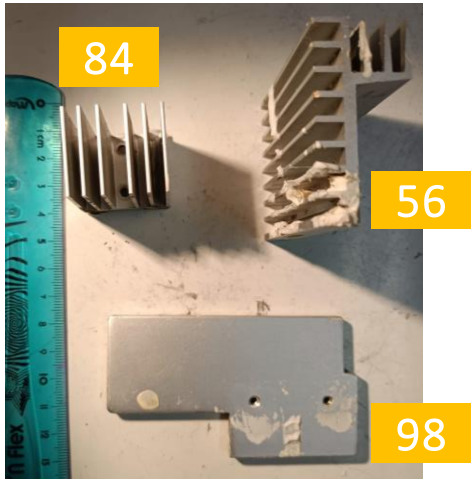


Pictures from Ludmila Courtillat--Piazza

# Power supply side 1: Others

Ring core coils 8, 30, 80g (with housing)

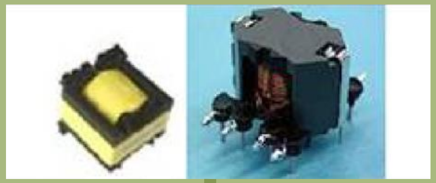

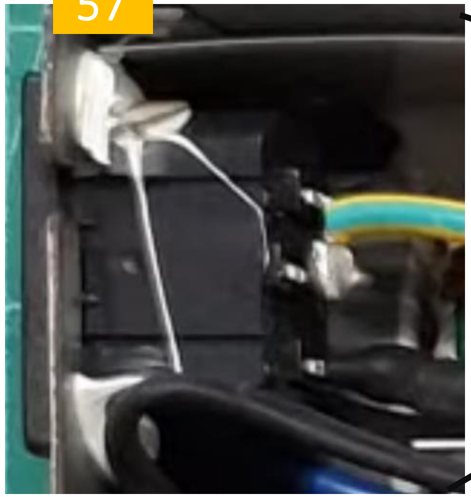


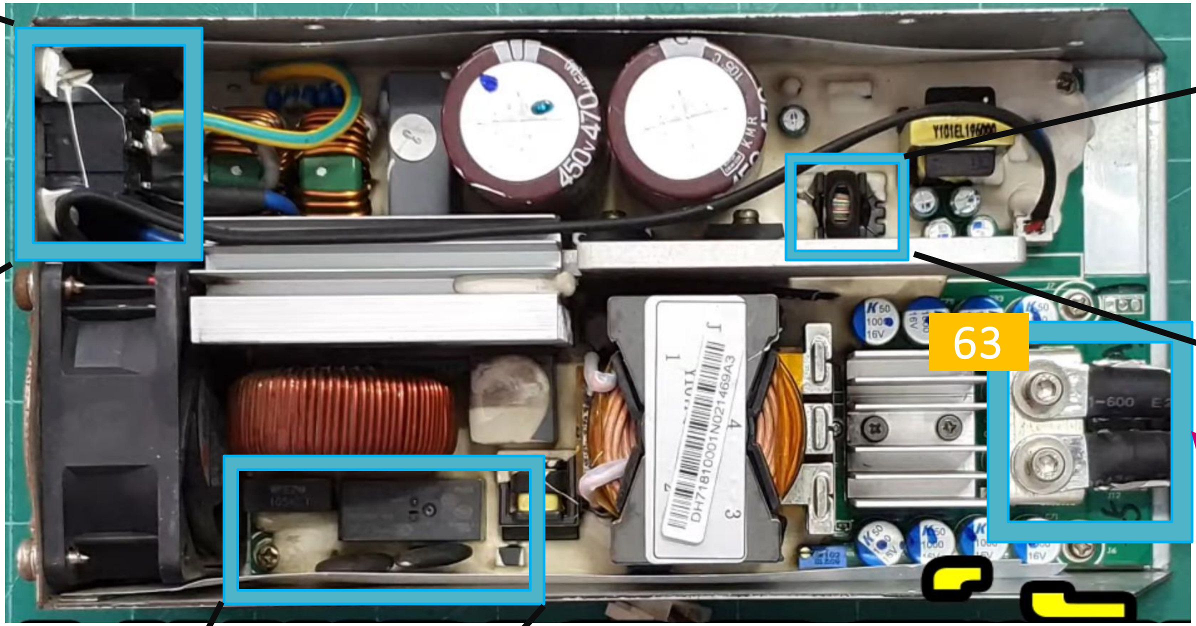

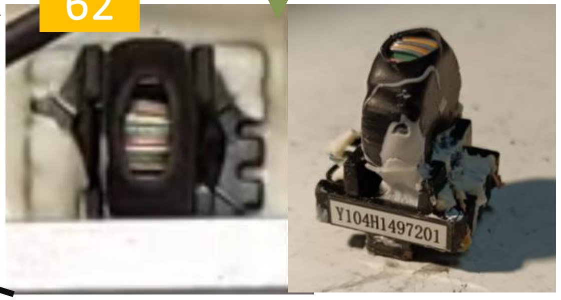


Picture from Ludmila Courtillat--Piazza

63

Connector

Connector

Inductor

Picture from: [22]

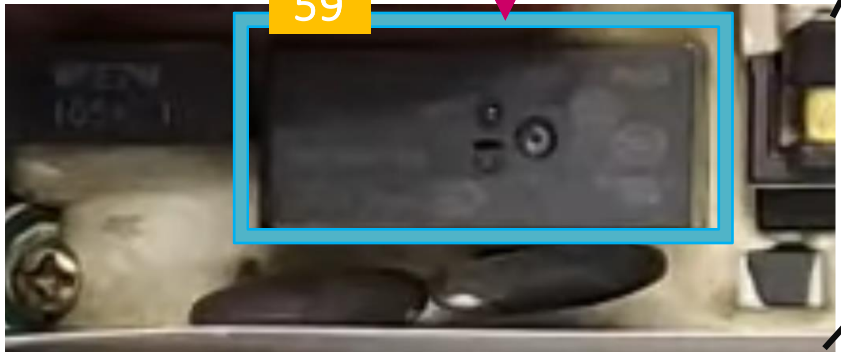


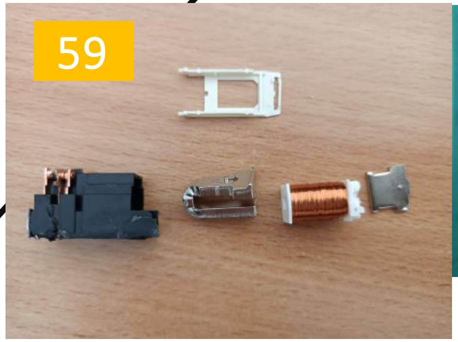


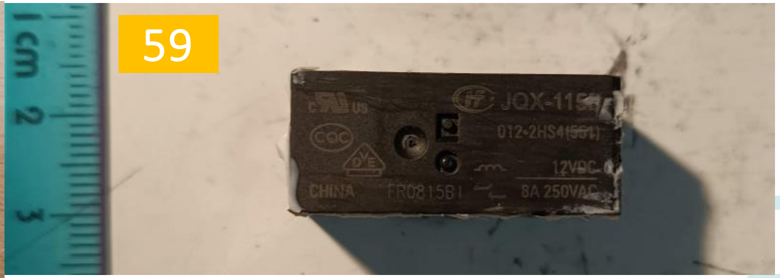


At the left, 59 dismantled - Pictures from Ludmila Courtillat--Piazza

# Power supply side 1: Components not really visible without dismantling

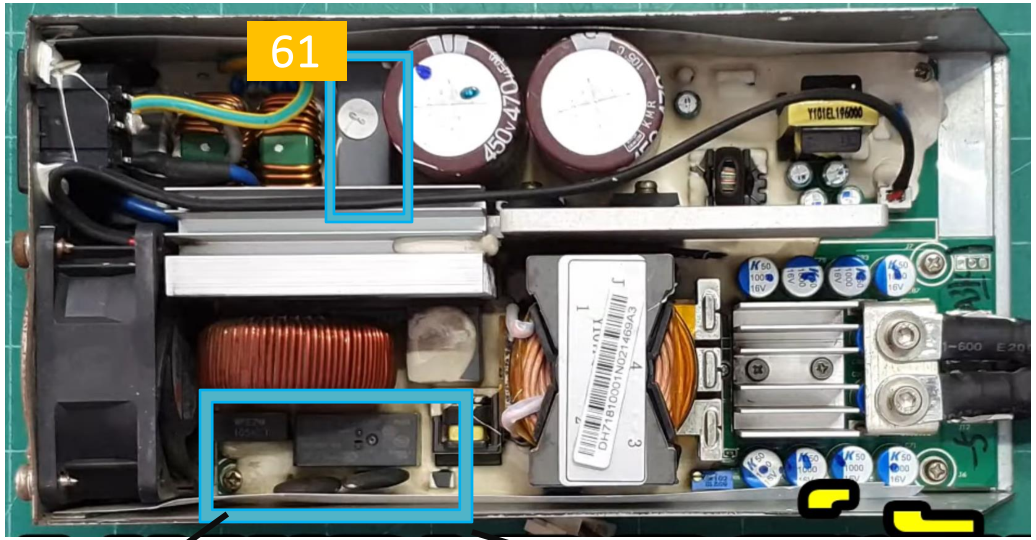


Picture from: [22]

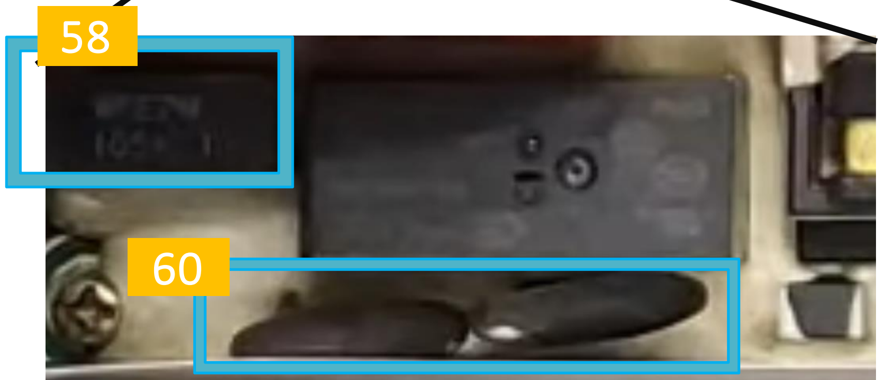


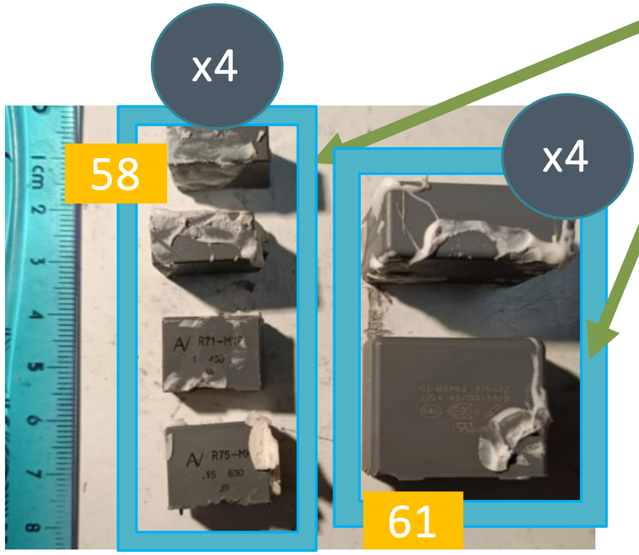


Picture from Ludmila Courtillat--Piazza

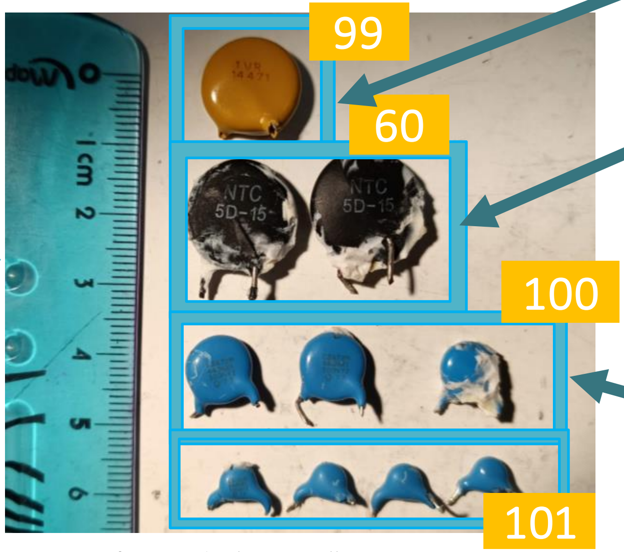


Picture from Ludmila Courtillat--Piazza

Capacitor film-capacitor boxed

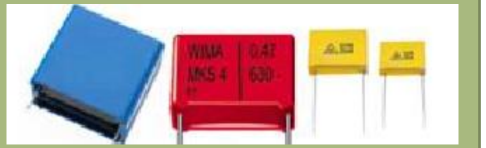

« TVR 14 471 »

Resistor Varistor TVR 14471

[51], [52]

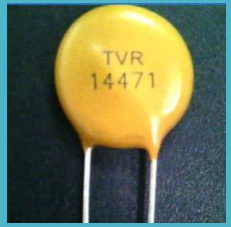


« NTC 5D-15 »

Resistor Thermistor

[53]

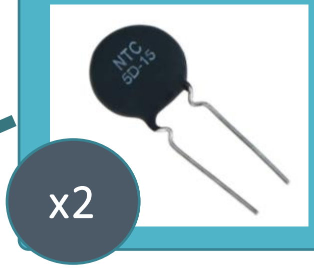


« CS472m / 440 ~X1 / 300 ~Y2 77»

Ceramic disc capacitor

[54]

x3 + x4

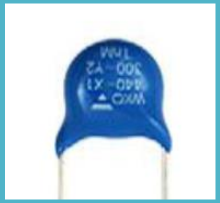

# Power supply side 1: Components invisible without dismantling (transistors)

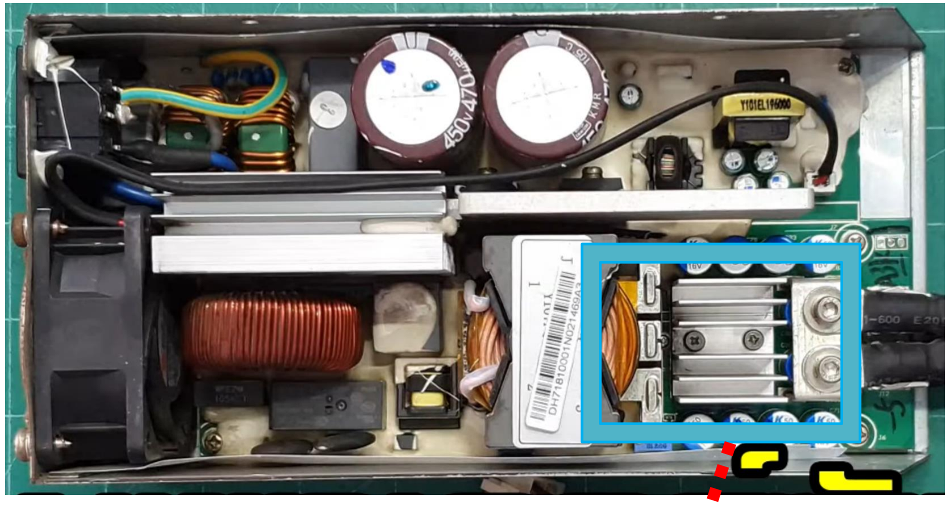

Picture from: [22]

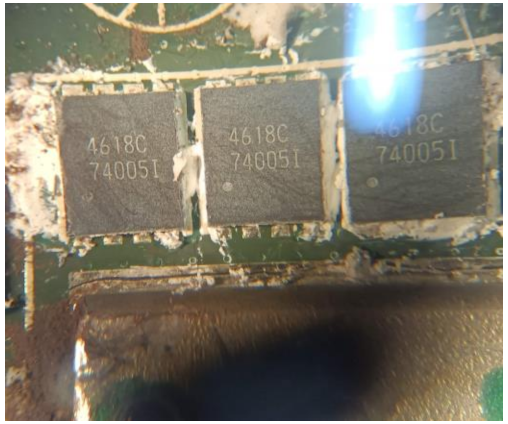

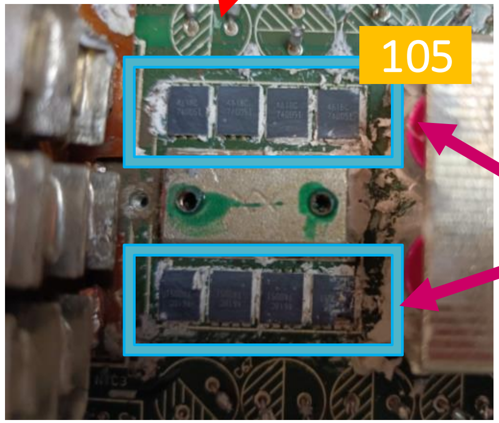

105

Transistors hiden by the heat sinks with ID 84. In the left side, view with a microscope. Pictures from Ludmila Courtillat--Piazza

x8

Transistor SMD with SOP package

102 transistor power THT/SMD SOT93/TO218 7 leads

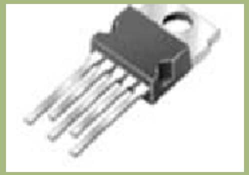

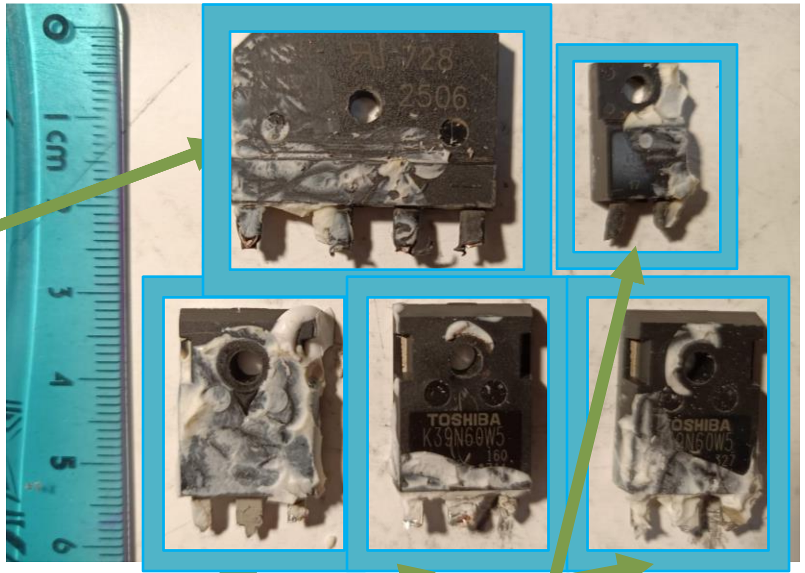

Picture from Ludmila Courtillat--Piazza

103 transistor power THT/SMD SOT93/TO218 3 leads

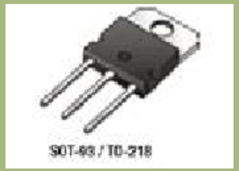


x3

Transistor THT SOT82 104

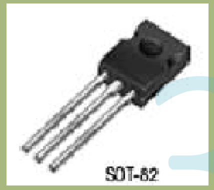

# Power supply side 2: ICs

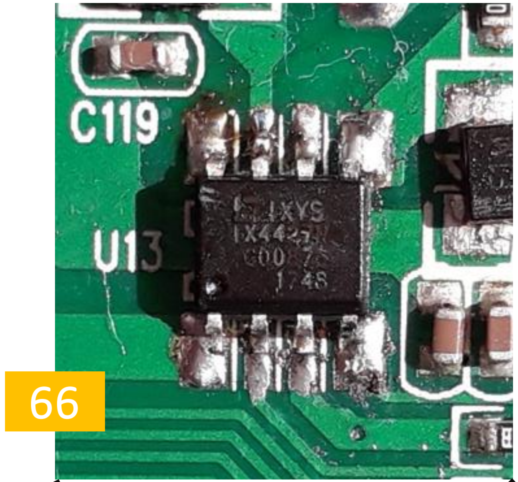


Picture from: [28]

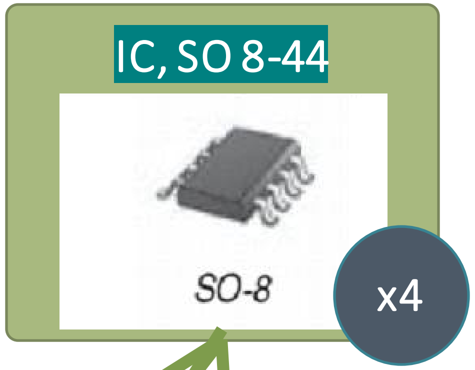


+ 11 ICs according to PCB labels

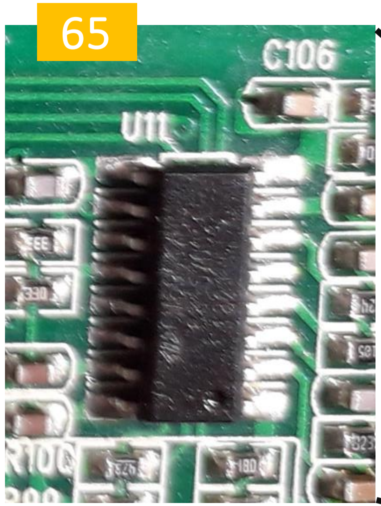


Picture from: [28]

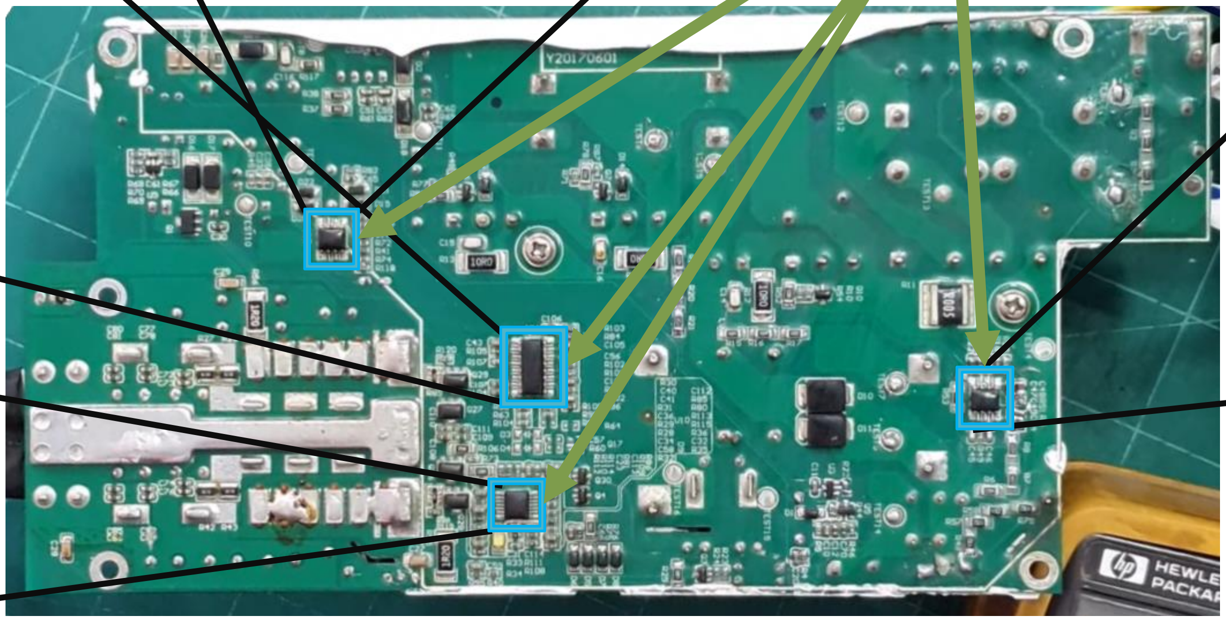

Picture from: [22]

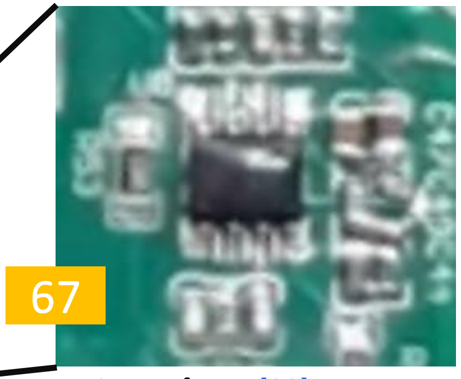


Picture from: [22]

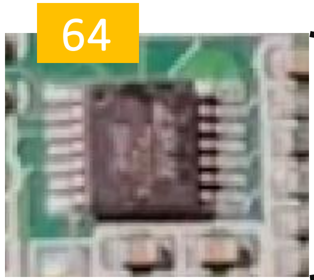


Picture from: [29]

# Power supply side 2: Resistors 1/2

69

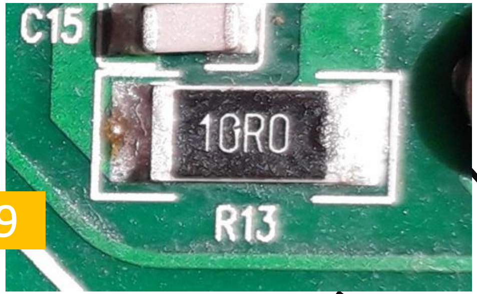


Picture from: [28]

68

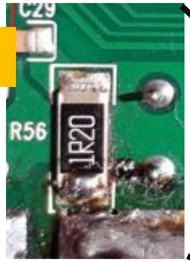


Picture from: [28]

x2

« 10R0 »

Resistor SMD

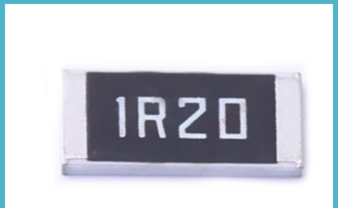


[30]

x3

« 10R0 »

Resistor SMD

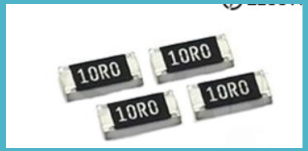


[31]

70

« 01B », « 272 », « 150 », « 330 »,...

+ > 45 small

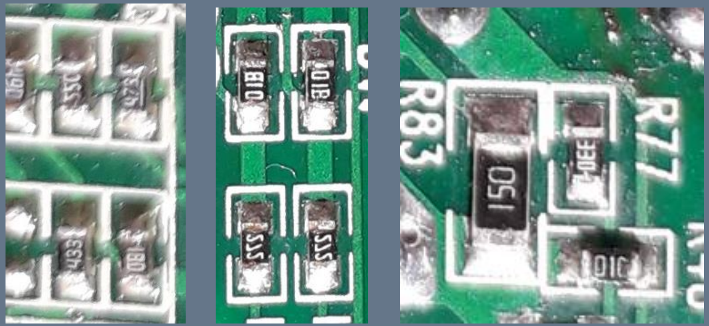


Pictures from: [28]

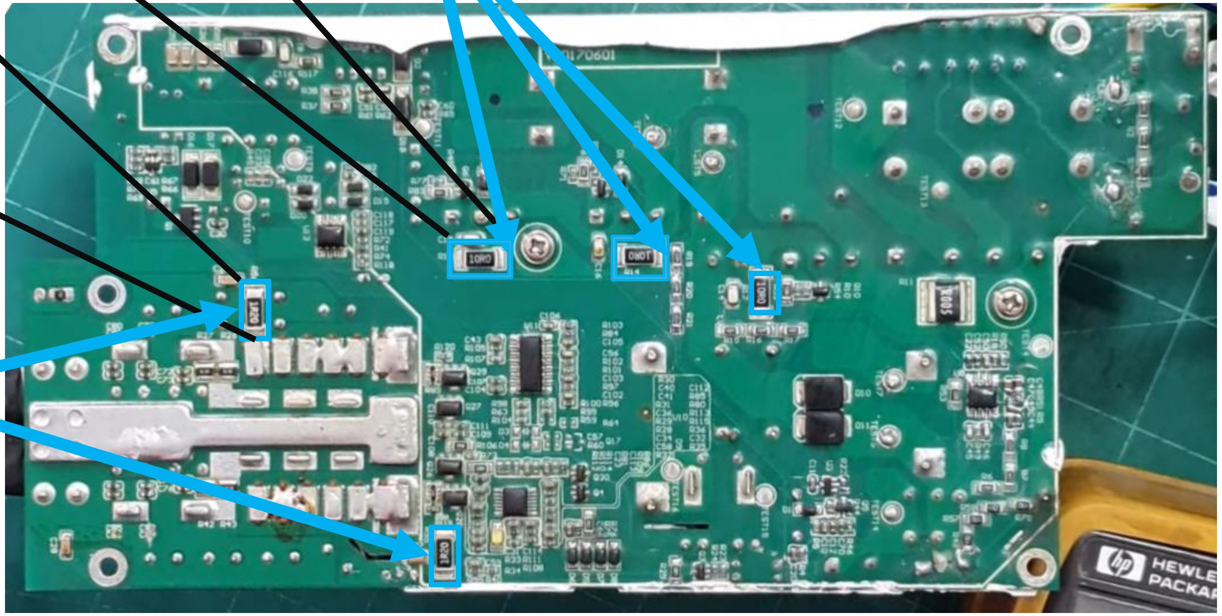

Picture from: [22]

# Power supply side 2: Resistors 2/2

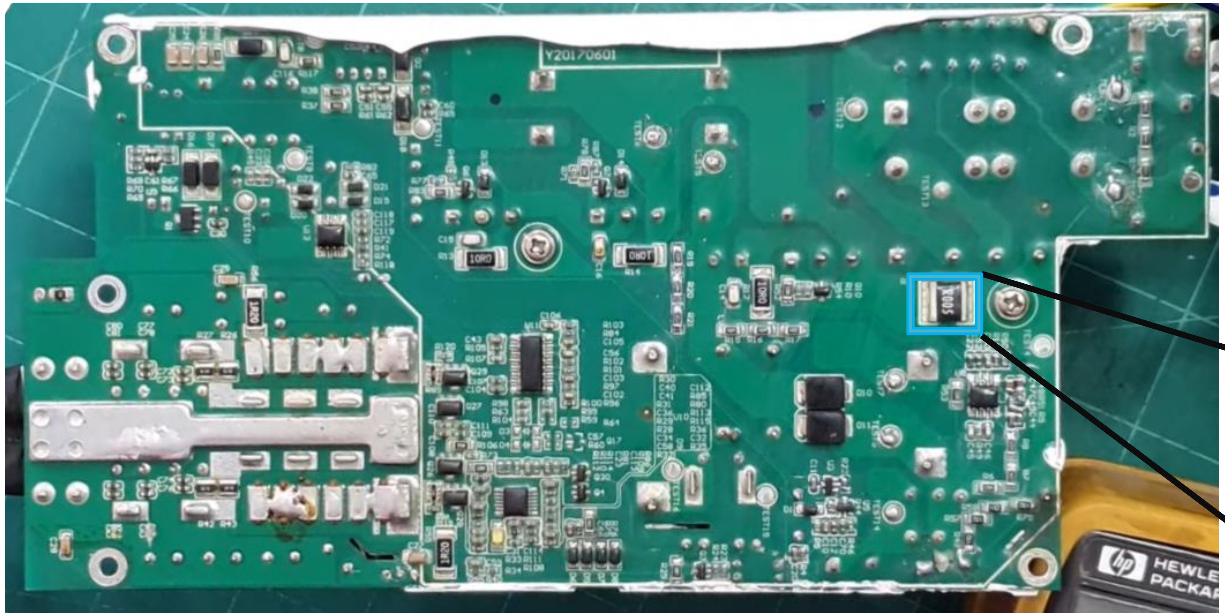

Picture from: [22]

SMD or thick film ?

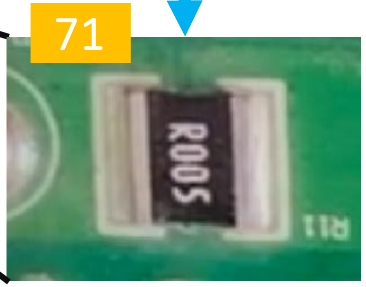


Picture from: [29]

+ >70 undifined resistors according to the PCB labels (total > 120)

# Power supply side 2: Diodes

+3 according to PCB labels (total > 22)

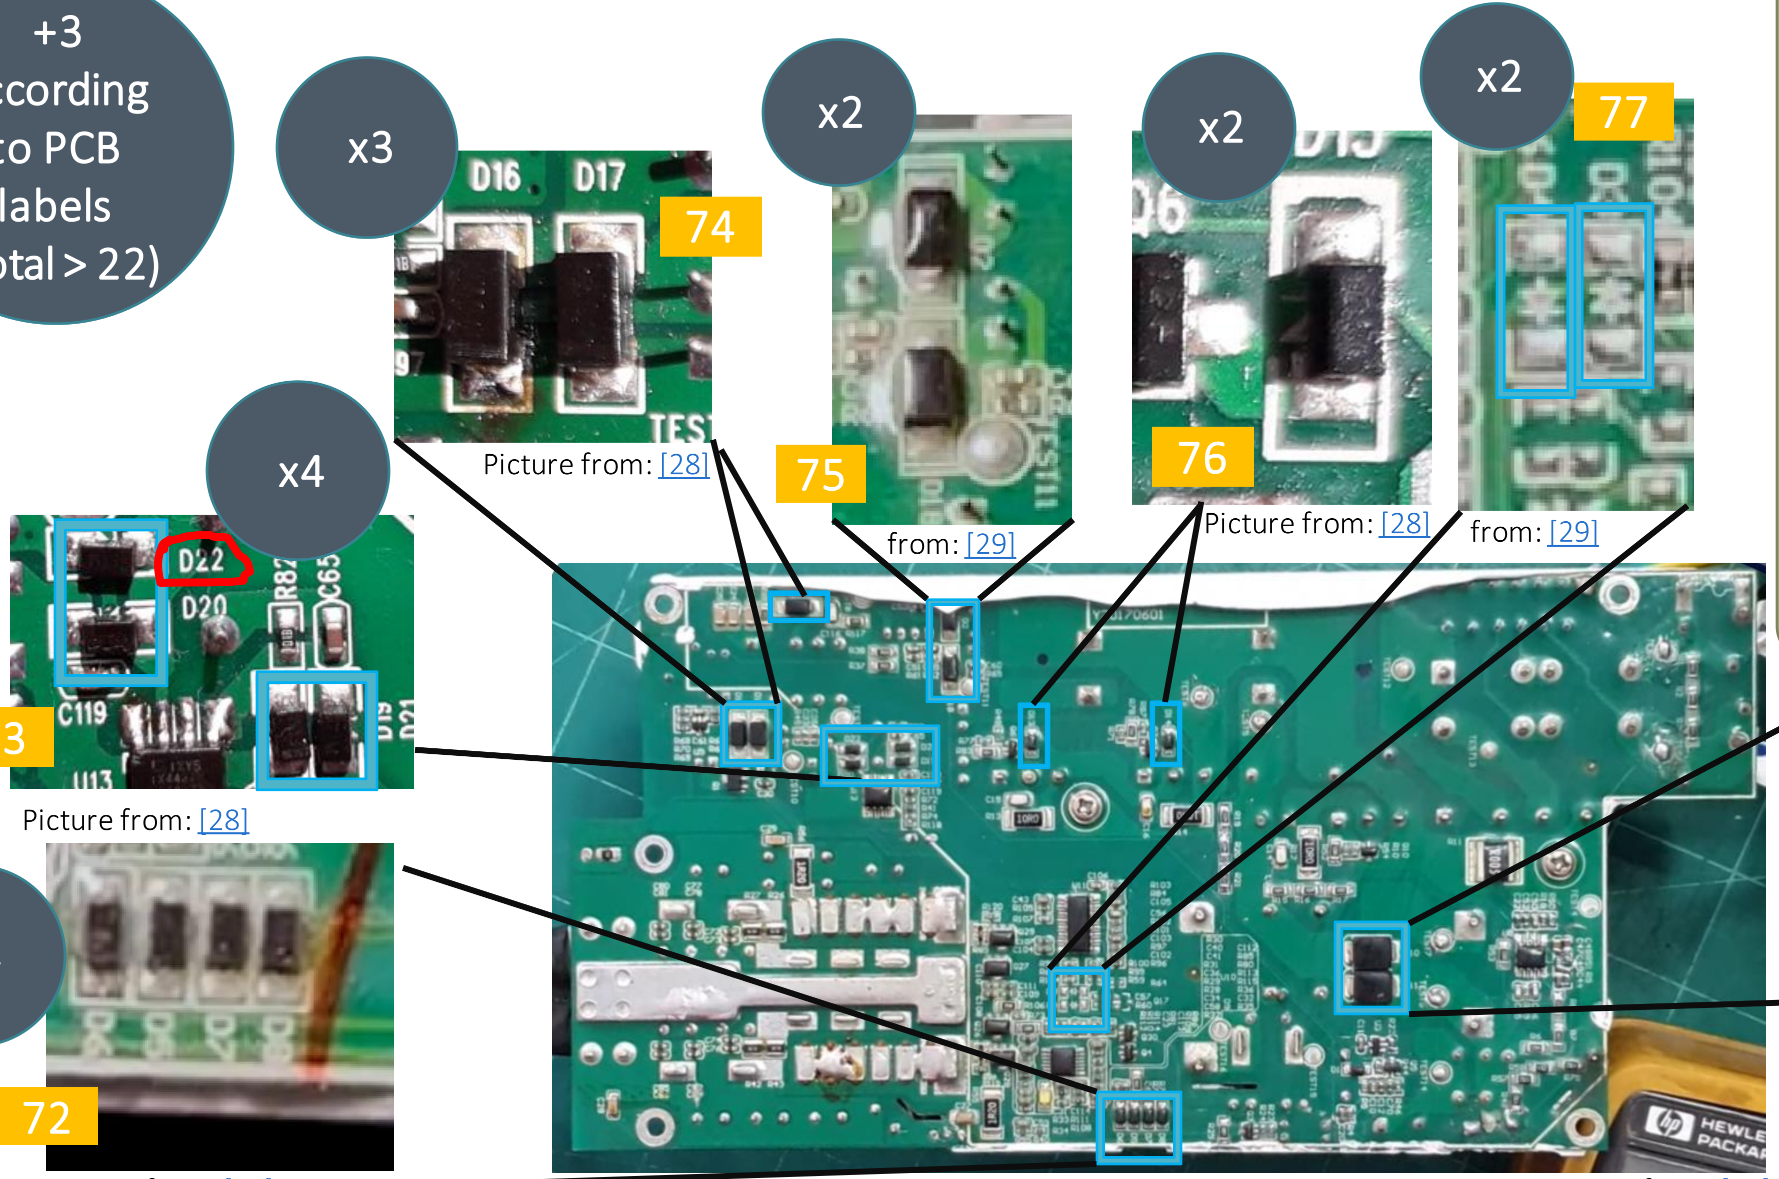


Picture from: [28]

from: [29]

Picture from: [28]

from: [29]

Picture from: [28]

Picture from: [29]

Picture from: [22]

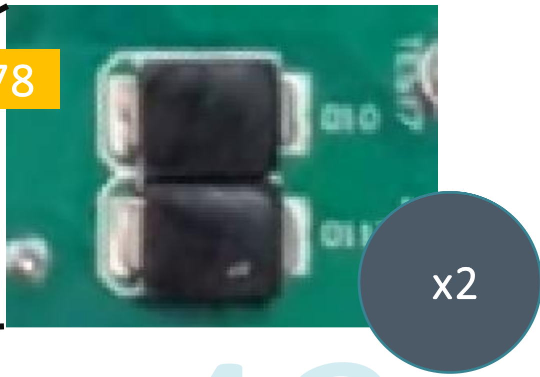


Diodes:

72, 73, 74, 75, 76, 77

Diode signal DO214/219

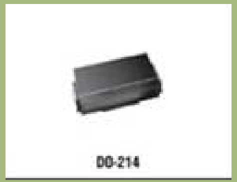


78

Diode signal SOD 123/323/523

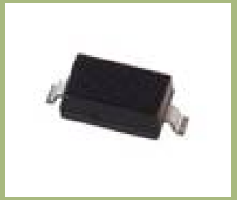

# Power supply side 2: Transistors

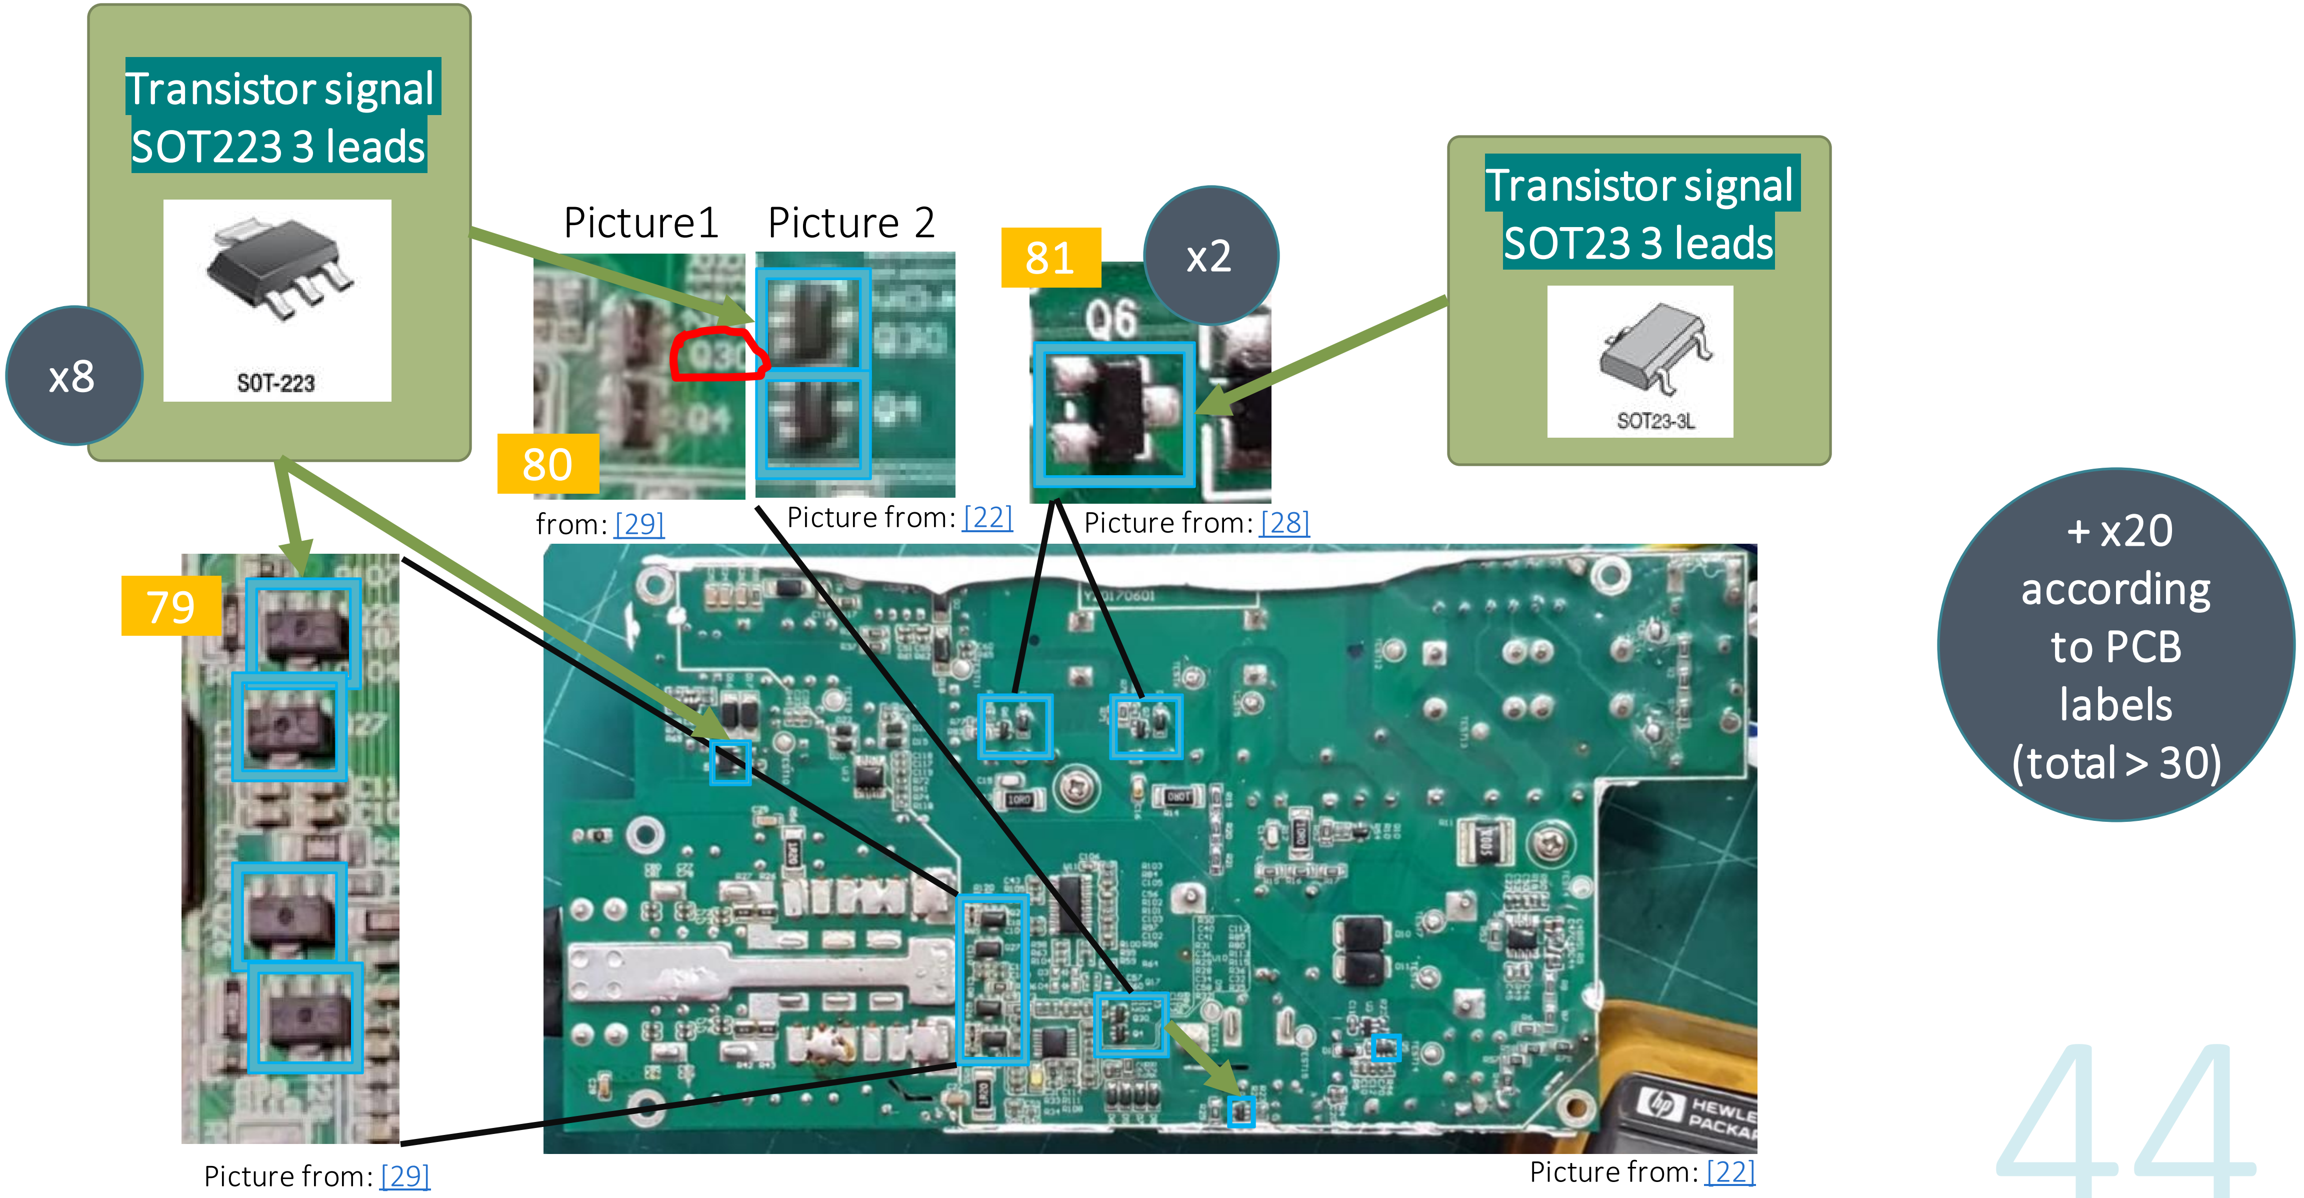

# Power supply side 2: Capacitors

82

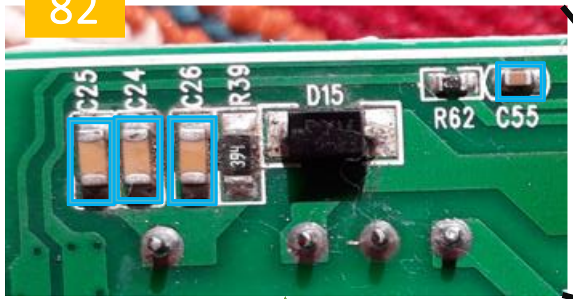


Picture from: [28]

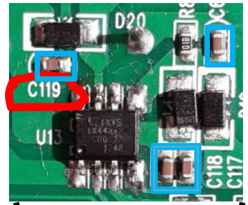


from: [28]

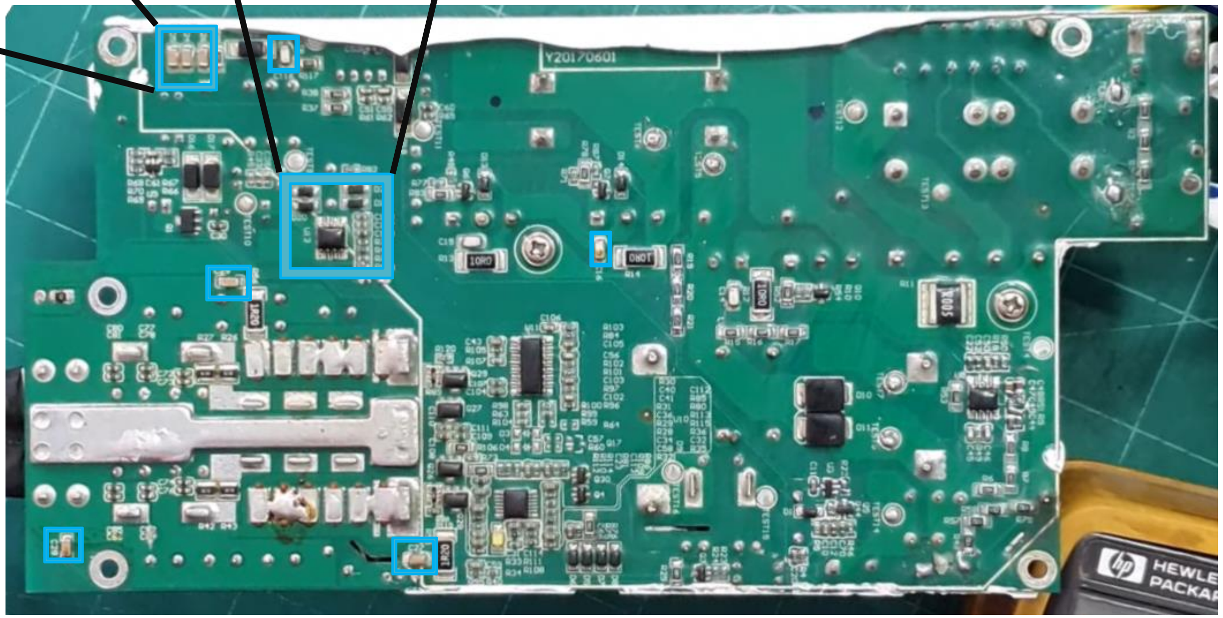

Picture from: [22]

~ x112
Big:
~ x7

Capacitor ceramic MLCC

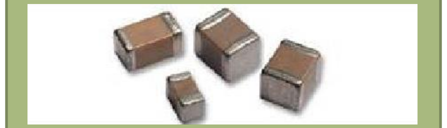

# Casing

# Casing

106

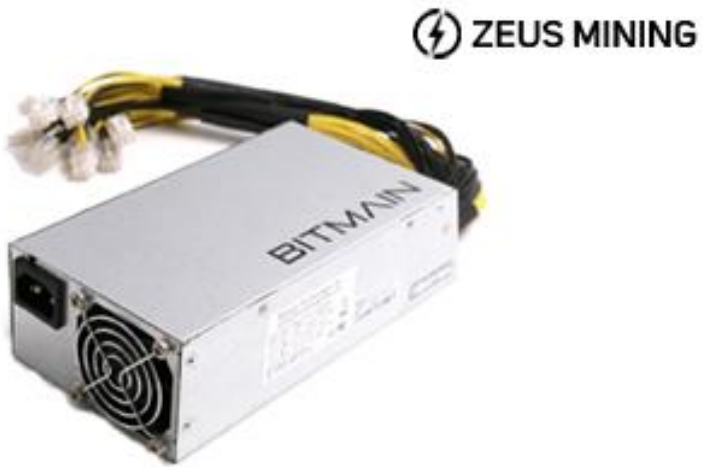


Picture from: [55]

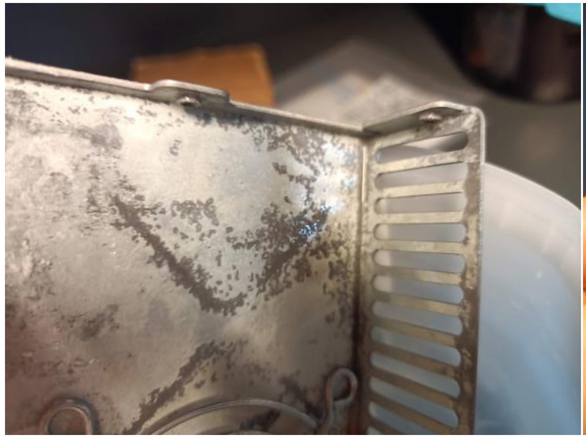

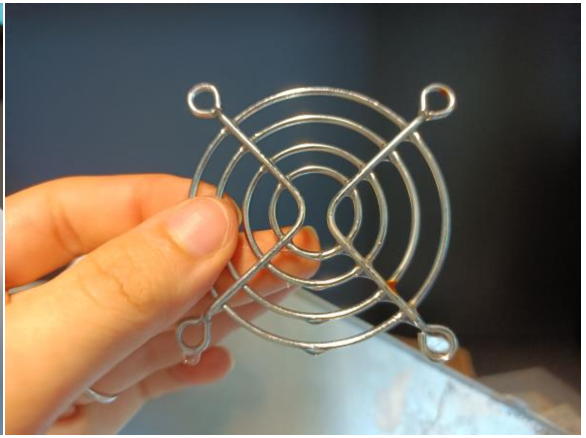

Picture from Ludmila Courtillat--Piazza

Here we manipulated the casing of the power supply

- Oxidation with water and salt: Yes
- Mass: 625g
- Magnetic properties: Yes

-> assumption: this is steel (but not stainless)

Approximation of the mass of the casing of the Antminer S9:

- Total mass of the miner: 4200g
- Control board: 100g
- Hashboard (x3)
  - without heat sinks: 50g –250g (visual estimation)
  - Heat sinks: ~ 64 x 4,5g (upper side) + 63 x 3g (lower side)
- Fan: ~300g according to various sources: [60] [61][62] [63]

Hence, we can estimate that the weight of the casing is between 1,453 and 2,343 kg.

# Fan

# Fan

89

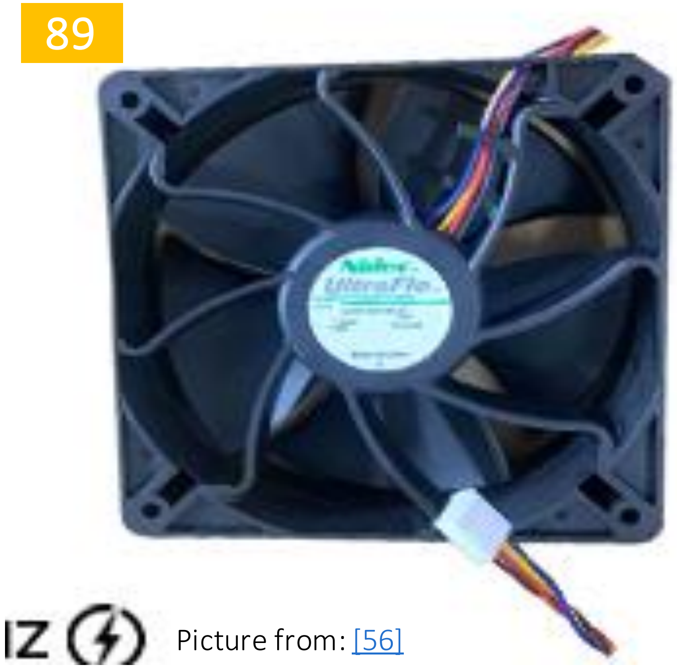

Picture from: [56]

Used in GaBi for plastic: **Linear low-density polyethylene**

**Because of an inscription on a proxi fan that corresponds**

| Code | Symbole de recyclage | Désignation IUPAC | Désignation courante | Famille |
|---|---|---|---|---|
| PE[4] :<br>PEBD (en anglais LDPE)<br>PEBDL (en anglais LLDPE)<br>PEHD (en anglais HDPE) | 4 (PEBD)<br>7 (PEBDL)<br>2 (PEHD) | PE : poly(méthylène) | polyéthylène basse densité (PEBD)<br>polyéthylène à basse densité linéaire (PEBDL)[5]<br>polyéthylène haute densité (PEHD) | polyoléfine |

[32]

# Cables

# Power cable

1,5 m
Source: [34]

28

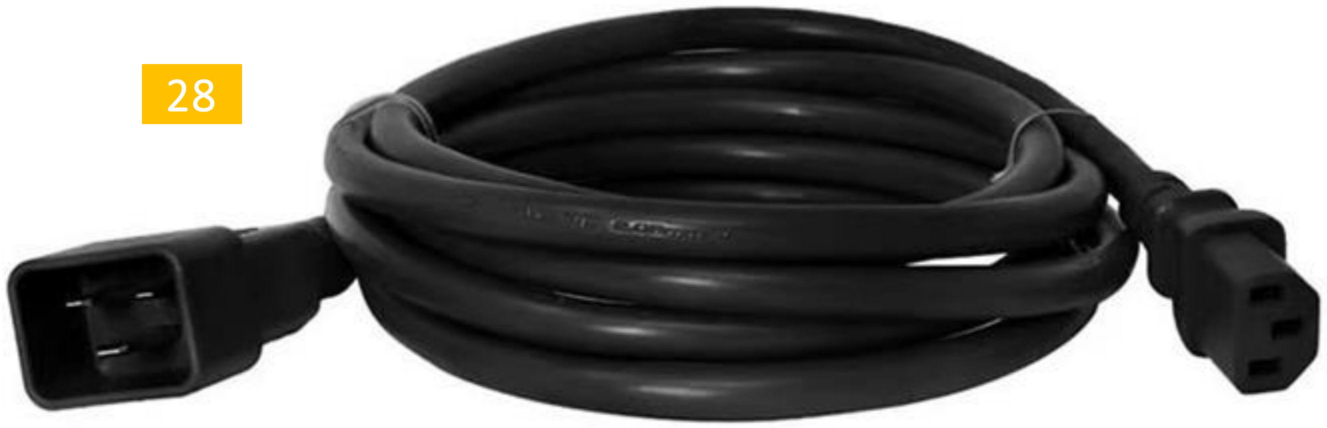

Picture from: [33]

# Main Fan Cable

85

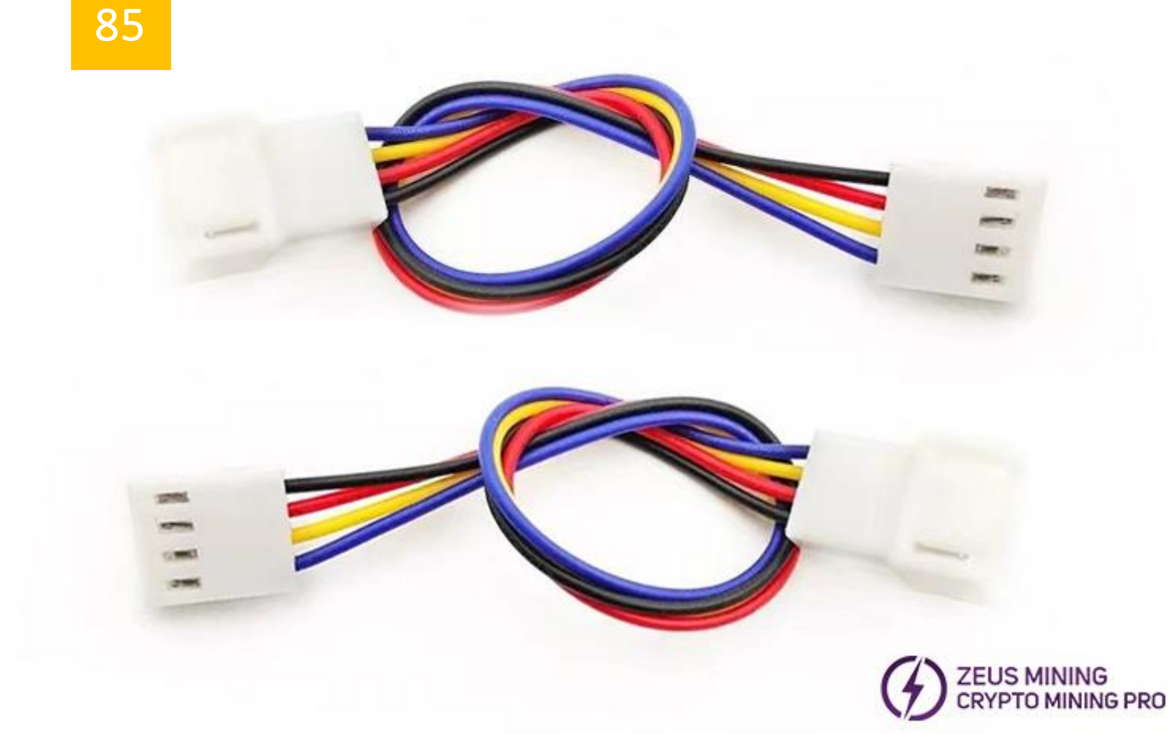


Picture from: [35]

# Power supply cable (with PCI-e power connectors)

x 2

86

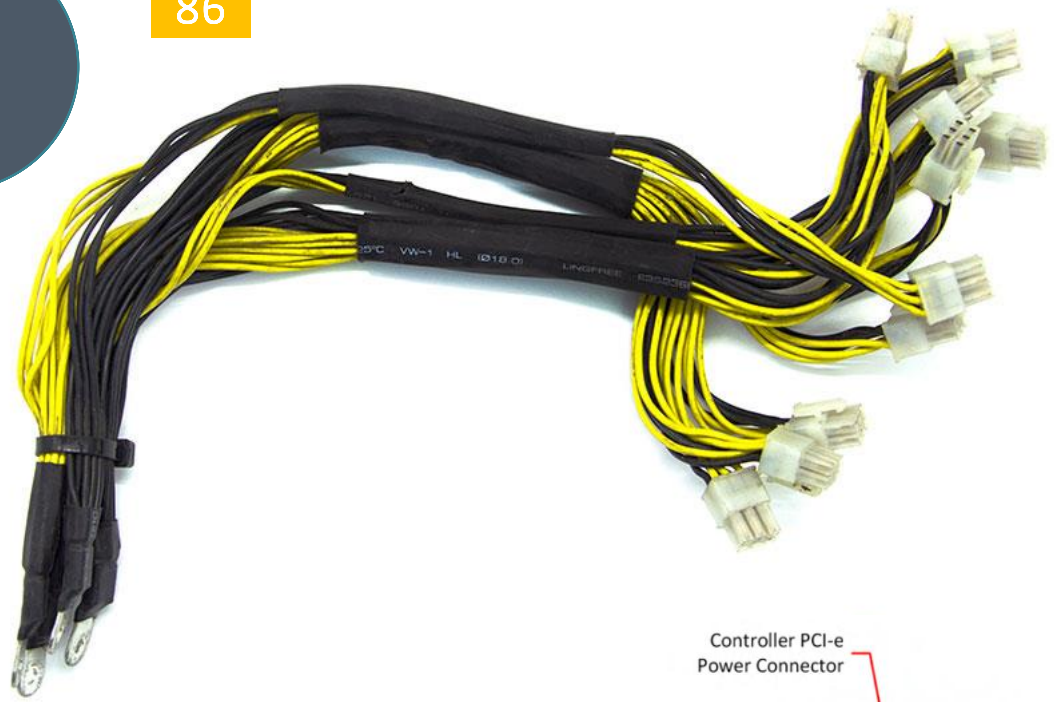

Picture from: [36]

Length: 40 cm

Each cable contains 5 groups of thin cable that end in an outlet.

Each of these groups contains 6 thin cables connected to the outlet. In total, there are 5x6x0.4=12m of thin cable.

We measure the thin cable to weigh 7g/m.

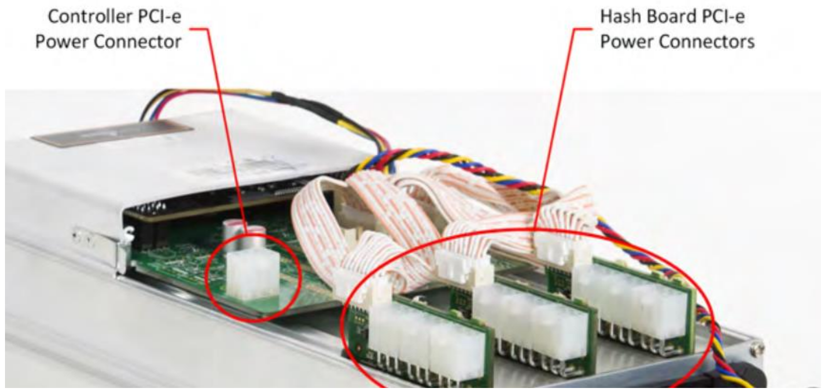


Picture from: [9]

# Data Cable

19 cm
Source: comparing [37] and [9]

87

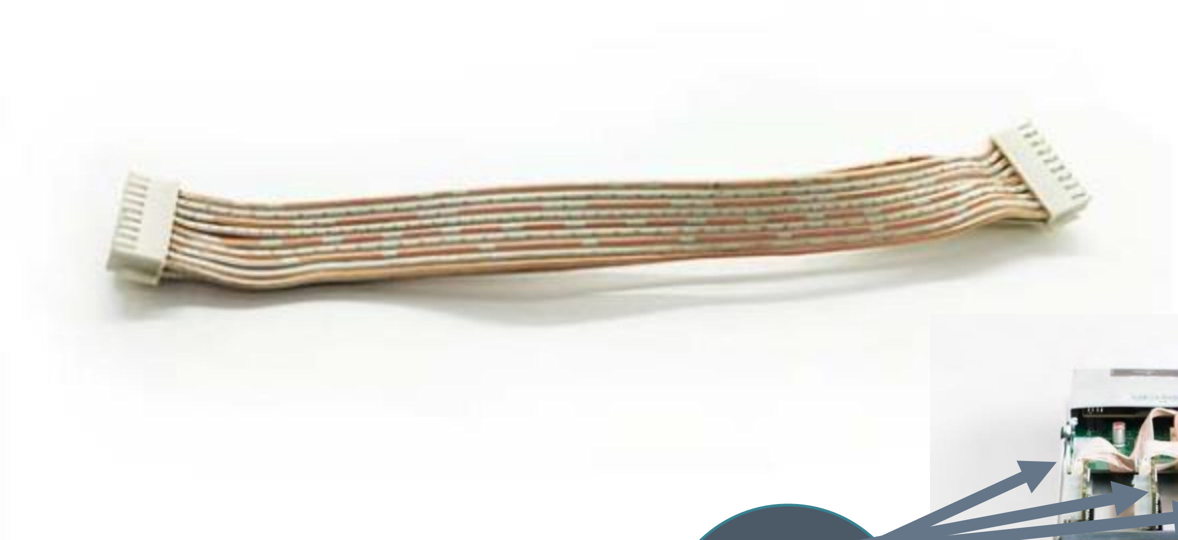

Picture from: [37]

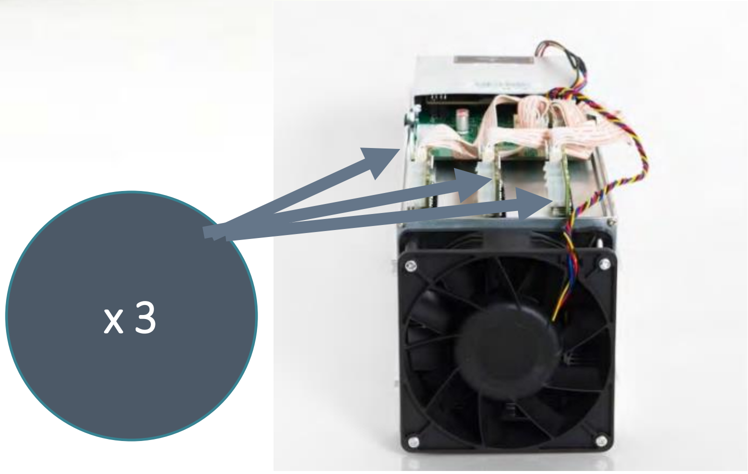


Picture from: [9]

# Power Supply Fan Cable

88

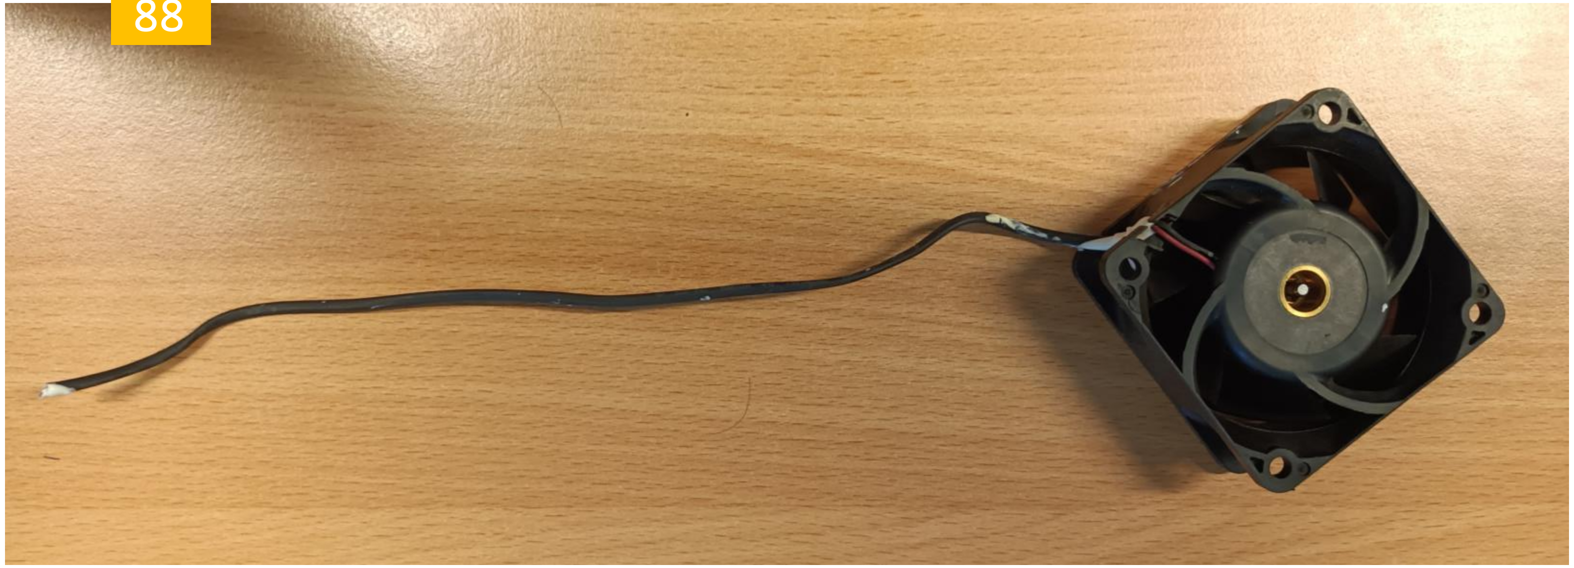

Picture from: Ludmila Courtillat--Piazza

20 cm

# Assembly

# Solder Paste

- Solder paste SnAg3Cu0.5 (SAC-Lot) assumed, because this is one of the most frequently used.
- Volume weight: 7,38 $g/cm^3$, source: [58]
- Thickness of the solder paste: ~ 0.1mm according to [59]

$$
\begin{aligned}
& l \times L \ [mm^2] && \text{[surface of ICs]} && (0)\\
& \times 0.01 \ [m^2] && \text{[conversion]} && (0)\\
& \times h \ (0.1mm) -> \times 0.01 \ [cm^3] && \text{[volume of solder paste]} && (0)\\
& \times \nu \ (7.38g/cm^3) \ (g/cm^3 \times cm^3 \sim g) && \text{[weight of solder paste]} && (0)\\
& \times 0.001 && \text{[conversion]}(kg) && (0)
\end{aligned}
$$

then the quantity of solder paste is $\boxed{7.38 \times 10^{-7} \sum_{i \in ICs} L_i \times l_i \times N_i}$

with $N_i$ the number of pieces of the ICs $i$, $L_i$ its length and $l_i$ its width.

# Transport

During the production

# Transport

We have no information about the locations of the manufacturing of the different components. As a consequence,
- We used the "market for" model in ecoinvent, that include transport for each process.

- In Sphera LCA, we reproduced the same assumptions than those made in the market for model in ecoinvent: for each process,

- 20km by truck
- 20km by train

# S19 Pro

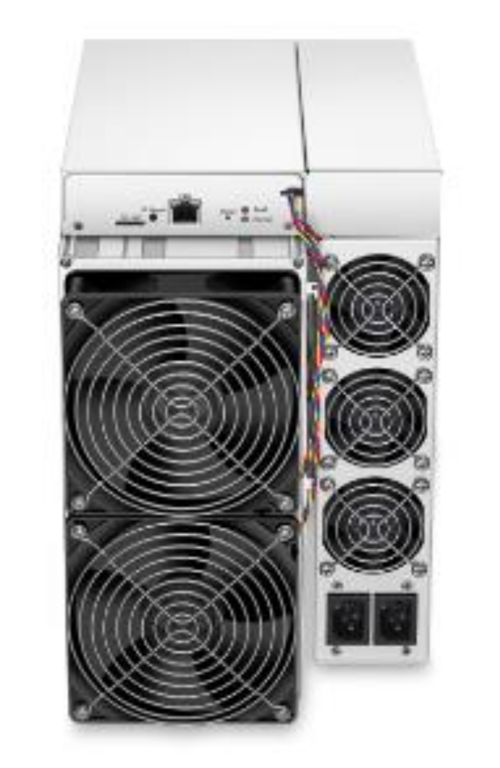

Picture from: [57]

# Hashboard

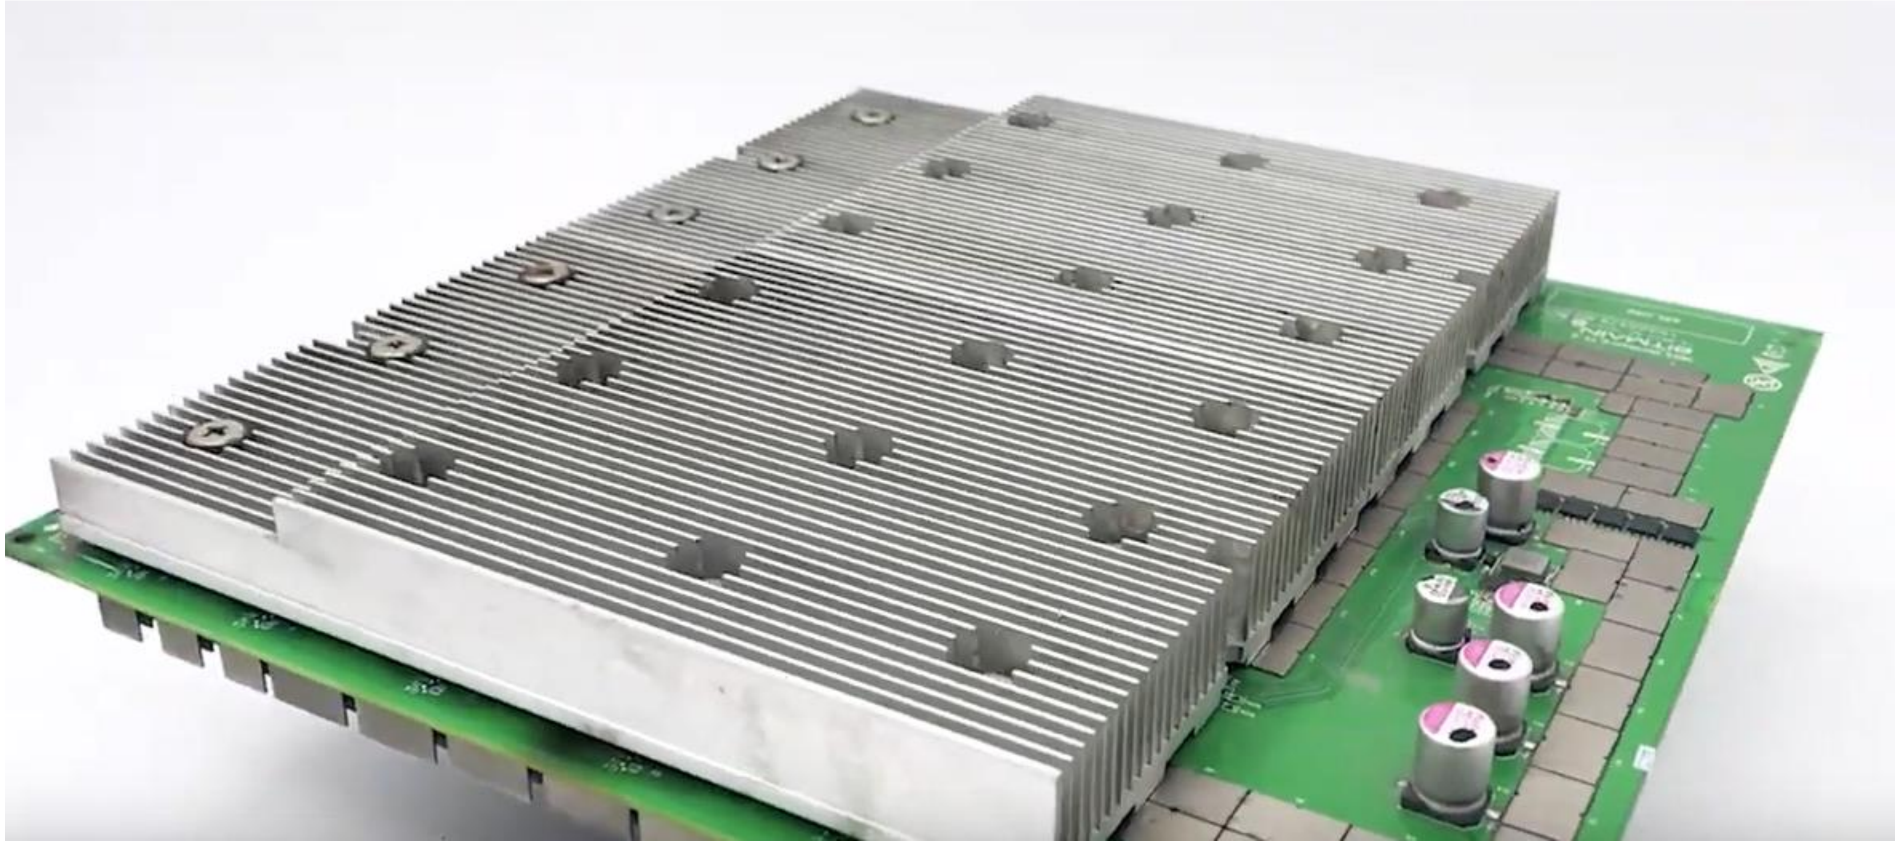

Picture from: [38]

# Hashboard

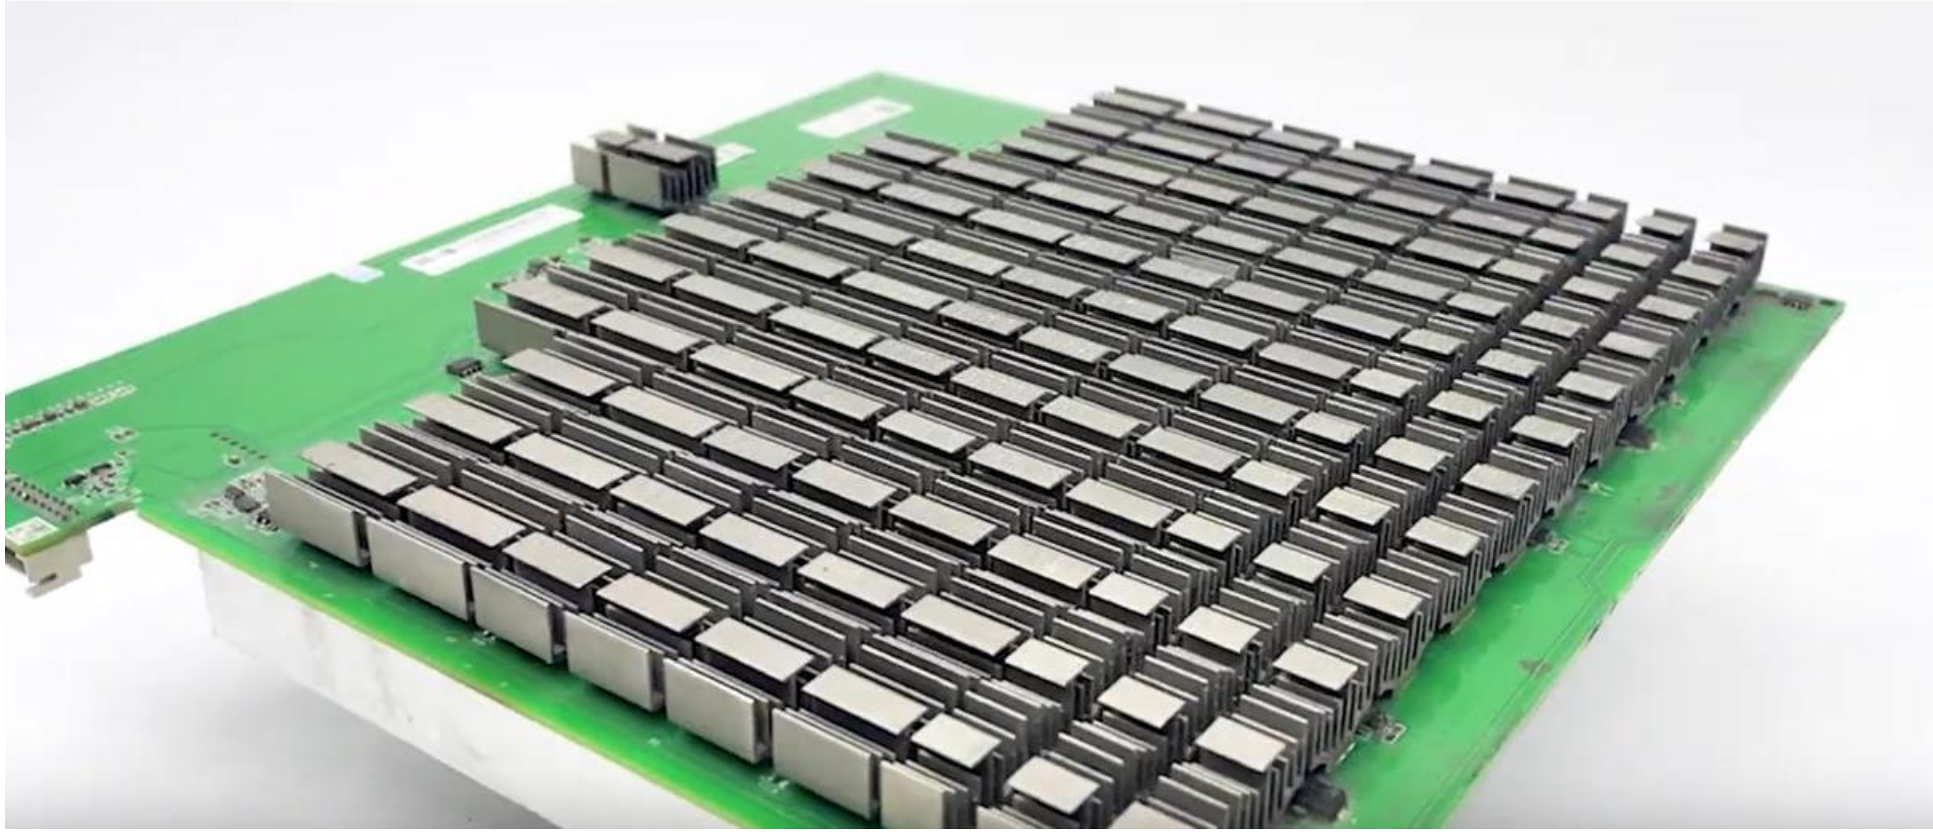

Picture from: [38]

# Hashboard

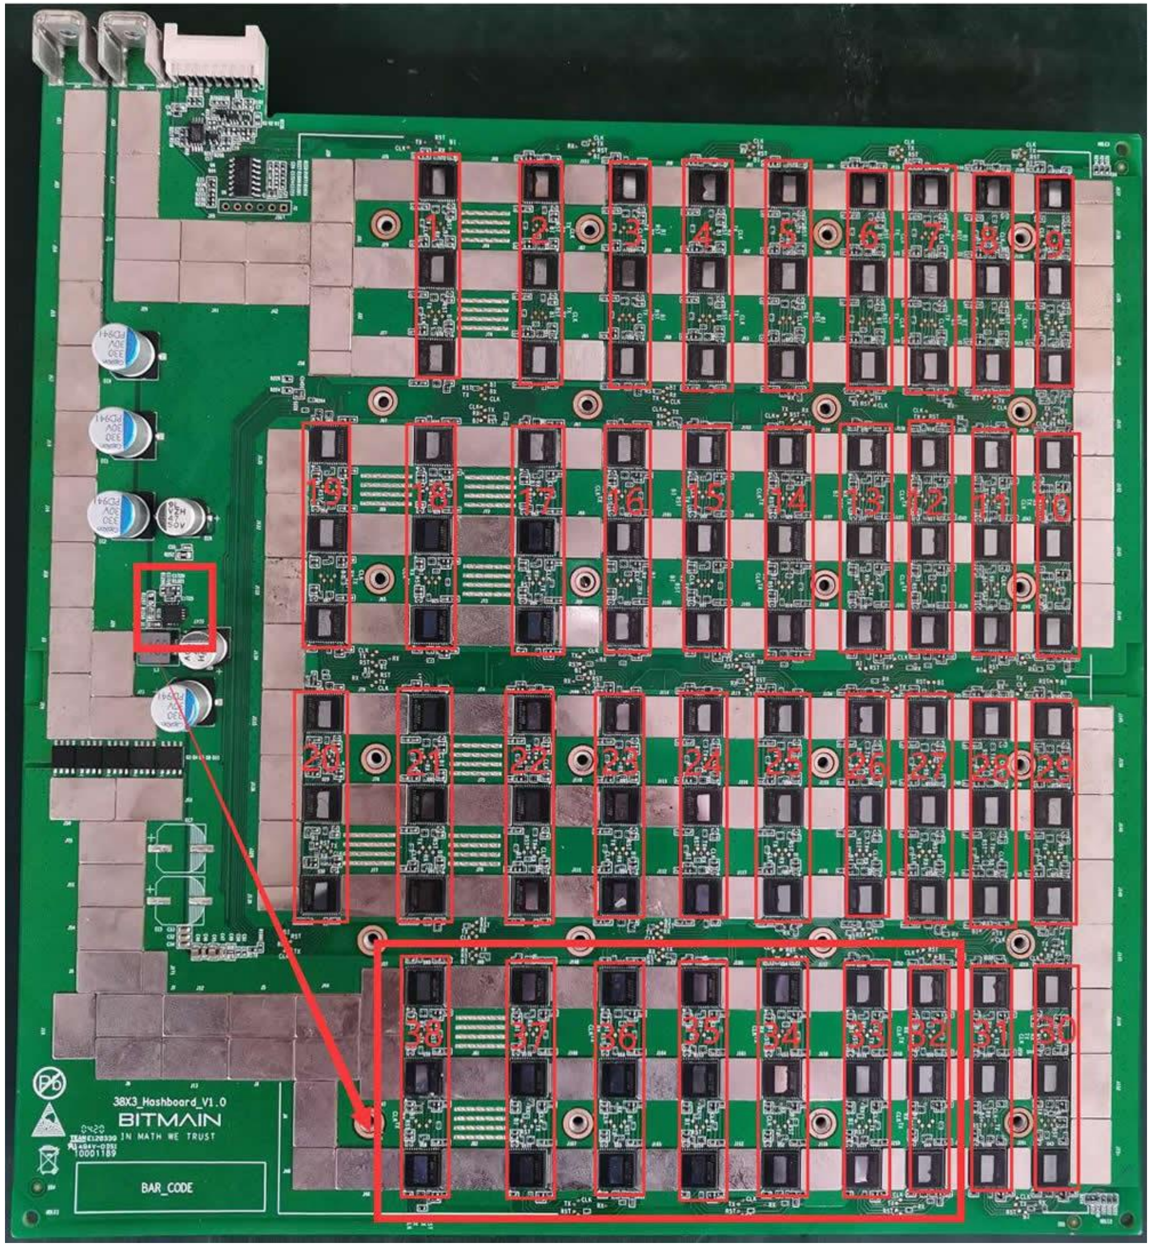


Picture from: [39]

# ASICs

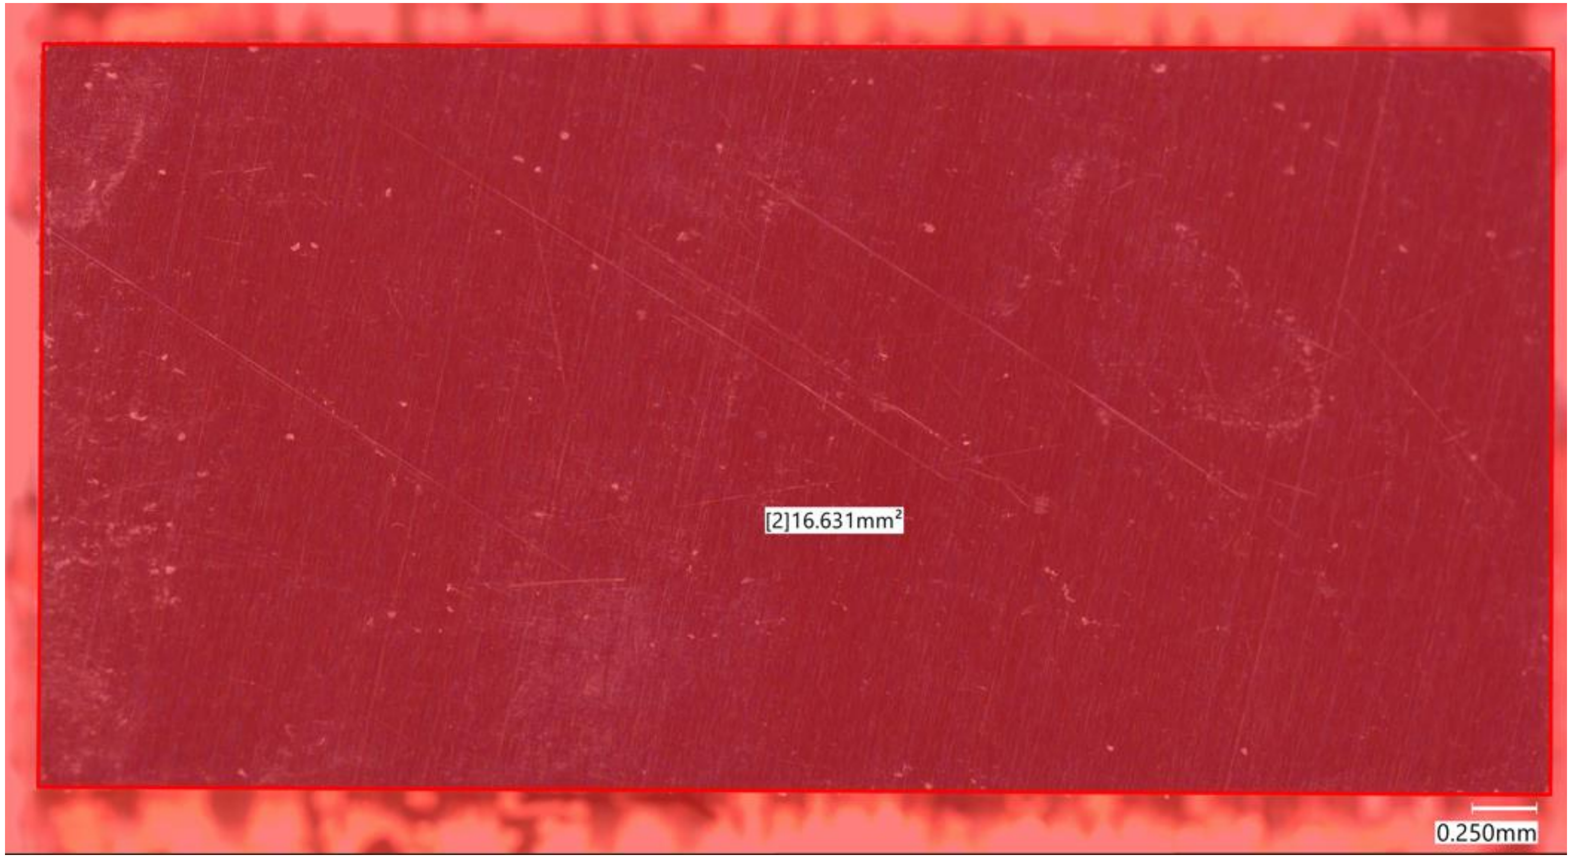


Picture of the die made with a precise microscope after package removing. The precise area is determinated with help of the computer.

Picture from: Thibaut Heremans, Thibault Pirson, Ludmila Courtillat--Piazza

# Power Supply APW12: Electrolytic capacitors

x4

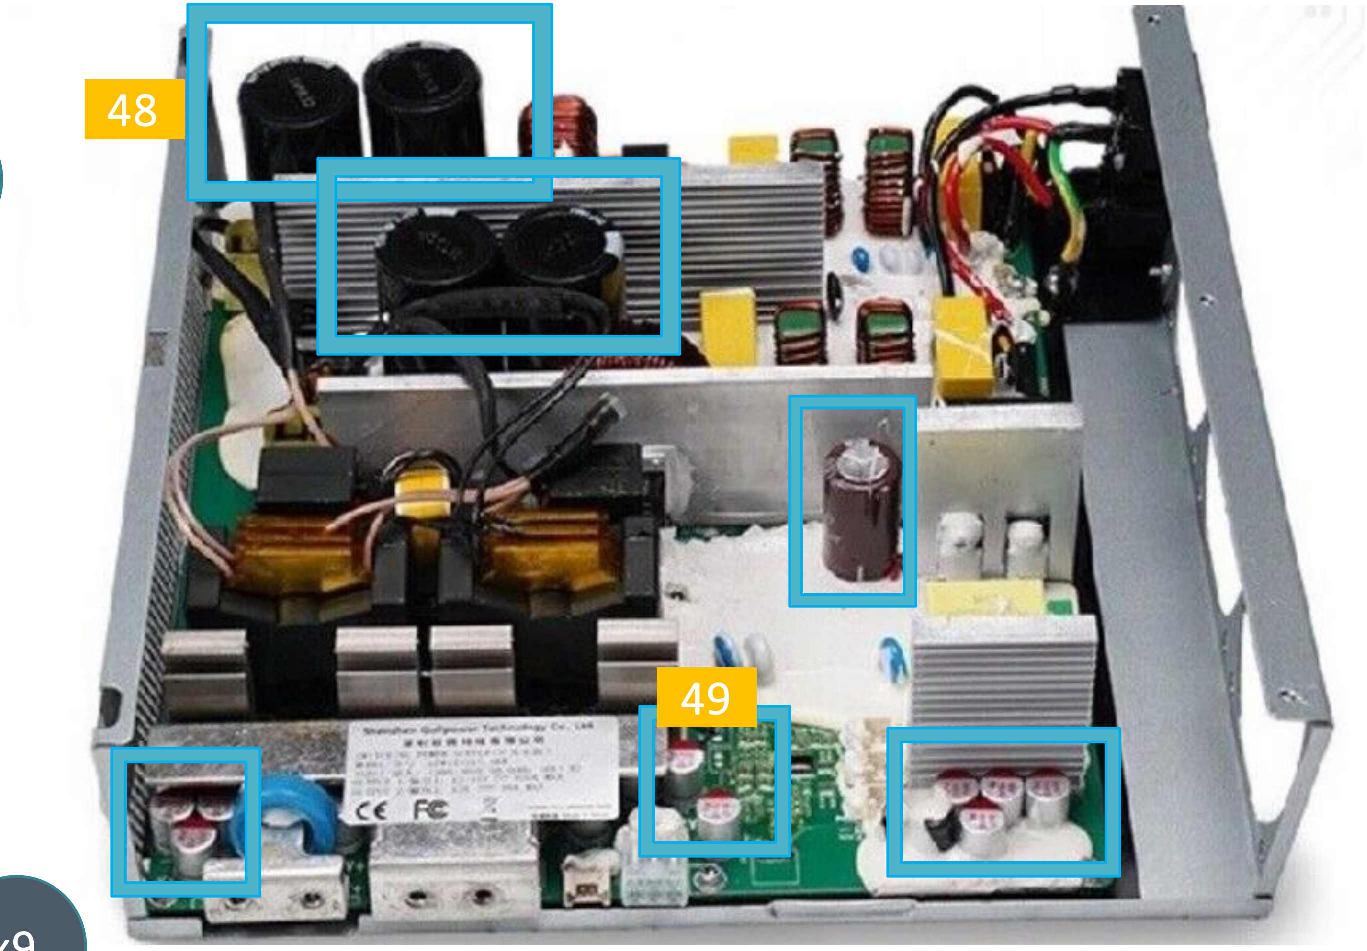


x9

Picture from: [40]

# Power Supply: ring core coils

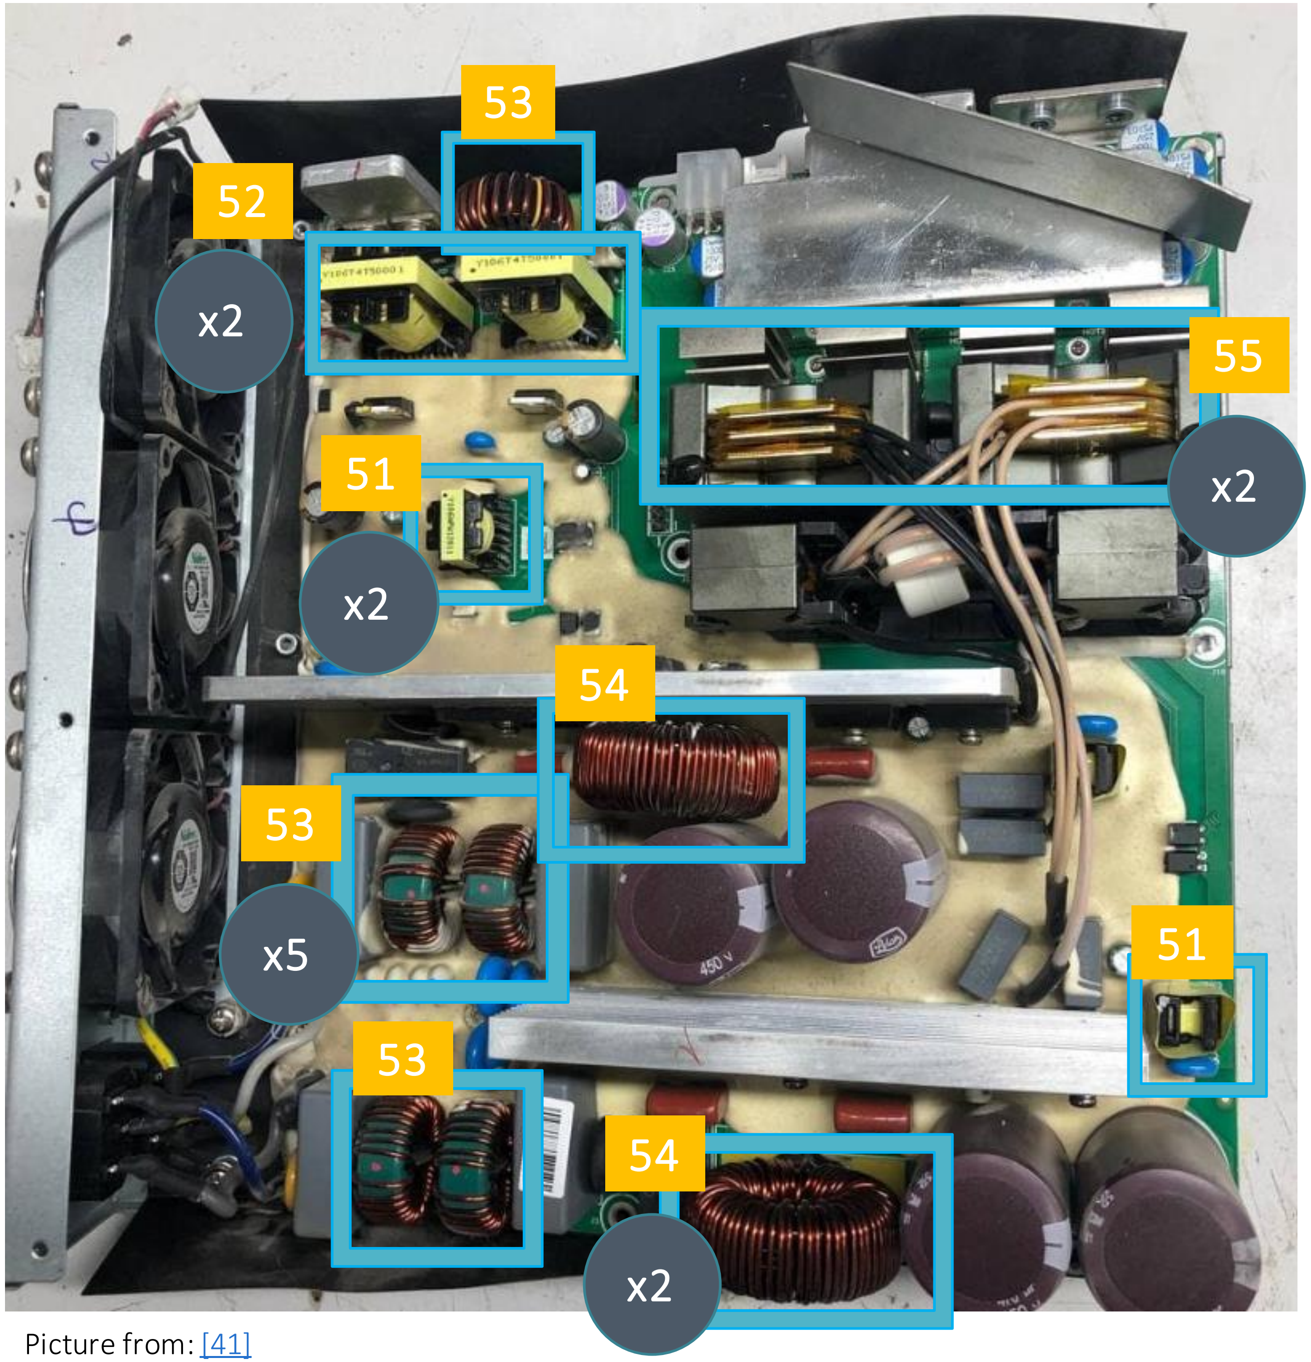


Picture from: [41]

# Power Supply

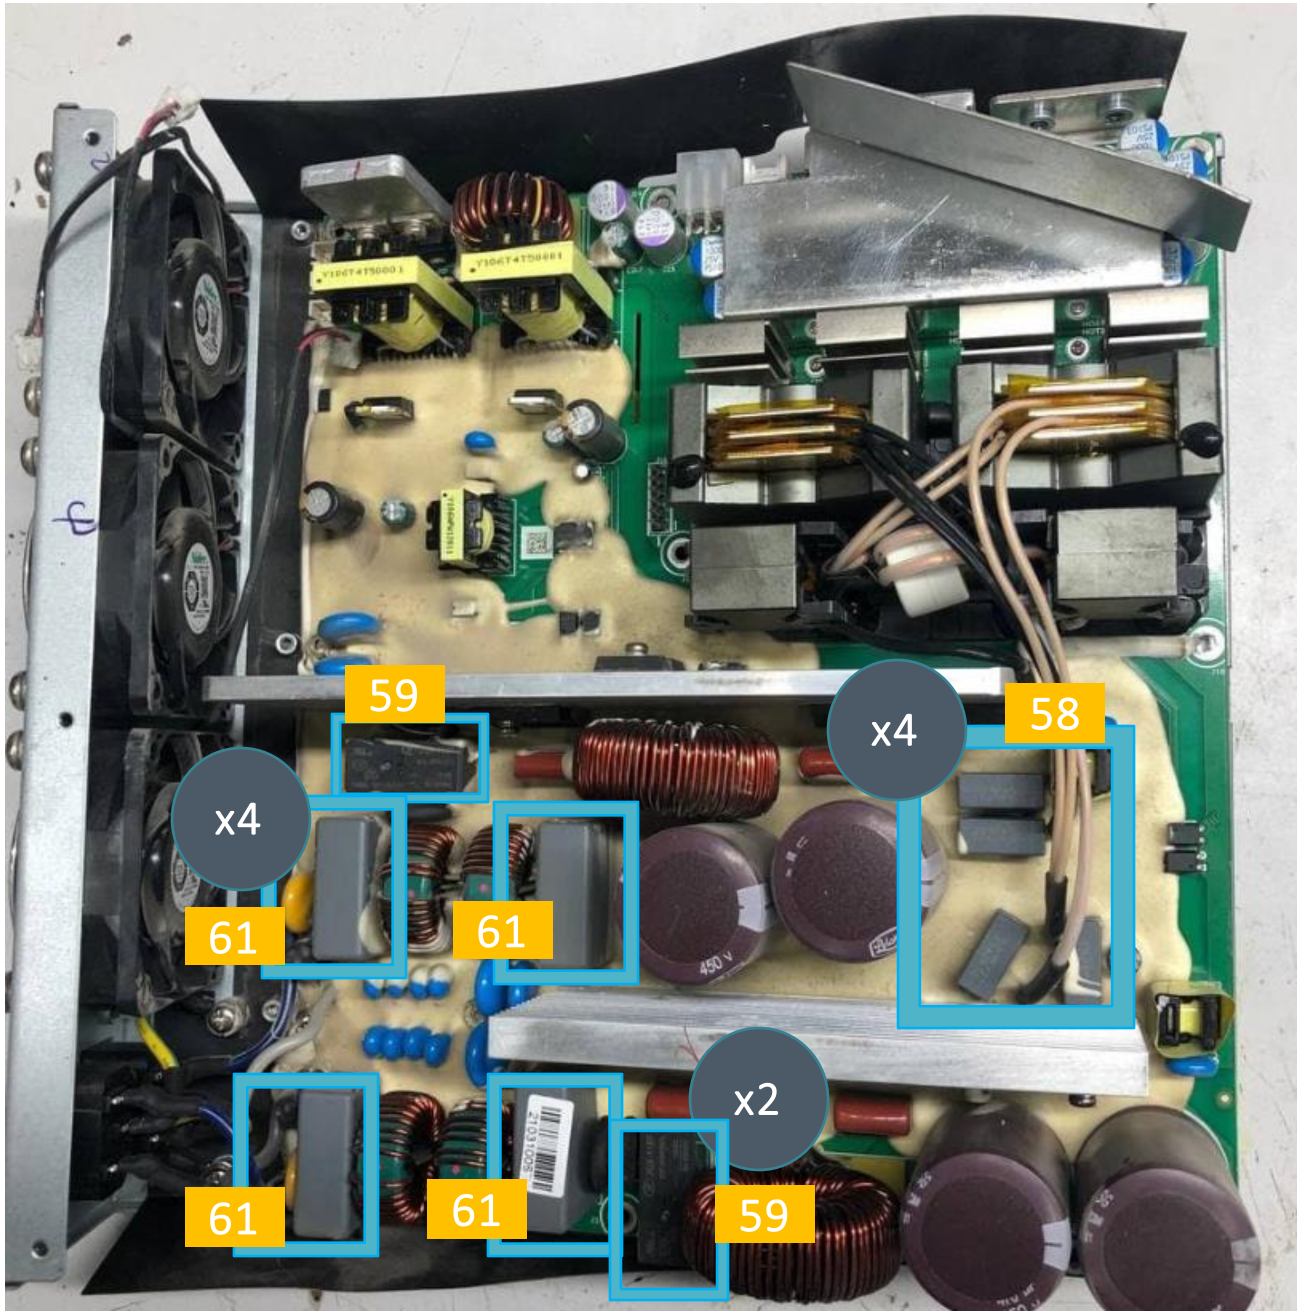


Picture from: [41]

# Power Supply: Fans and cables

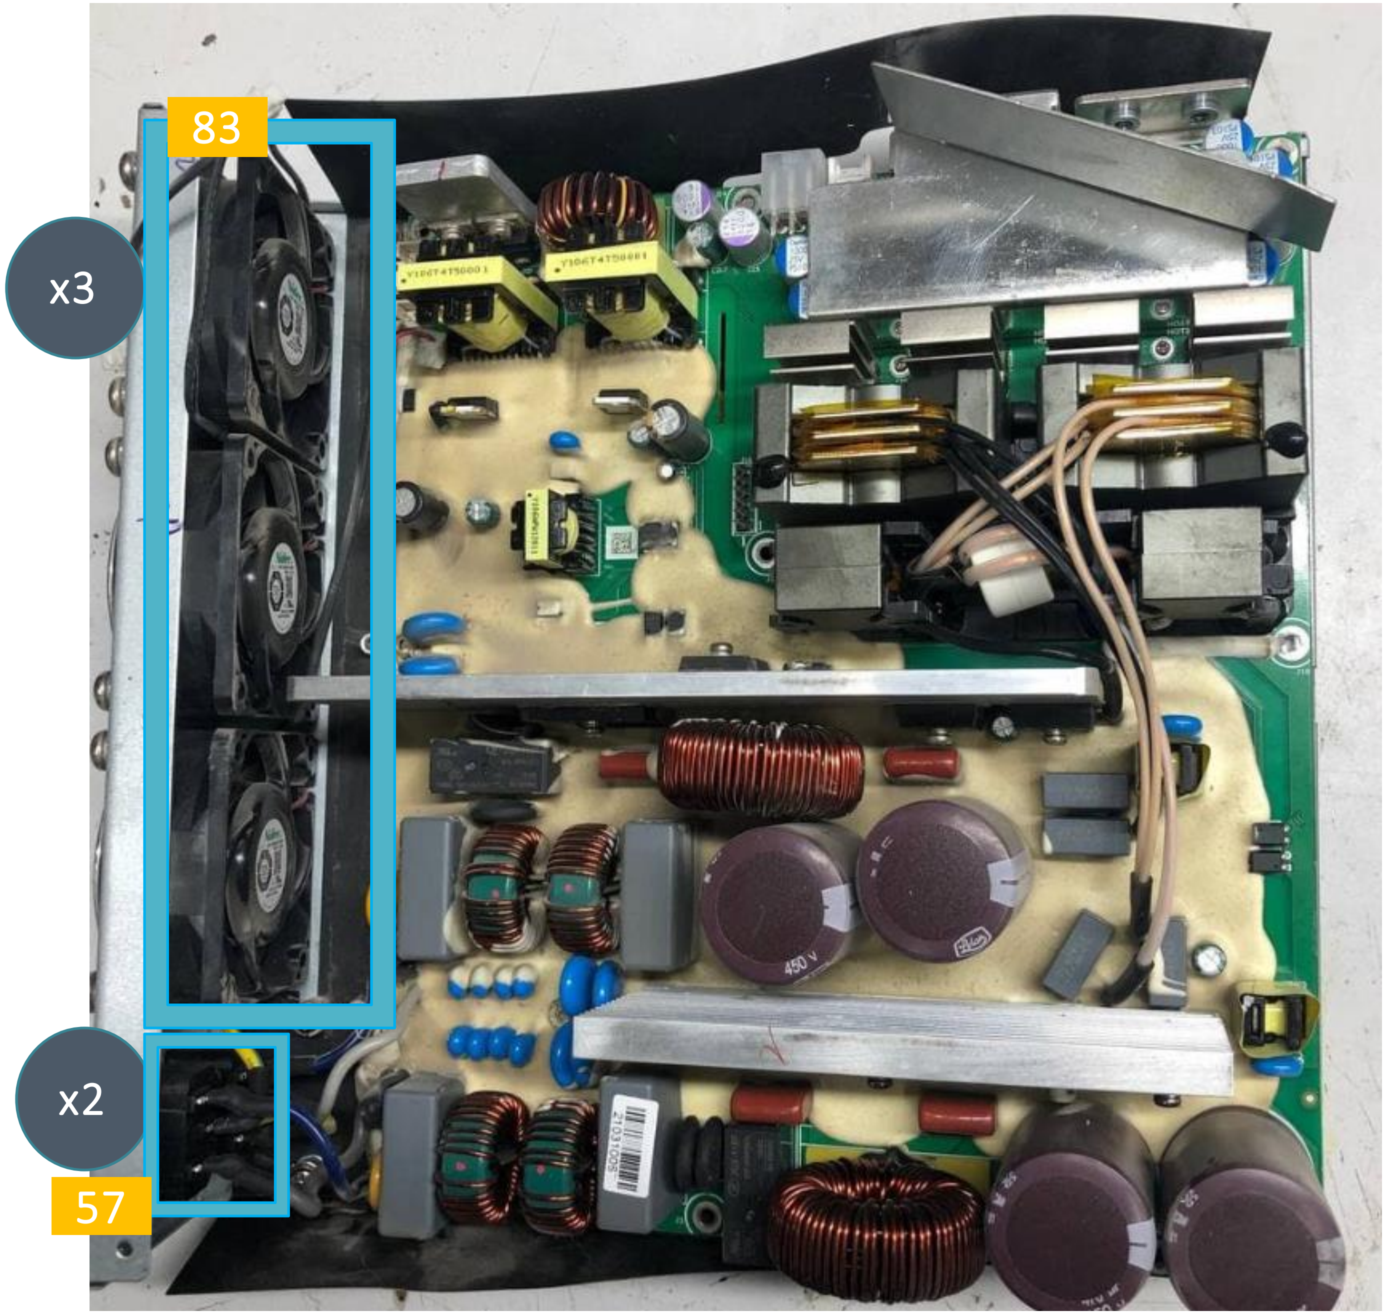


Picture from: [41]

# Additional Information

# Additional Information (ICs):

36

BM1387B

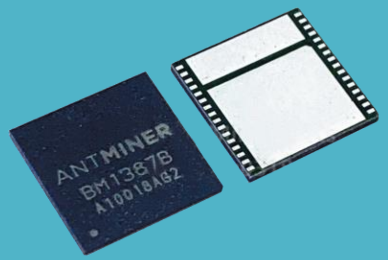


BGA, 16nm

[13], [14]

- Nb of PIN: 16 (edges)+56+1 (big at the center) = 73
- Area: 0,8 x 0,8 cm
- Package: BGA
- Nature of the chip: ASIC computing SHA-256
- Technology node: 16 nm

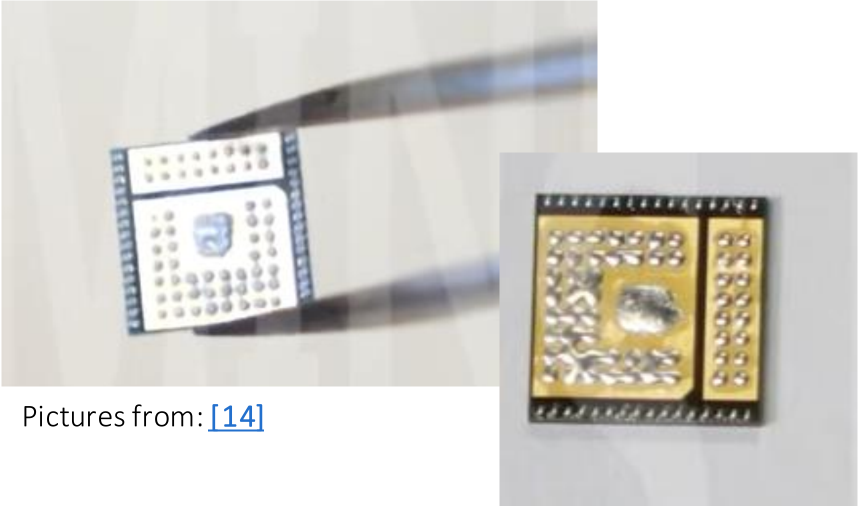

Pictures from: [14]

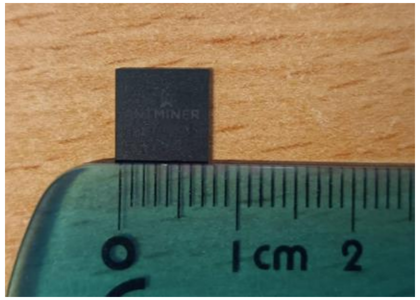


Picture from: Ludmila Courtillat--Piazza

Die after chemical removing of the package

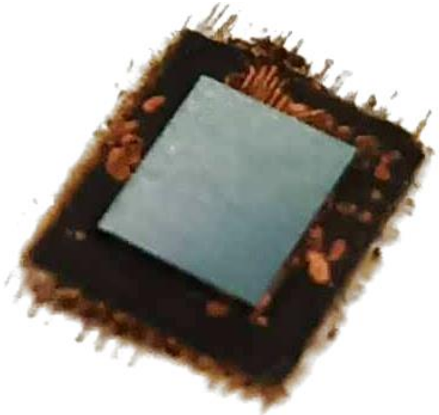

Picture from: Ludmila Courtillat--Piazza

Die after chemical removing of the package (microscope)

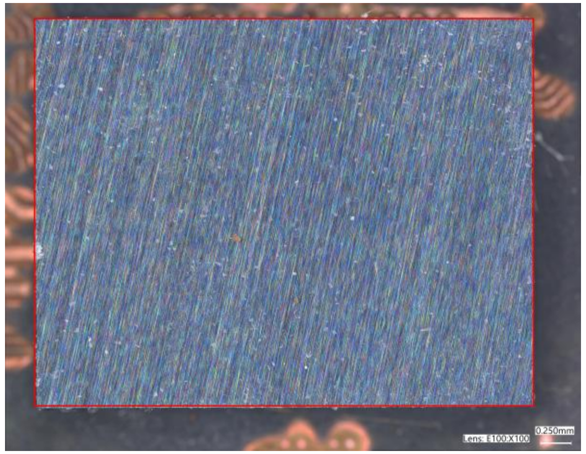

Picture from: Thibaut Heremans, Thibault Pirson, Ludmila Courtillat--Piazza

# Additional Information (ICs):

1

« XILINX / ZYNQ / XC7Z010 / CLG400ABX1809 / D5578954A / 1C /TAIWAN »

System on Chip Xilinx Zynq®-Z-7010 SoC

[1],
[42], [43]

- Nb of PIN: 400
- Number of I/Os: 130
- Package: BGA
- Nature of the chip: SoC
- Origine: Taiwan

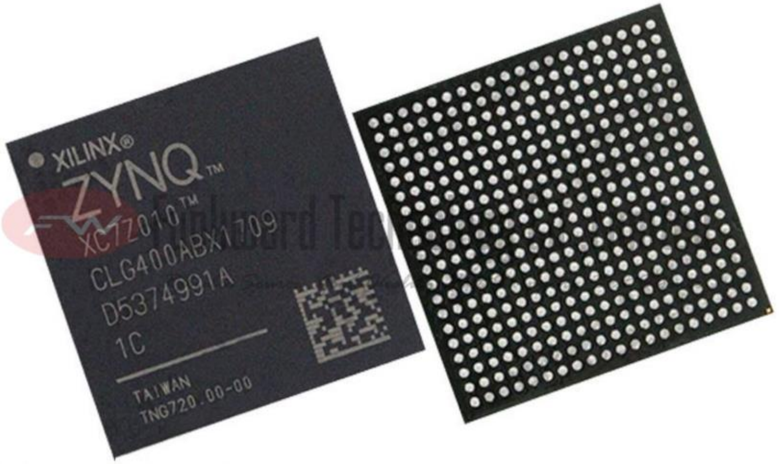


Picture from: [42]

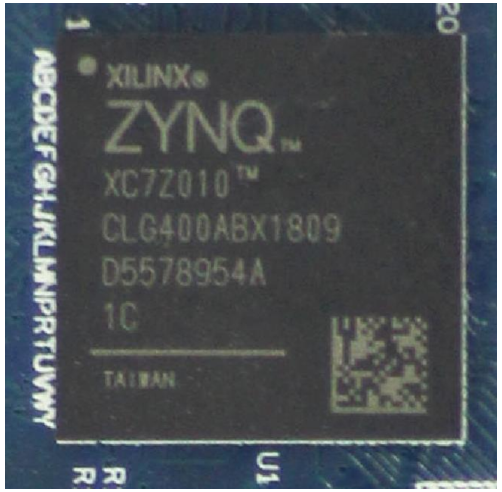


Picture from: [5]

Die after chemical removing of the package (microscope)

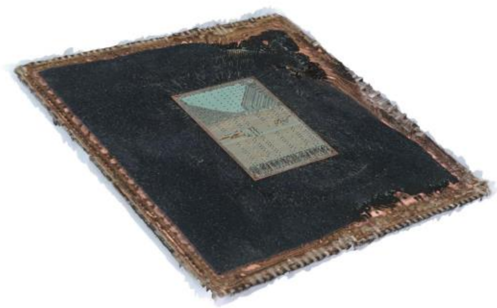

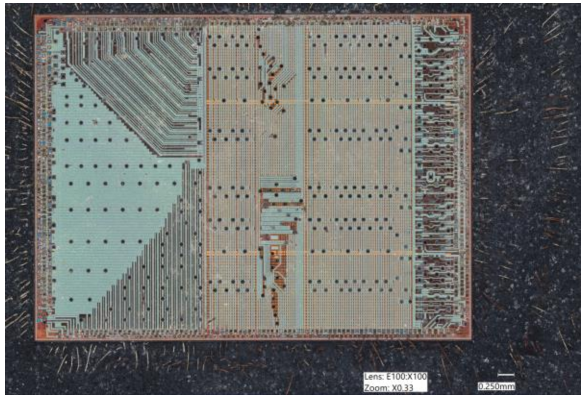

Pictures from: Thibaut Heremans, Thibault Pirson, Ludmila Courtillat--Piazza

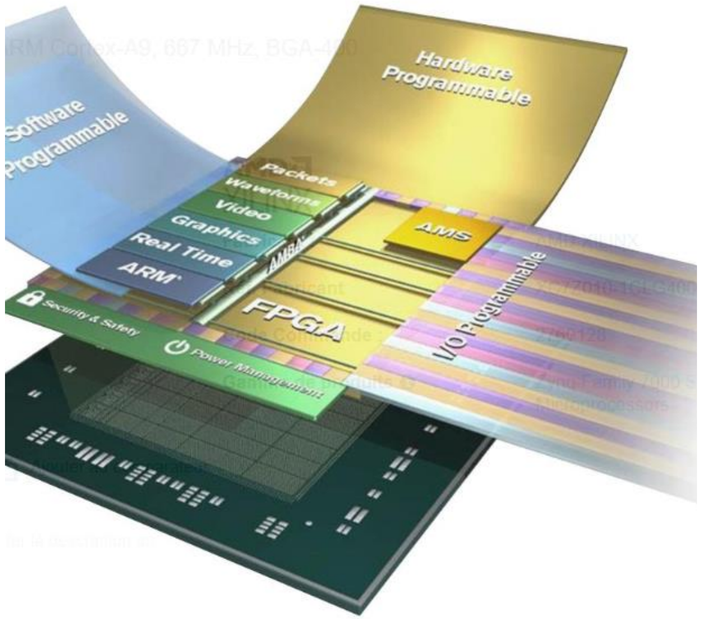


Picture from: [43]

# Additional Information(ICs):

2

« H5007NL YDL-1801C2 »

-> H500NL (Ethernet Transformer)

[2]

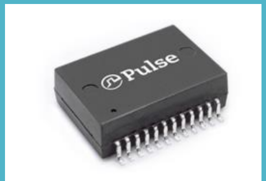

- Nb of PIN: 24
- Size: 17,53 x 12,2 (16,0) mm
- Package: SMT
- Nature of the chip: ETH transformer
- Function: Ethernet transformer

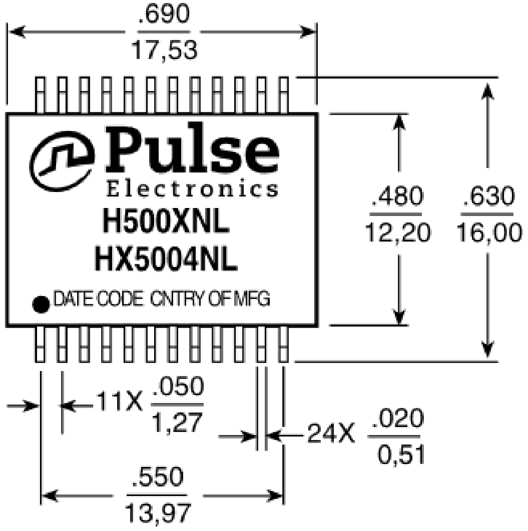


Picture from datasheet available on: [2]

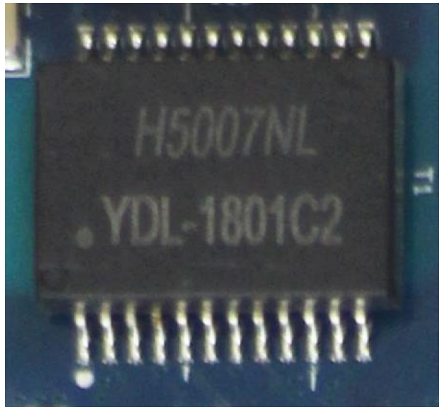


Picture from: [5]

« 7UK15 D9PTK + logo de Micron »

-> DRAM Micron MT41K128M16JT-125:k

[3], [4]

3

- Nb of PIN: 96
- Size: 8 x 13 mm
- Package: BGA
- Nature of the chip: DRAM
- Manufacturer: Micron

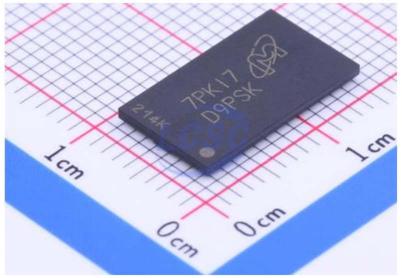


Picture from: [4]

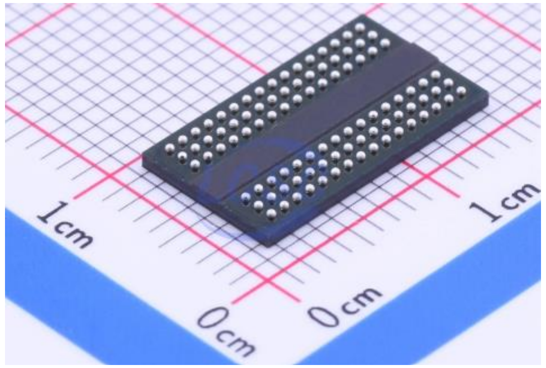


Picture from: [4]

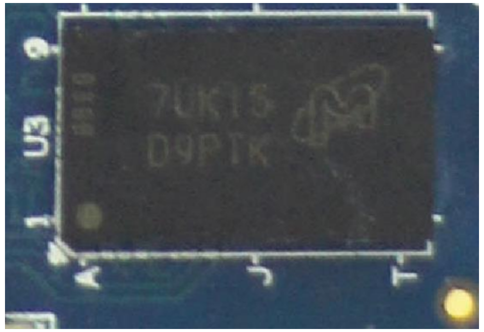


Picture from: [5]

# Additional Information (ICs):

Figure 5: 48-Pin TSOP – Type 1, CPL

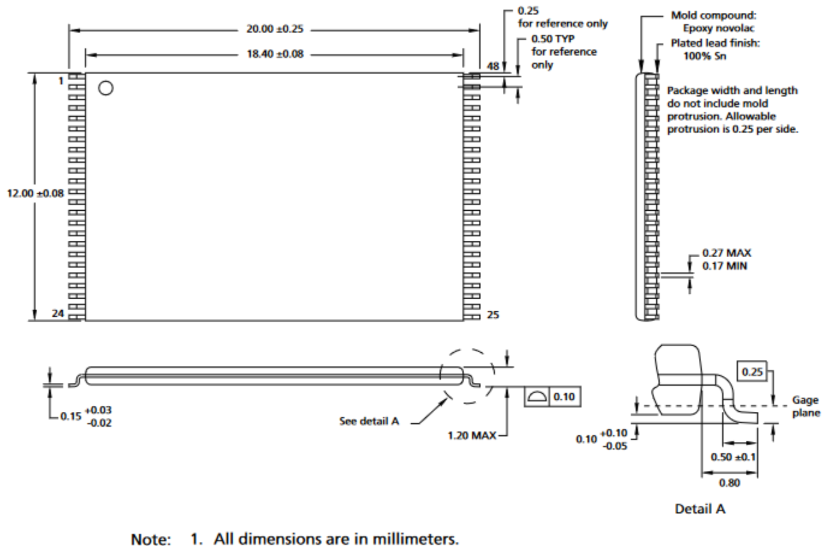


Picture from: [44]

4

« 1746 / I-D / logo micron / 29F2G08ABAEA / WP / E »

SLC NAND Flash

MT29F2G08ABAEA WP-IT:E TR

[7], [44], [45]

- Nb of PIN: 48
- Size: 12,0 0x 18,40 (20,00) mm
- Package: TSOP
- Origine: Malasya

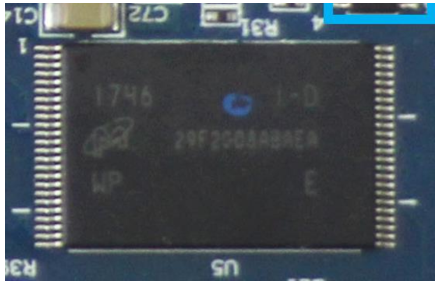

Picture from: [5]

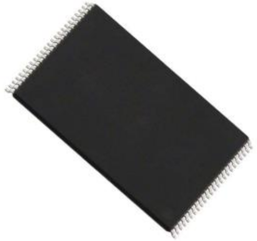

Picture from: [7]
(no longer available)

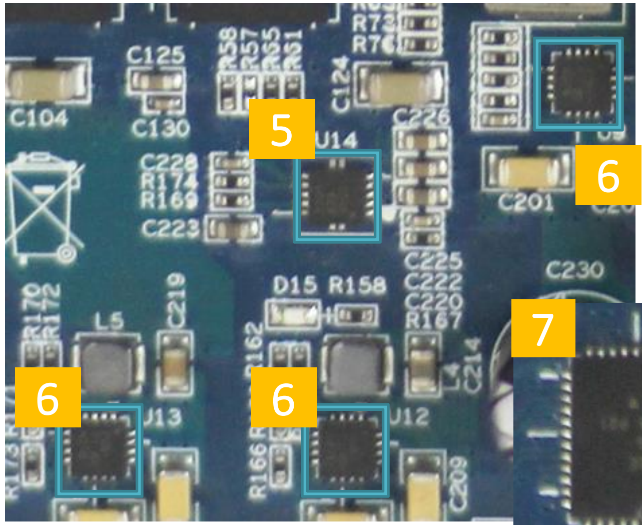


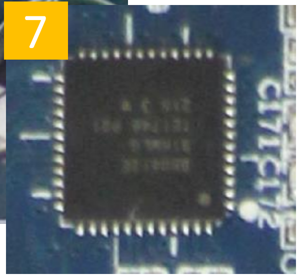


Picture from: [5]

5
- Nb of PIN: 14
- Size: 3 (4) x 3 (4) mm

6
- Nb of PIN: 16
- Size: 3 (4) x 3 (4) mm

7
- Nb of PIN: 48
- Size: 6,5 (7,5) x 6,5 (7,5) mm

IC, TQFP 32-100

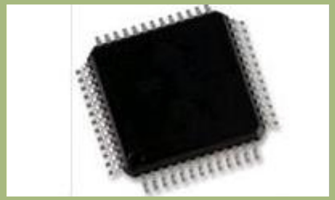

# Additional Information (ICs):

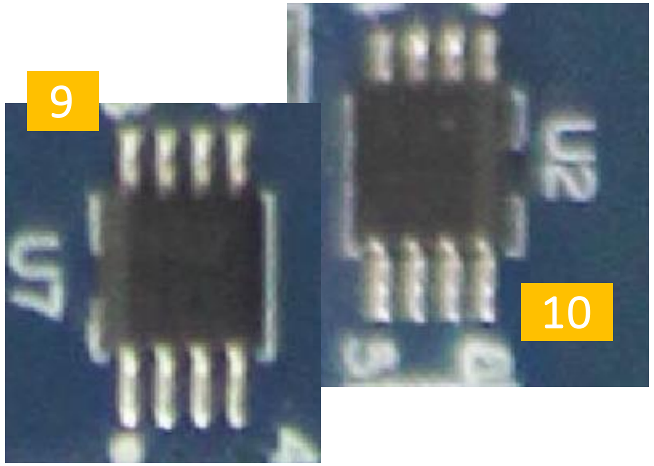


Pictures from: [5]

9, 10

- Nb of PIN: 8
- Size: 3 (5) x 2,5 mm
- function: programmer la board

IC, SO 8-44

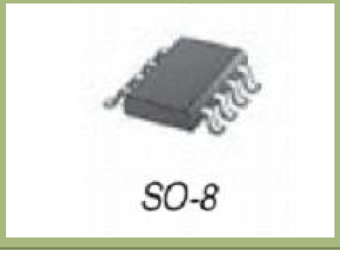


37

« 61P8K6J / 27402S »

Switching controller LM27402S

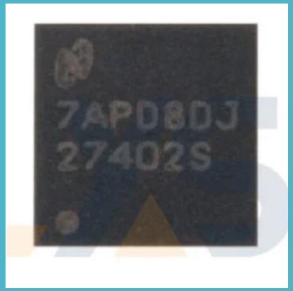


[16], [17]

- Nb of PIN: 16
- Size: 16 mm² 4 x 4
- Size of thermal pad: 2,6 x 2,6 -+ 1 mm²
- Package: WQFN-16
- Nature du chip: controller
- Function: Switching controller

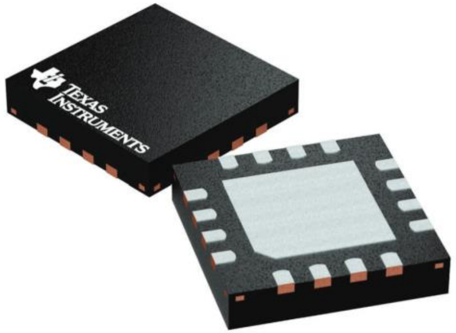


Pictures from: [17]

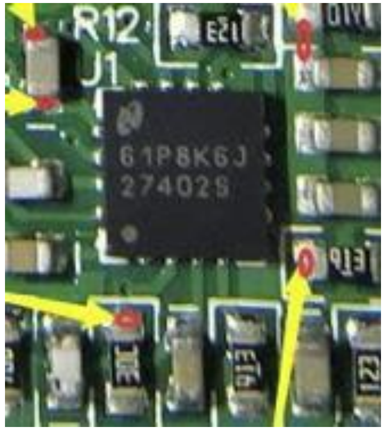


Pictures from: [16]

# Additional Information (ICs):

«PIC16F1704 / -V SL 'symbole' / 'symbole' 1612B17 »

38

**Microcontroller**

PIC16F1704-I/SL

MCU 8-bit PIC RISC 7KB Flash 3.3V/5V Automotive 14-Pin SOIC N Tube

[18]

- Nb of PIN: 14
- Number of IO: 12
- Size: 8,65 x 3,9 mm
- Package: SOIC-14
- Nature du chip: MCU
- Manufacturer: Microchip
- Date of release: 2018-12-07

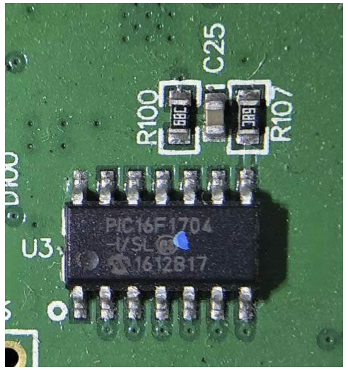


Picture from: [6]

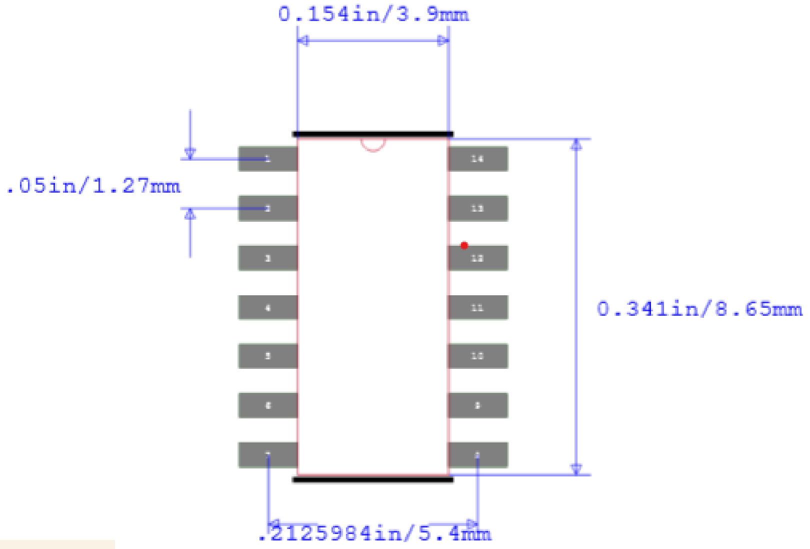


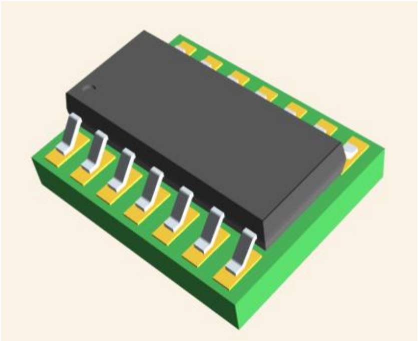

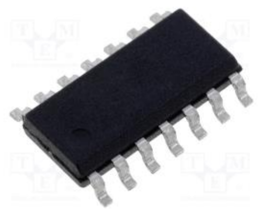

Pictures from: [18] (no longer available without login)

# Additional Information

Remark: several versions of similar heat sinks are used. As illustrated by this picture, the heat sinks on both sides of the hashboards are not the same.

35

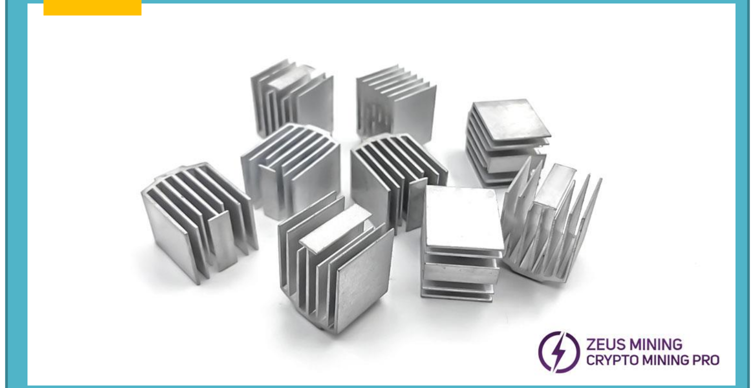


[11], [12]

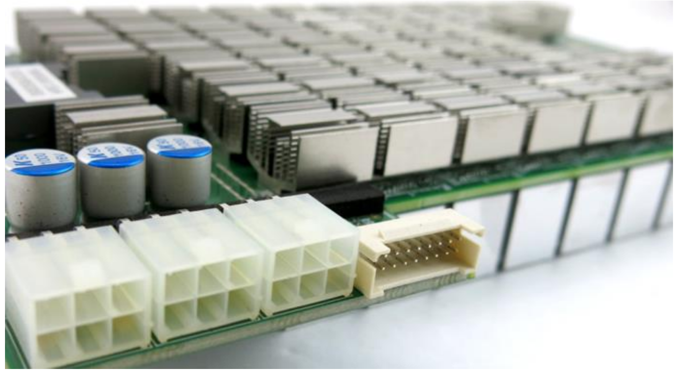

Picture from: [47]

43

« TPHR90 / 03NL / 5:42 »

TPHR9003NL

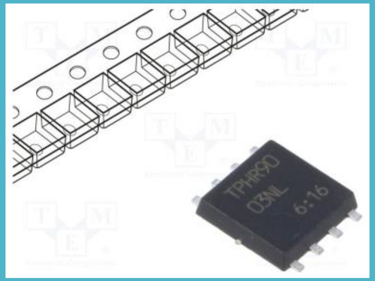


[46], [48]

Area: 5 x 5mm
Nb of PINs: 8
Mass: 0.069 g
Manufacturer: Toshiba
Package: SOP

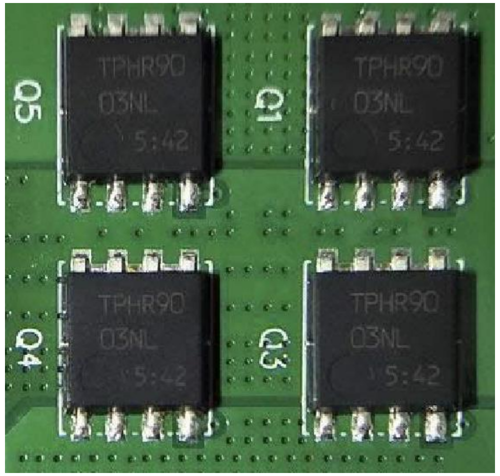


Picture from: [6]

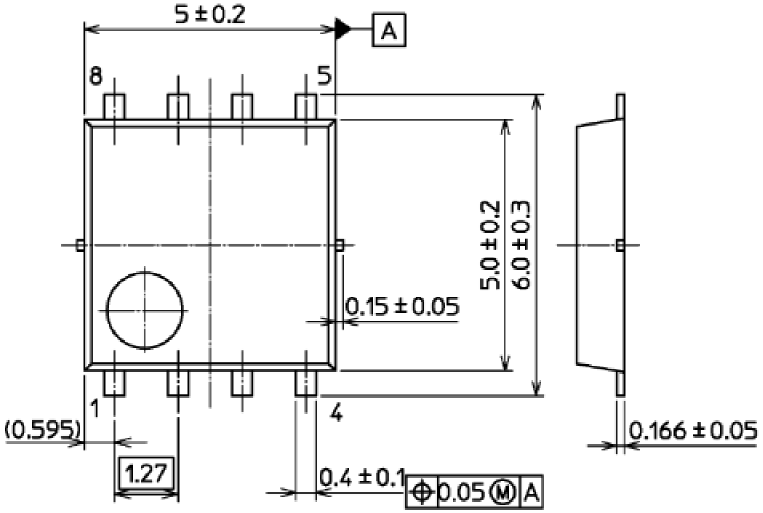


Picture from: [48]

# Additional Information:

44

« 1AM »

SOT-23 MMBT3904

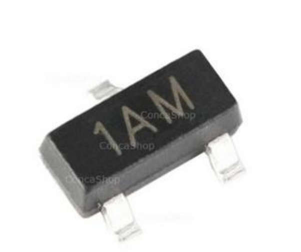


[19]

- Area: 1,3 x 2,9 mm
- Nb of PINs: 3

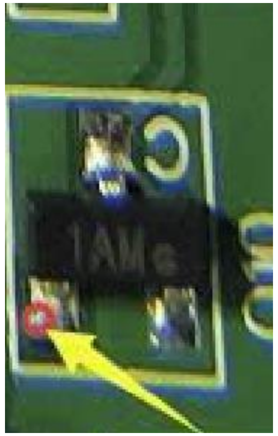


Picture from: [6]

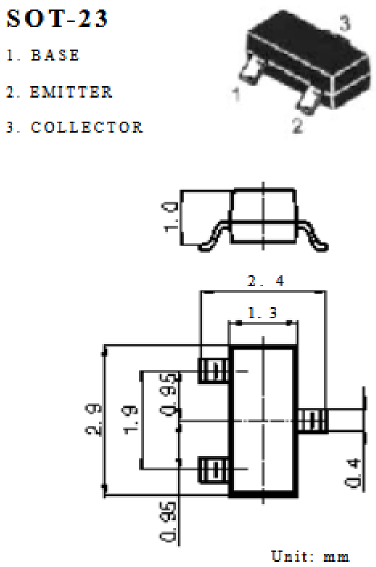


Picture from: [19]

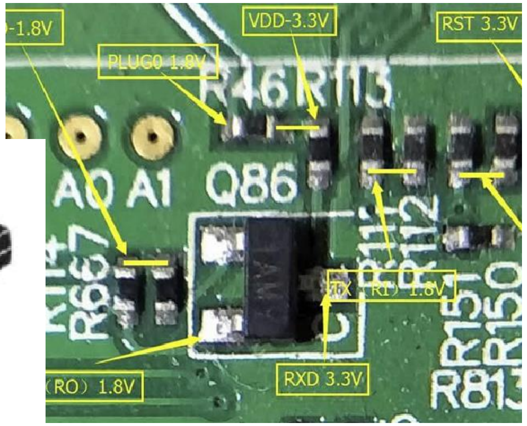


Picture from: [6]

Transistor signal SOT23 3 leads

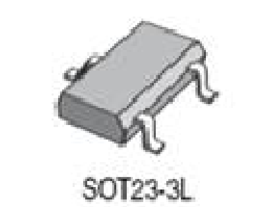


45

« KDDCI40A/1.5UH / Y0331R503050 »

Y0331R503050 1.5UH power inductor

[20]

- Area: (estimated) 30 x 31 mm

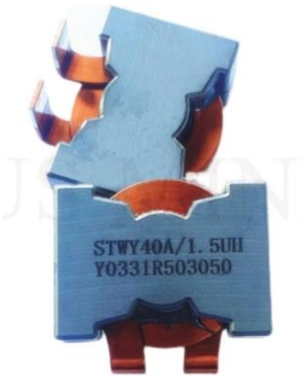


Picture from: [20]

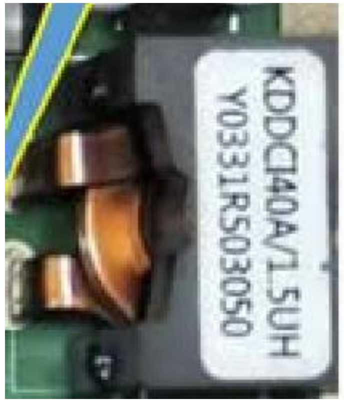


Picture from: [6]

Ring core coils 8, 30, 80g (with housing)

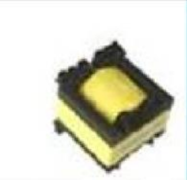

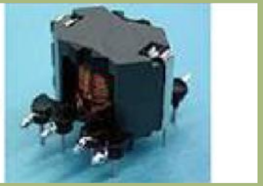

# Additional Information:

48

« 450v470 »

Electrolitic capacitor

Nichicon 470µF Aluminium Electrolytic Capacitor 450V dc, Snap-In - LGU2W471MELC

[23], [24]

- Area: (estimated) 35 (Dia.) x 50mm

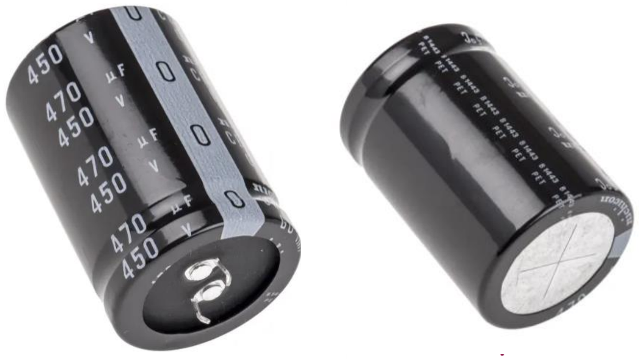

Pictures from: [23]

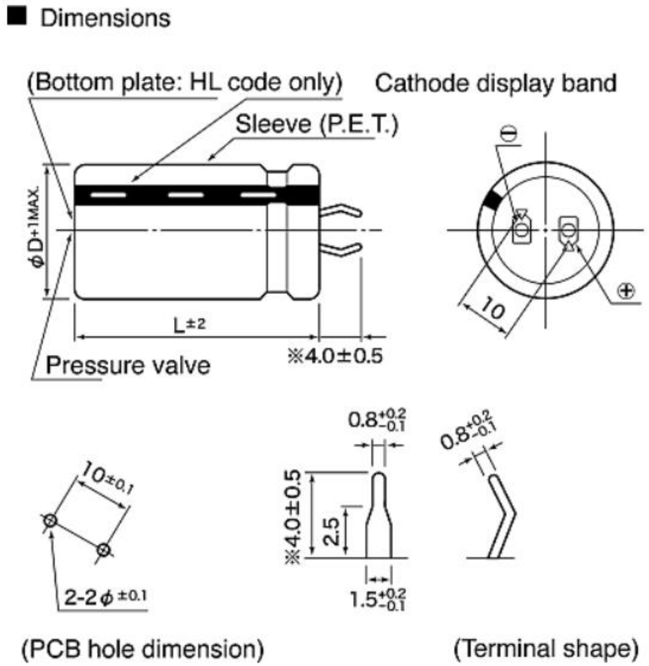


Pictures from: [24]

# Sources:


[1] https://www.digikey.be/en/product-highlight/t/trenz/te0723-arduzynq-series-with-xilinx-zynq-z-7010-z-7007s-soc?utm_adgroup=General&utm_source=google&utm_medium=cpc&utm_campaign=Dynamic%20Search_EN_RLSA_Product_Cart&utm_term=&productid=&gclid=EAIaIQobChMIr6eK3ZPP_QIV0vd3Ch2X1QQREAAYASAAEgIEgPD_BwE

[2] https://productfinder.pulseeng.com/product/H5007NL

[3] https://www.micron.com/products/dram/ddr3-sdram/part-catalog/mt41k128m16jt-125

[4] https://www.lcsc.com/product-detail/DDR-SDRAM_Micron-Tech-MT41K128M16JT-125-k_C36513.html

[5] https://support.bitmain.com/hc/en-us/articles/360019493654-S9-series-S9-S9i-S9j-S9-Hydro-Control-Board-Program-Recovery

[6] https://www.zeusbtc.com/manuals/Antminer-S9-Hash-Board-Repair-Guide.asp

[7] https://octopart.com/mt29f2g08abaeawp-it%3Ae+tr-micron-20494102?gclid=EAIaIQobChMIhOS9ms3Y_QIVc-TmCh3BagCjEAAYASAAEgKW9_D_BwE

[8] https://botland.store/tht-electrolytic-capacitors/16730-electrolytic-capacitor-4700uf25v-16x25mm-105c-tht-5pcs-5904422378264.html

# Sources:


[9] https://www.zeusbtc.com/manuals/user-manuals/AntMiner-S9-Installation-Guide.pdf

[10] https://www.ebay.com/itm/Antminer-S9-Spower-Hashboard-63-V1-95-Submodel-S9-12-93-/362981698322?_ul=BR

[11] https://www.zeusbtc.com/ASIC-Miner-Repair/Parts-Tools-Details.asp?ID=289

[12] https://www.zeusbtc.com/ASIC-Miner-Repair/Parts-Tools-Details.asp?ID=1158

[13] https://www.zeusbtc.com/ASIC-Miner-Repair/Parts-Tools-Details.asp?ID=58

[14] https://www.youtube.com/watch?v=5WH7g61d90w

[15] https://www.antminerdistribution.com/antminer-s9/s9-hash-board/

https://miningwholesale.eu/product/bitmain-antminer-s9i-hashboard/

[16] https://lys-sz.com/products/lm27402s-lm27402sq-nopb-switching-controller-high-performance-synchronous-buck-27402s-for-antminer

[17] https://www.ti.com/product/LM27402?utm_source=google&utm_medium=cpc&utm_campaign=app-bsr-null-prodfolderdynamic-cpc-pf-google-wwe_int&utm_content=prodfolddynamic&ds_k=DYNAMIC+SEARCH+ADS&DCM=yes&gclid=EAIaIQobChMIs_qPmaXb_QIVGMjVCh0BQwmNEAAYASAAEgJ0dvD_BwE&gclsrc=aw.ds#descriptio

# Sources:


[18] https://html.alldatasheet.com/html-pdf/140113/AVICTEK/1AM/290/1/1AM.html

[19] https://octopart.com/tphr9003nl-toshiba-52058653?gclid=EAIaIQobChMI8qjUxZ3Z_QIVQIxoCR3Inw5ZEAAYASAAEgKWd_D_BwE

[20] https://www.zeusbtc.com/ASIC-Miner-Repair/Parts-Tools-Details.asp?ID=2431

[21] https://www.antminerdistribution.com/apw3/

[22] https://www.youtube.com/watch?v=KYS1yTZv1Xs&t=1164s

[23] https://benl.rs-online.com/web/p/aluminium-capacitors/4909406?cm_mmc=BE-PLA-DS3A-_-google-_-CSS_BE_NL_Passive_Components_Whoop-_-(BE:Whoop!)+Aluminium+Capacitors-_-4909406&matchtype=&pla-340045680949&gclid=Cj0KCQjwuLShBhC_ARIsAFod4fIacAU1P76pbOiM8dLG3_NK-5HSMqHqXDFLbq1KjGpJ_6Aa8ELBzNkaAontEALw_wcB&gclsrc=aw.ds

[24] https://docs.rs-online.com/8d8e/0900766b80634fdb.pdf

[25] https://fr.aliexpress.com/item/1005003092048920.html?gatewayAdapt=glo2fra

[26] https://www.zeusbtc.com/ASIC-Miner-Repair/Parts-Tools-Details.asp?ID=1967

[27] https://www.alibaba.com/product-detail/6025-6cm-DC12V-0-27A-APW3_62326692063.html

# Sources:


[28] https://bitcointalk.org/index.php?topic=4553538.0

[29] https://www.youtube.com/watch?v=4cJo5qBBkkI&t=380s

[30] https://www.zeusbtc.com/ASIC-Miner-Repair/Parts-Tools-Details.asp?ID=2541

[31] https://www.zeusbtc.com/ASIC-Miner-Repair/Parts-Tools-Details.asp?ID=1283

[32] https://en.wikipedia.org/wiki/Linear_low-density_polyethylene

[33] https://www.zeusbtc.com/ASIC-Miner-Repair/Parts-Tools-Details.asp?ID=2870

[34] https://support.bitmain.com/hc/en-us/articles/360018041153-Choose-the-correct-power-cord-for-your-miner

[35] https://www.zeusbtc.com/ASIC-Miner-Repair/Parts-Tools-Details.asp?ID=2576

[36] https://www.zeusbtc.com/ASIC-Miner-Repair/Parts-Tools-Details.asp?ID=70

[37] https://ru.zeusbtc.com/ASIC-Miner-Repair/Parts-Tools-Details.asp?ID=78

[38] https://www.youtube.com/watch?v=qAdhTWS0ujk

[39] https://www.zeusbtc.com/manuals/Antminer-S19-Pro-Hash-Board-Repair-Guide.asp

[40] https://www.ebay.com/itm/354080014467

[41] https://asicdip.com/files/Bitmain_APW_12_modifications_en.pdf

# Sources:


[42] https://www.ebay.com/itm/163782006818

[43] https://be.farnell.com/fr-BE/xilinx/xc7z010-1clg400c/psoc-arm-cortex-a9-667mhz-bga/dp/2760128

[44] https://4donline.ihs.com/images/VipMasterIC/IC/MICT/MICTS03967/MICTS03967-1.pdf?hkey=52A5661711E402568146F3353EA87419

[45] https://www.avnet.com/shop/us/products/micron/mt29f2g08abaeawp-it%3Ae-tr-3074457345626790348?CMP=EMA_Octopart_inventoryfeed_VSE

[46] https://octopart.com/tphr9003nl-toshiba-52058653?gclid=EAIaIQobChMI8qjUxZ3Z_QIVQIxoCR3Inw5ZEAAYASAAEgKWd_D_BwE

[47] https://www.parallelminer.com/product/bitmain-antminer-s9-hash-board-replacement-bm1387-16nm-63-chips/

[48] https://datasheet.octopart.com/TPHR9003NL-Toshiba-datasheet-86281461.pdf

[49] https://miningwholesale.eu/product/bitmain-antminer-s9-hashboard/

[50] https://www.ginifab.com/feeds/cm_to_inch/virtual_ruler_on_your_image.html

[51] https://www.datasheetcafe.com/tvr14471-pdf-21901/

[52] https://www.amazon.com/20PCS-TVR14471-varistor-14d471k-Authentic/dp/B08F4RKZKS

# Sources:


[53] https://www.aliexpress.com/i/33011524141.html?gatewayAdapt=glo2fra

[54] https://www.vishay.com/docs/22204/wko.pdf

[55] https://www.zeusbtc.com/ASIC-Miner-Repair/Parts-Tools-Details.asp?ID=61

[56] https://www.zeusbtc.com/ASIC-Miner-Repair/Parts-Tools-Details.asp?ID=46

[57] https://www.zeusbtc.com/manuals/user-manuals/AntMiner-S19-Pro-manual.pdf

[58] https://www.cynel.com.pl/en/products/103-sn96-5ag3cu0-5-sac305)

[59] https://www.belfuse.com/resources/ApplicationNotes/PowerSolutions/app-note-BPS-Non-Isolated-DC-DC-Converter-Eutectic-Solder-Process.pdf

[60] https://www.amazon.com/Bitmain-Fan-AntMiner-S9-T9/dp/B01N4BQZ27

[61] https://www.zeusbtc.com/ASIC-Miner-Repair/Parts-Tools-Details.asp?ID=46

[62] https://www.parallelminer.com/product/bitmain-antminer-s9k-6100-rpm-high-performance-fan-260cfm-2-8a-12v-120mm-x-38mm/

[63] https://fr.aliexpress.com/item/1005004019236116.html?gatewayAdapt=glo2fra
